# Supplementary material for: Training Generative Image Super-Resolution Models by Wavelet-Domain Losses Enables Better Control of Artifacts
Source: arXiv:2402.19215 source file (2024-02-29)
Supplement: Supplementary file 1 [file X_suppl.tex]

\clearpage
\maketitlesupplementary

\section{Further Visual Comparison of SISR}

We provide further visual comparisons of 4$\times$ SISR between our proposed method WGSR and the other state-of-the-art methods including ESRGAN-FS \cite{freq_sep}, ESRGAN+ \cite{esrganplus}, RankSRGAN \cite{zhang2021ranksrgan}, SPSR \cite{ma_SPSR}, SRFlow-DA \cite{jo2021srflowda}, LDL \cite{details_or_artifacts}, FxSR \cite{fxsr}, PDASR \cite{PDASR}, SROOE \cite{srooe_Park_2023_CVPR} and DualFormer \cite{dualformer_luo2023effectiveness} in Fig. \ref{fig:supp_div2k1} to Fig. \ref{fig:supp_urban2}. From these visual comparisons, one can draw consistent observations in line with the results in the paper. Our proposed method WGSR not only suppresses visual artifacts but also simultaneously restores structural shapes and realistic details.

\section{Perception-Distortion Trade-off}
Fig. \ref{fig:pd_urban_div2k} provides perception-distortion points for our WGSR and other state-of-the-art methods on PSNR-NRQM plane for Set14 \cite{set14_cite}, Urban100 \cite{urban100_cite} and DIV2K \cite{Agustsson_2017_CVPR_Workshops} validation datasets. Our proposed method, WGSR, significantly improves fidelity and perceptual scores across all datasets, resulting in a better PD trade-off point. Specifically, WGSR achieves the highest NRQM \cite{Ma_NRQM} scores on Urban100 and DIV2K datasets when compared to other methods with comparable PSNR scores. This also validates the generalization performance of the proposed WGSR to different benchmarks.

\section{Further Visual Comparison of Different Wavelet Filters}

The visual comparison of proposed WGSR method with different wavelet families \cite{wavelet_doc} for 4$\times$ SISR is shown in Fig. \ref{fig:supp_wavelet_fam_visual}. We observe that visual performance varies according to the choice of wavelet family and the results show that the best perception-distortion trade-off point is achieved by the Symlet “sym7” filter. However, all wavelet filters notably mitigate artifacts while providing photo-realistic SR results.  

\begin{figure}
\centering
\begin{subfigure}{0.47\textwidth} 
     \begin{subfigure}{\textwidth}
        \includegraphics[width=\textwidth]{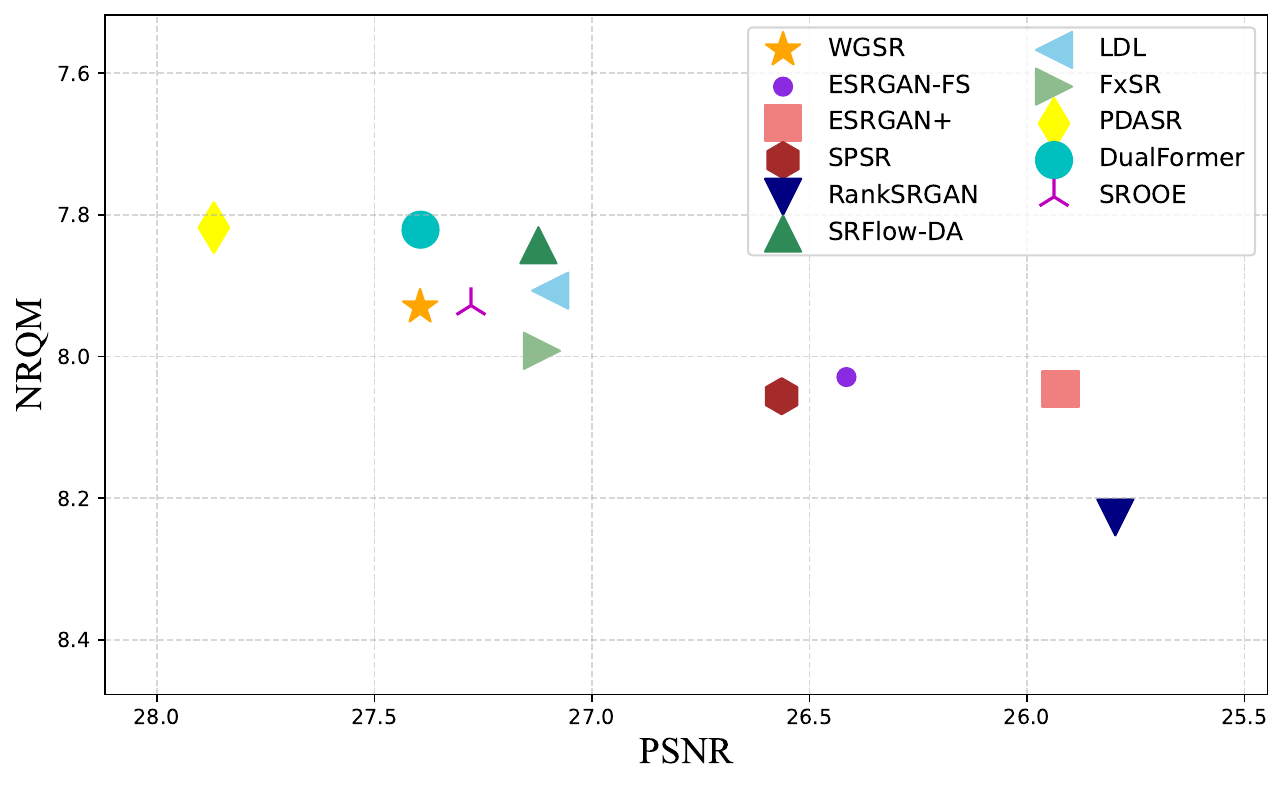} 
    \end{subfigure} 
    \caption{Set14 \cite{set14_cite}}
    \vspace{10pt}
     \begin{subfigure}{\textwidth}
        \includegraphics[width=\textwidth]{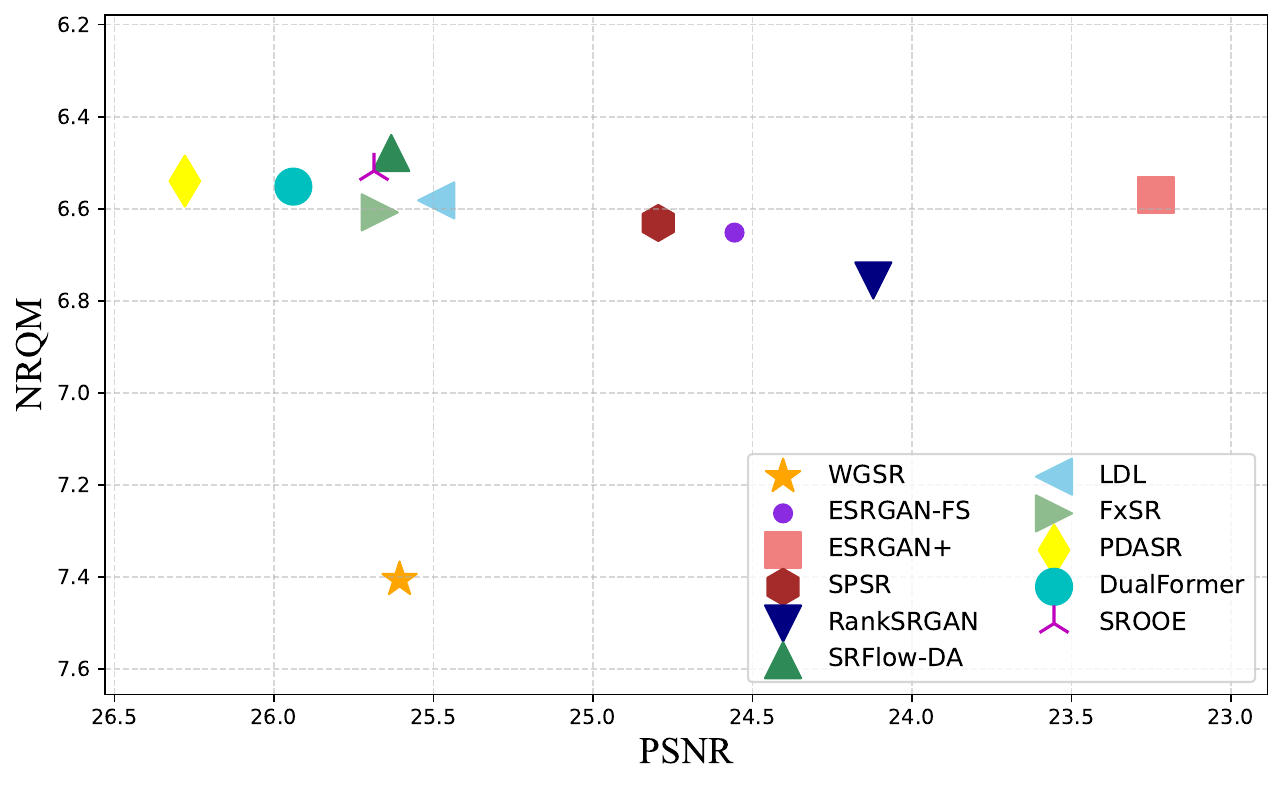} 
    \end{subfigure} 
    \caption{Urban100 \cite{urban100_cite}}
    \vspace{10pt}
    \begin{subfigure}{\textwidth}
        \includegraphics[width=\textwidth]{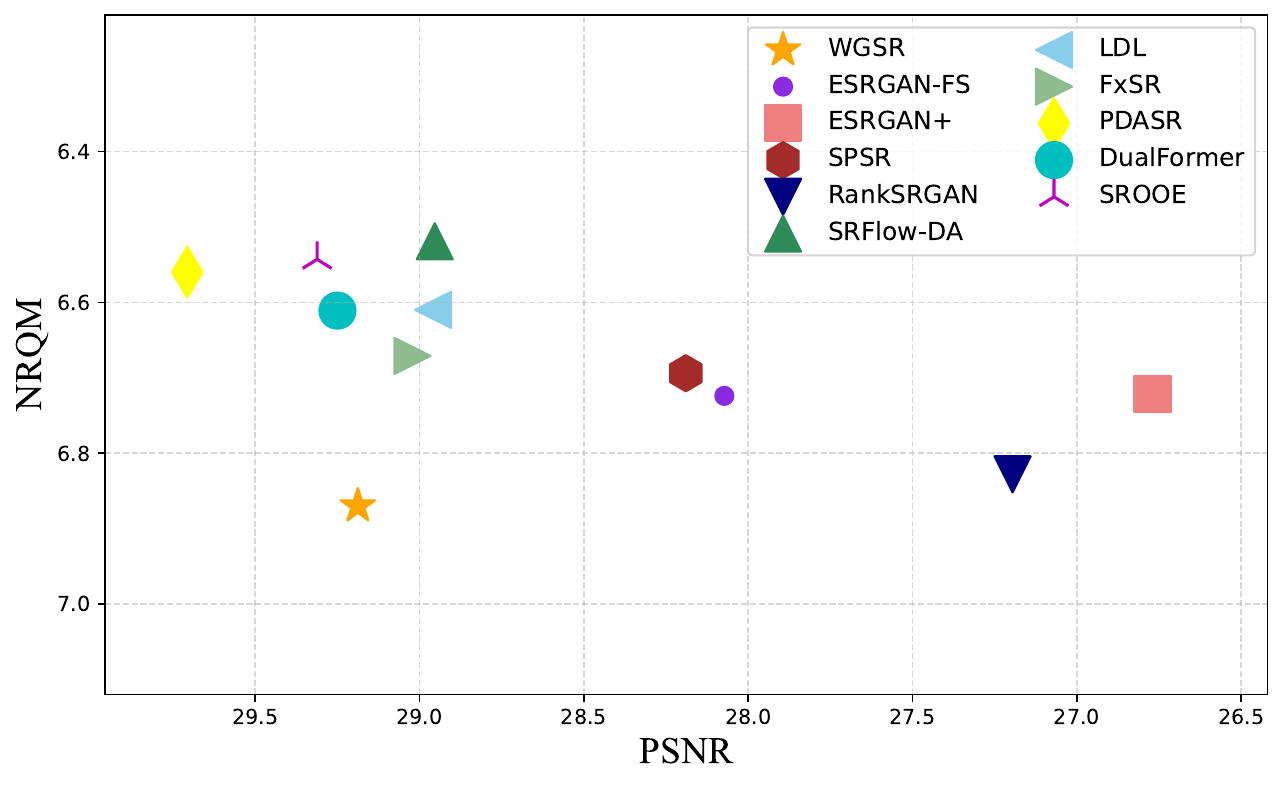} 
    \end{subfigure}
    \caption{DIV2K \cite{Agustsson_2017_CVPR_Workshops}}
    \vspace{10pt}
\end{subfigure}
\caption{Perception-distortion trade-off performance of our model WGSR compared to other state-of-the-art methods on the PSNR-NRQM plane.}
\label{fig:pd_urban_div2k} 
\end{figure}

\begin{figure*}
\centering
\begin{subfigure}{0.16\textwidth}
     \begin{subfigure}{\textwidth}
        \includegraphics[width=\textwidth]{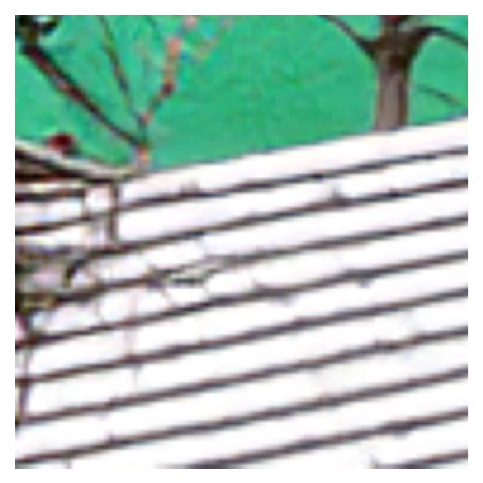} \\ \small ESRGAN-FS \cite{freq_sep} \\ (18.20 / 0.216)
    \end{subfigure}
    \begin{subfigure}{\textwidth}
        \includegraphics[width=\textwidth]{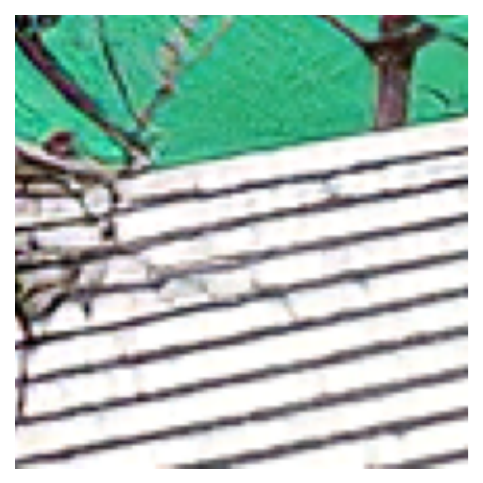} \\ \small ESRGAN+ \cite{esrganplus} \\ (17.83 / 0.187)
    \end{subfigure}
     \begin{subfigure}{\textwidth}
        \includegraphics[width=\textwidth]{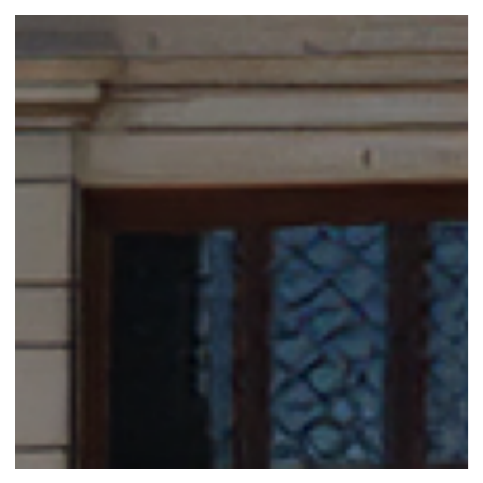} \\ \small ESRGAN-FS \cite{freq_sep} \\ (29.56 / 0.169)
    \end{subfigure}
    \begin{subfigure}{\textwidth}
        \includegraphics[width=\textwidth]{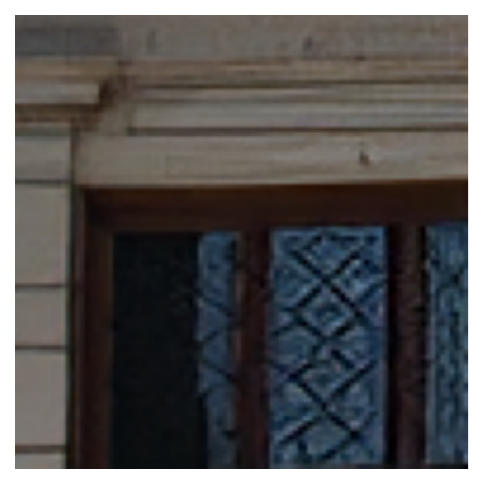} \\ \small ESRGAN+ \cite{esrganplus} \\ (26.33 / 0.191)
    \end{subfigure}
     \begin{subfigure}{\textwidth}
        \includegraphics[width=\textwidth]{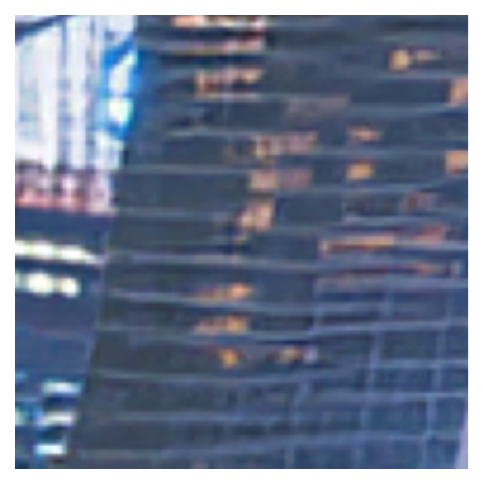} \\ \small ESRGAN-FS \cite{freq_sep} \\ (22.88 / 0.203)
    \end{subfigure}
    \begin{subfigure}{\textwidth}
        \includegraphics[width=\textwidth]{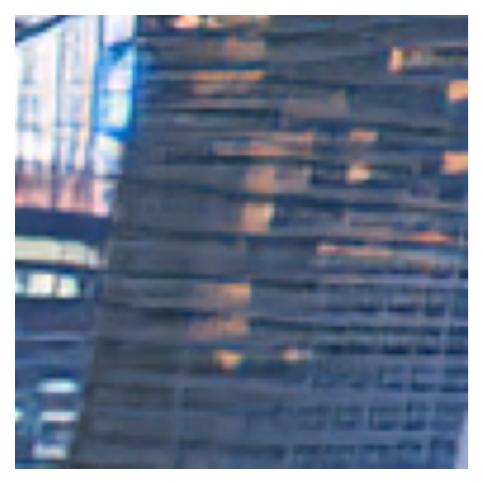} \\ \small ESRGAN+ \cite{esrganplus} \\ (22.49 / 0.218)
    \end{subfigure}
\end{subfigure}
\begin{subfigure}{0.16\textwidth}
    \begin{subfigure}{\textwidth}
        \includegraphics[width=\textwidth]{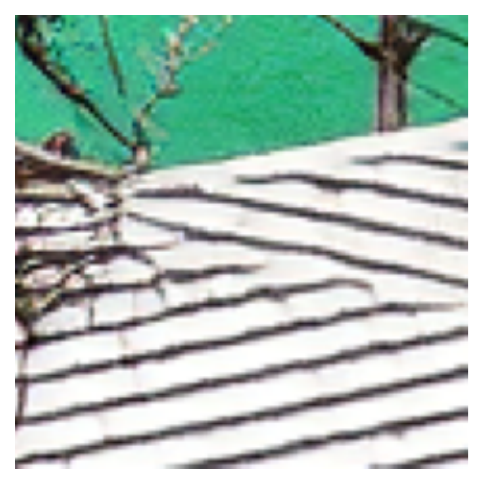} \\ \small SPSR \cite{ma_SPSR} \\ (14.64 / 0.179)
    \end{subfigure}
    \begin{subfigure}{\textwidth}
        \includegraphics[width=\textwidth]{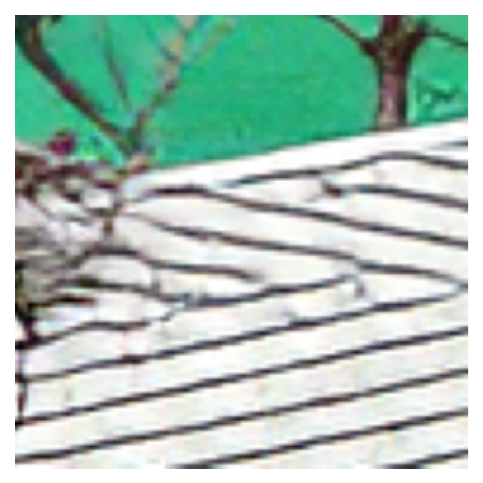} \\ \small RankSRGAN \cite{zhang2021ranksrgan} \\ (14.99 / 0.230)
    \end{subfigure}
    \begin{subfigure}{\textwidth}
        \includegraphics[width=\textwidth]{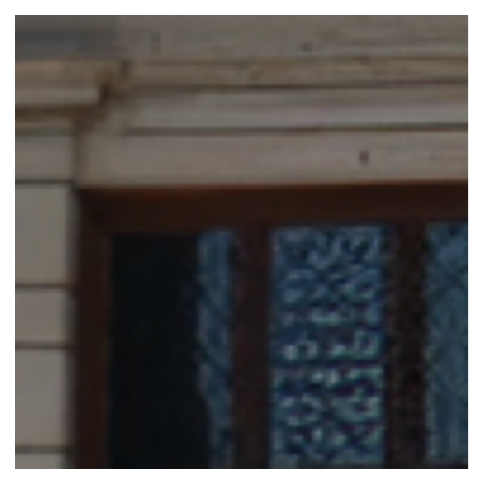} \\ \small SPSR \cite{ma_SPSR} \\ (29.92 / 0.127)
    \end{subfigure}
    \begin{subfigure}{\textwidth}
        \includegraphics[width=\textwidth]{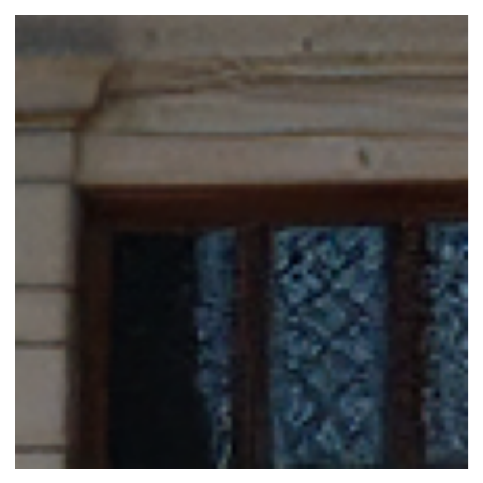} \\ \small RankSRGAN \cite{zhang2021ranksrgan} \\ (28.04 / 0.138)
    \end{subfigure}
    \begin{subfigure}{\textwidth}
        \includegraphics[width=\textwidth]{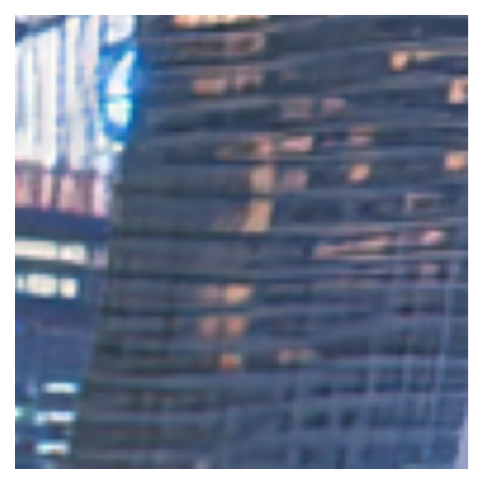} \\ \small SPSR \cite{ma_SPSR} \\ (23.88 / 0.184)
    \end{subfigure}
    \begin{subfigure}{\textwidth}
        \includegraphics[width=\textwidth]{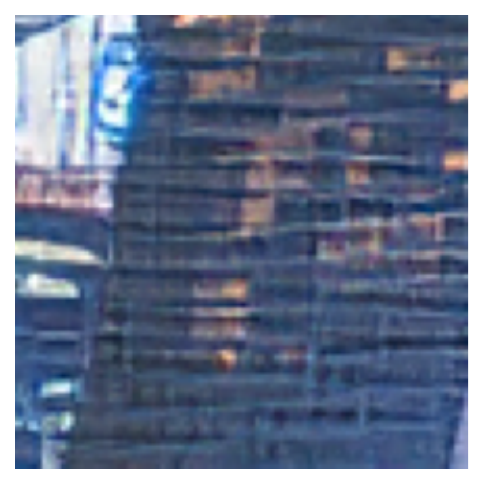} \\ \small RankSRGAN \cite{zhang2021ranksrgan} \\ (21.09 / 0.214)
    \end{subfigure}
\end{subfigure}
\begin{subfigure}{0.16\textwidth}
    \begin{subfigure}{\textwidth}
        \includegraphics[width=\textwidth]{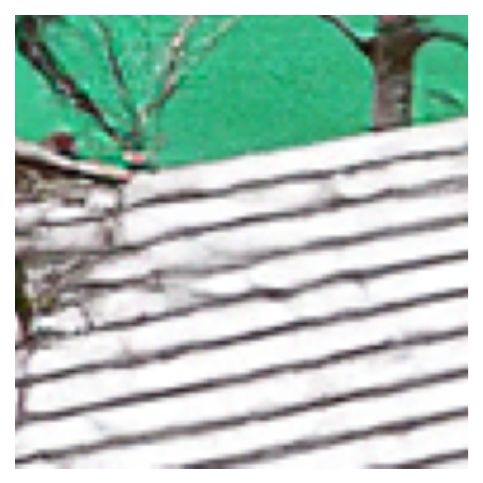} \\\small  SRFlow-DA \cite{jo2021srflowda} \\ (18.24 / 0.193)
    \end{subfigure}
    \begin{subfigure}{\textwidth}
        \includegraphics[width=\textwidth]{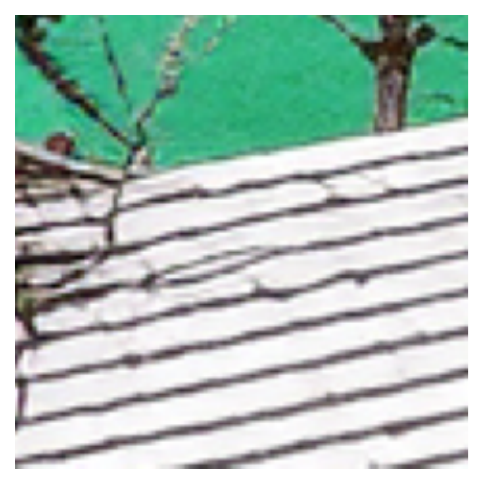} \\ \small LDL \cite{details_or_artifacts} \\ (18.02 / 0.167)
    \end{subfigure}
    \begin{subfigure}{\textwidth}
        \includegraphics[width=\textwidth]{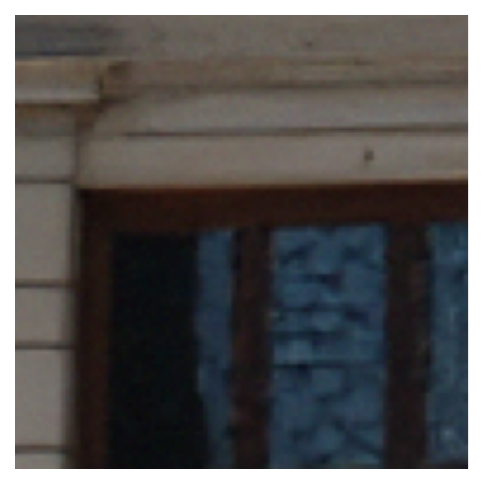} \\\small  SRFlow-DA \cite{jo2021srflowda} \\ (31.11 / 0.167)
    \end{subfigure}
    \begin{subfigure}{\textwidth}
        \includegraphics[width=\textwidth]{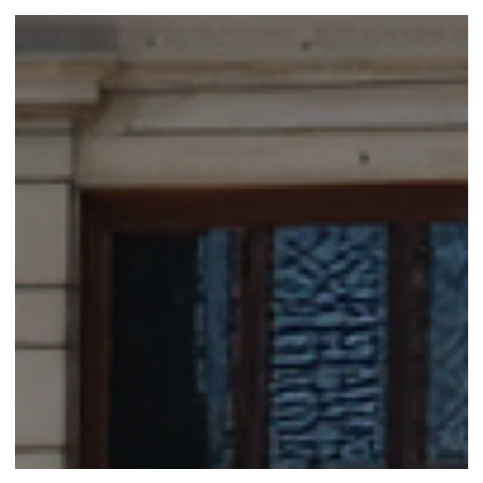} \\ \small LDL \cite{details_or_artifacts} \\ (28.75 / 0.149)
    \end{subfigure}
    \begin{subfigure}{\textwidth}
        \includegraphics[width=\textwidth]{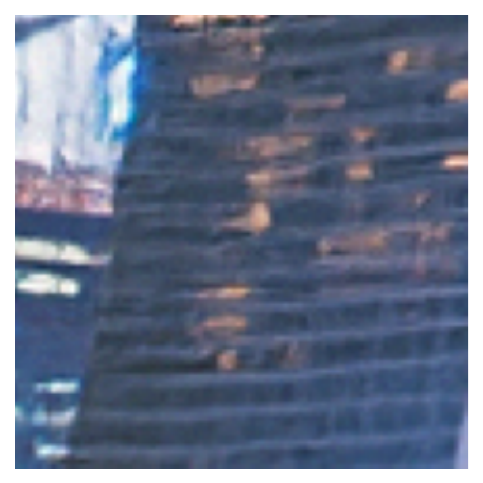} \\\small  SRFlow-DA \cite{jo2021srflowda} \\ (24.96 / 0.238)
    \end{subfigure}
    \begin{subfigure}{\textwidth}
        \includegraphics[width=\textwidth]{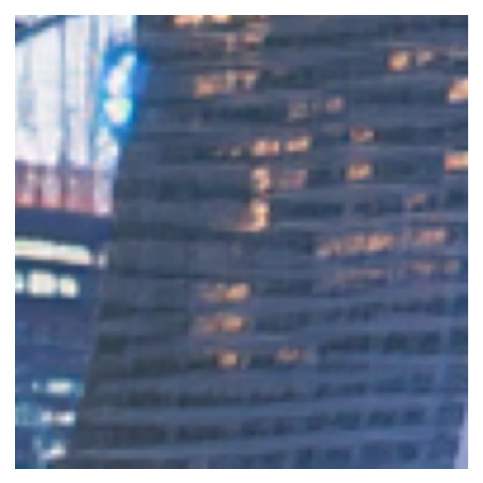} \\ \small LDL \cite{details_or_artifacts} \\ (24.41 / 0.179)
    \end{subfigure}
\end{subfigure}
\begin{subfigure}{0.16\textwidth}
    \begin{subfigure}{\textwidth}
        \includegraphics[width=\textwidth]{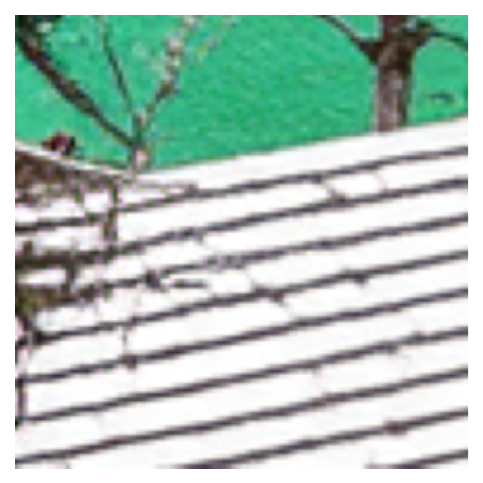} \\ \small FxSR \cite{fxsr} \\ (18.98 / 0.188)
    \end{subfigure}
            \begin{subfigure}{\textwidth}
        \includegraphics[width=\textwidth]{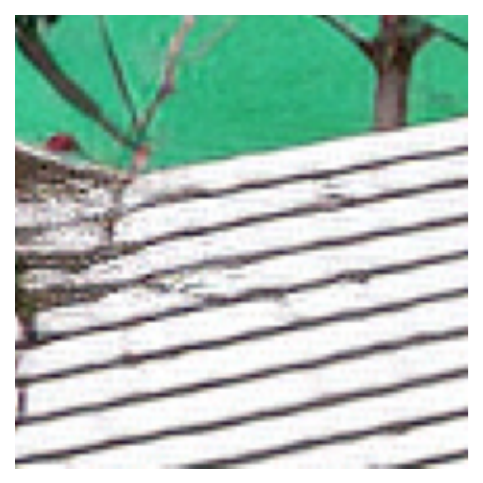} \\ \small PDASR \cite{PDASR} \\ (19.40 / 0.200)
    \end{subfigure}
    \begin{subfigure}{\textwidth}
        \includegraphics[width=\textwidth]{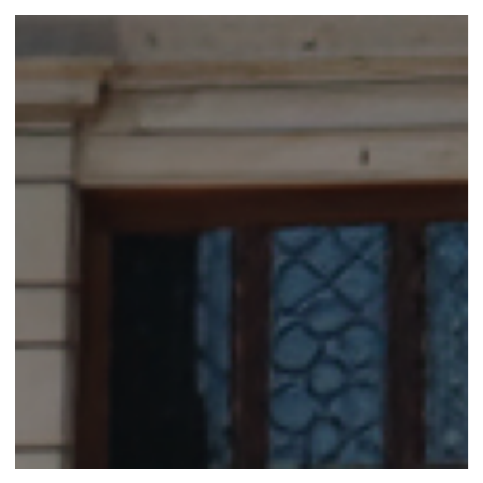} \\ \small FxSR \cite{fxsr} \\ (31.64 / 0.166)
    \end{subfigure}
            \begin{subfigure}{\textwidth}
        \includegraphics[width=\textwidth]{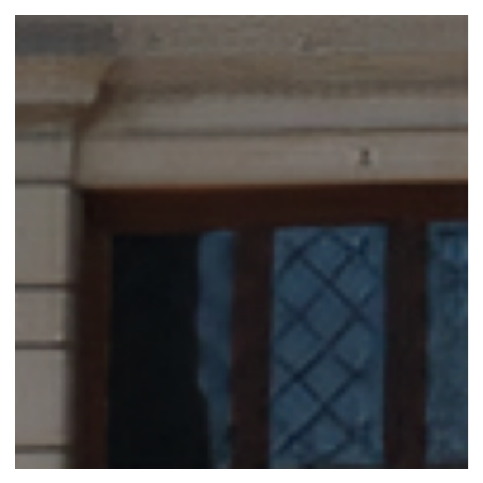} \\ \small PDASR \cite{PDASR} \\ (31.22 / 0.177)
    \end{subfigure}
    \begin{subfigure}{\textwidth}
        \includegraphics[width=\textwidth]{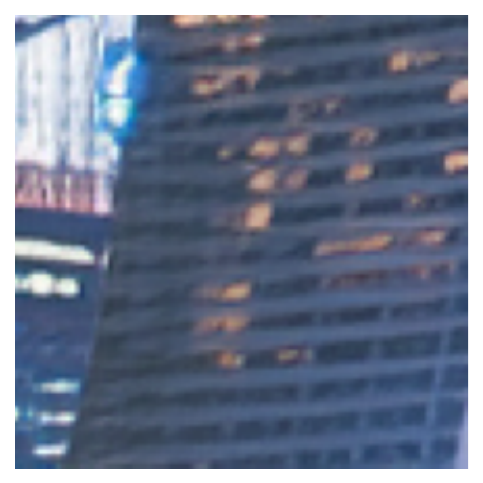} \\ \small FxSR \cite{fxsr} \\ (24.84 / 0.190)
    \end{subfigure}
            \begin{subfigure}{\textwidth}
        \includegraphics[width=\textwidth]{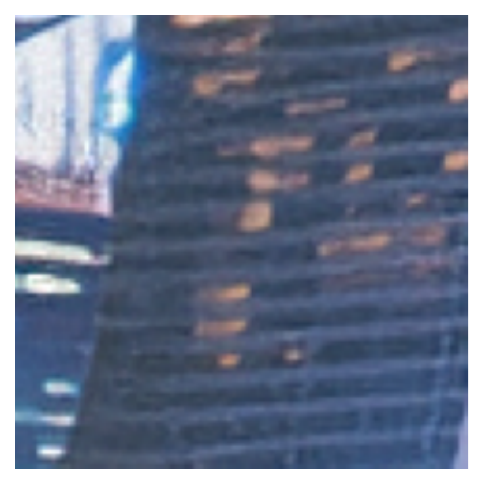} \\ \small PDASR \cite{PDASR} \\ (25.72 / 0.222)
    \end{subfigure}
\end{subfigure}
\begin{subfigure}{0.16\textwidth}
    \begin{subfigure}{\textwidth}
        \includegraphics[width=\textwidth]{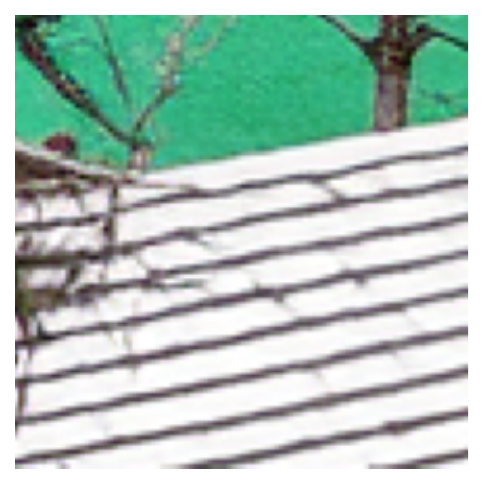} \\ \small SROOE \cite{srooe_Park_2023_CVPR} \\ (19.26 / 0.156)
    \end{subfigure}
    \begin{subfigure}{\textwidth}
        \includegraphics[width=\textwidth]{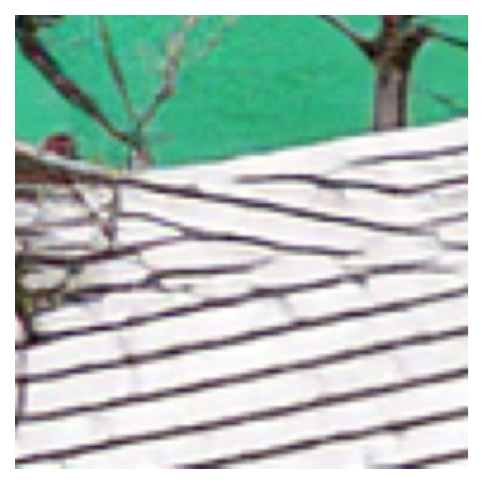} \\ \small  DualFormer \cite{dualformer_luo2023effectiveness} \\ (16.58 / 0.172)
    \end{subfigure}
    \begin{subfigure}{\textwidth}
        \includegraphics[width=\textwidth]{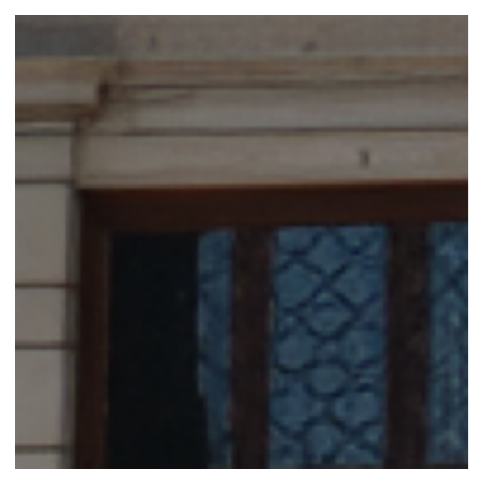} \\ \small SROOE \cite{srooe_Park_2023_CVPR} \\ (31.02 / 0.167)
    \end{subfigure}
    \begin{subfigure}{\textwidth}
        \includegraphics[width=\textwidth]{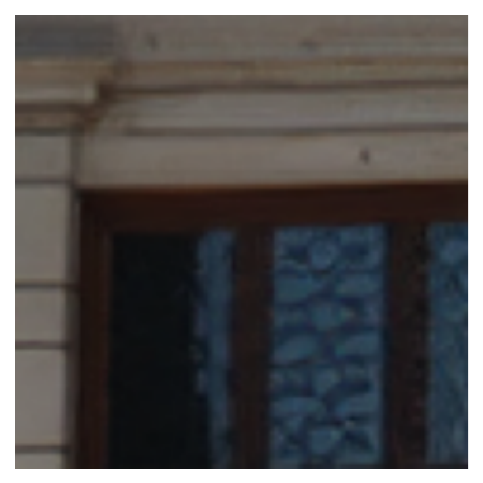} \\ \small  DualFormer \cite{dualformer_luo2023effectiveness} \\ (31.59 / 0.150)
    \end{subfigure}
    \begin{subfigure}{\textwidth}
        \includegraphics[width=\textwidth]{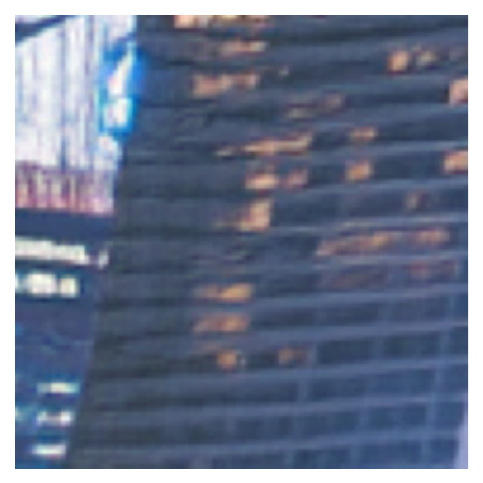} \\ \small SROOE \cite{srooe_Park_2023_CVPR} \\ (24.95 / 0.194)
    \end{subfigure}
    \begin{subfigure}{\textwidth}
        \includegraphics[width=\textwidth]{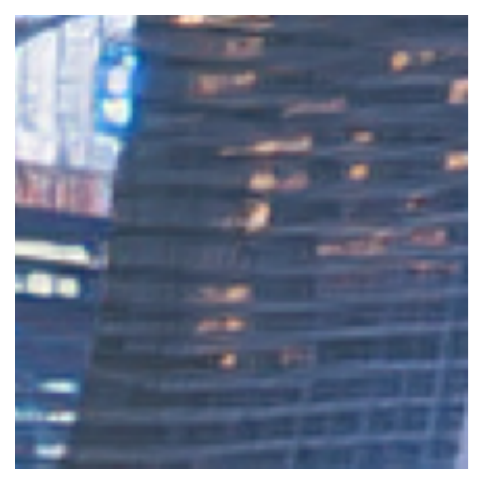} \\ \small  DualFormer \cite{dualformer_luo2023effectiveness} \\ (24.73 / 0.206)
    \end{subfigure}
\end{subfigure}
\begin{subfigure}{0.16\textwidth}
    \begin{subfigure}{\textwidth}
        \includegraphics[width=\textwidth]{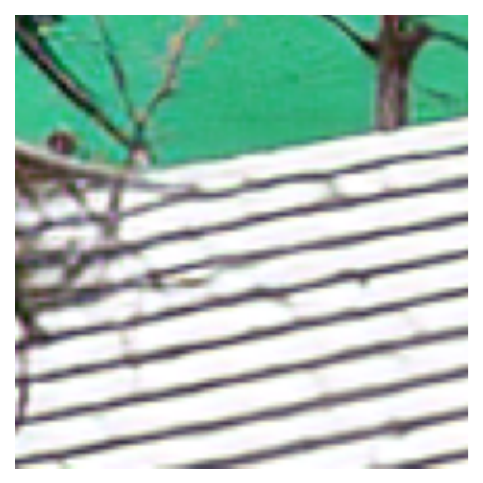} \\ \small WGSR (Ours) \\(19.64 / 0.176)
    \end{subfigure}
        \begin{subfigure}{\textwidth}
        \includegraphics[width=\textwidth]{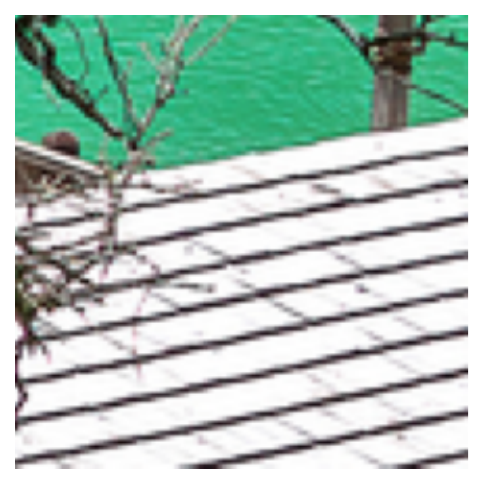} \\ \small HR (img-807)\\ (PSNR$\uparrow$ / DISTS$\downarrow$\cite{dists})
    \end{subfigure}
    \begin{subfigure}{\textwidth}
        \includegraphics[width=\textwidth]{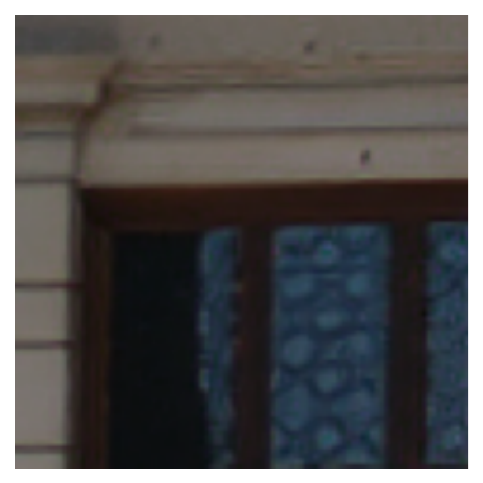} \\ \small WGSR (Ours) \\(31.85 / 0.147)
    \end{subfigure}
        \begin{subfigure}{\textwidth}
        \includegraphics[width=\textwidth]{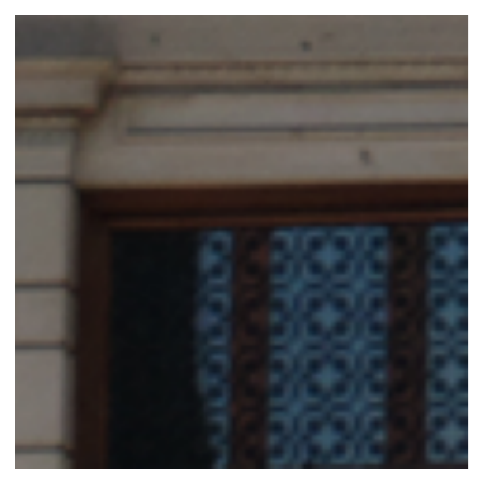} \\ \small HR (img-812)\\ (PSNR$\uparrow$ / DISTS$\downarrow$\cite{dists})
    \end{subfigure}
    \begin{subfigure}{\textwidth}
        \includegraphics[width=\textwidth]{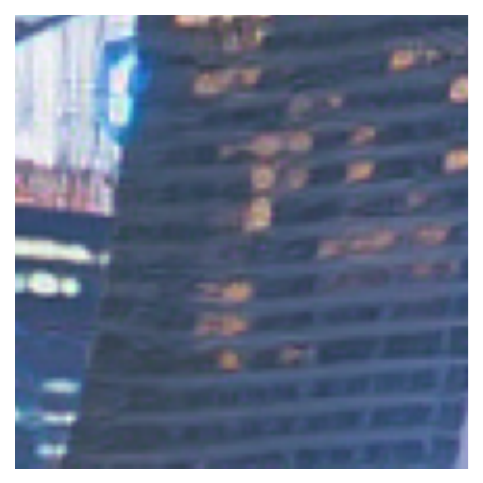} \\ \small WGSR (Ours) \\(26.11 / 0.183)
    \end{subfigure}
        \begin{subfigure}{\textwidth}
        \includegraphics[width=\textwidth]{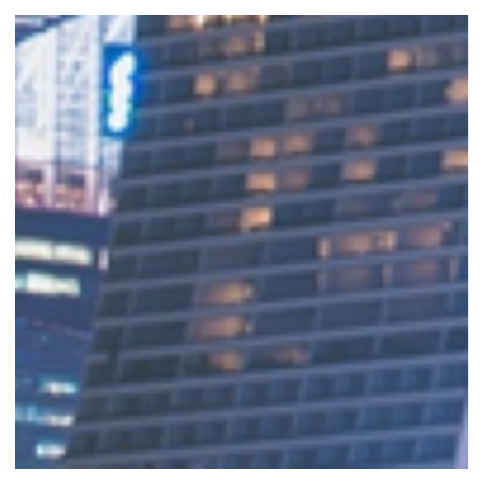} \\ \small HR (img-814)\\ (PSNR$\uparrow$ / DISTS$\downarrow$\cite{dists})
    \end{subfigure}
\end{subfigure} 
\caption{Visual comparison of the proposed wavelet-guided perceptual optimization method with the state-of-the-art for $\times$4 SR on natural images from DIV2K validation set \cite{Agustsson_2017_CVPR_Workshops}. The proposed WGSR has clear advantages in reconstructing realistic high-frequency details while inhibiting artifacts.}
\label{fig:supp_div2k1} 
\end{figure*}

\begin{figure*}
\centering
\begin{subfigure}{0.16\textwidth}
     \begin{subfigure}{\textwidth}
        \includegraphics[width=\textwidth]{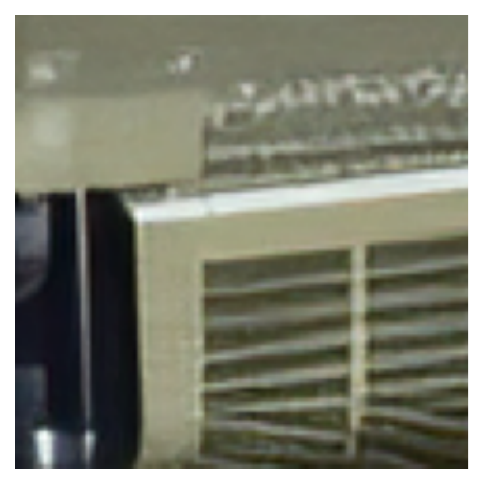} \\ \small ESRGAN-FS \cite{freq_sep} \\ (24.76 / 0.130)
    \end{subfigure}
    \begin{subfigure}{\textwidth}
        \includegraphics[width=\textwidth]{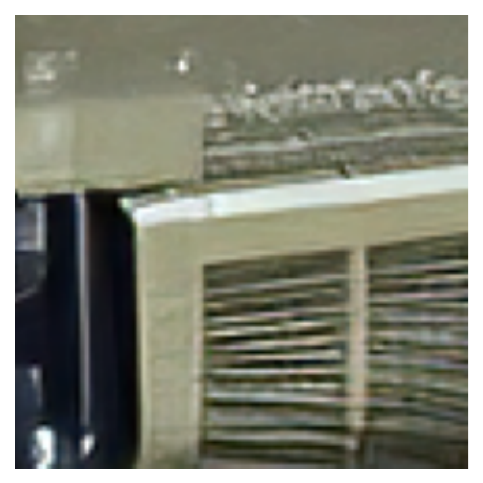} \\ \small ESRGAN+ \cite{esrganplus} \\ (20.79 / 0.179)
    \end{subfigure}
     \begin{subfigure}{\textwidth}
        \includegraphics[width=\textwidth]{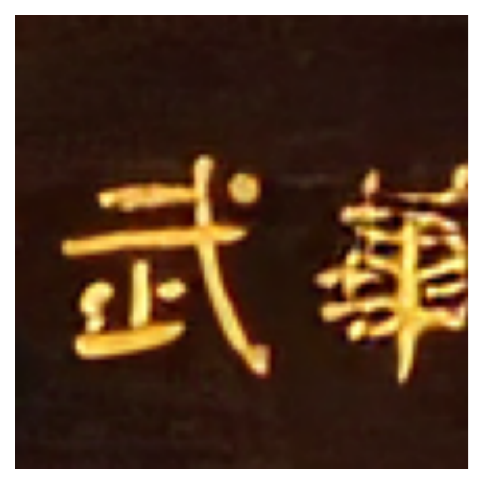} \\ \small ESRGAN-FS \cite{freq_sep} \\ (21.00 / 0.146)
    \end{subfigure}
    \begin{subfigure}{\textwidth}
        \includegraphics[width=\textwidth]{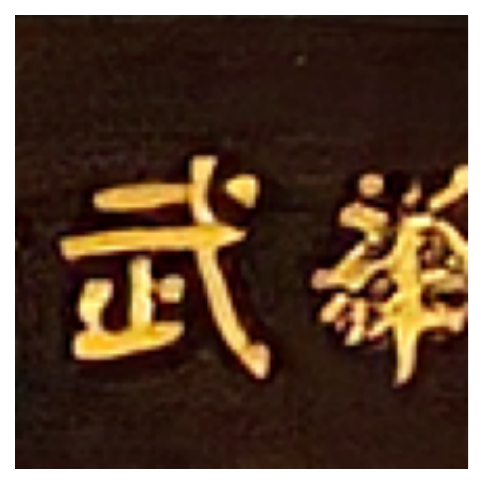} \\ \small ESRGAN+ \cite{esrganplus} \\ (19.53 / 0.168)
    \end{subfigure}
     \begin{subfigure}{\textwidth}
        \includegraphics[width=\textwidth]{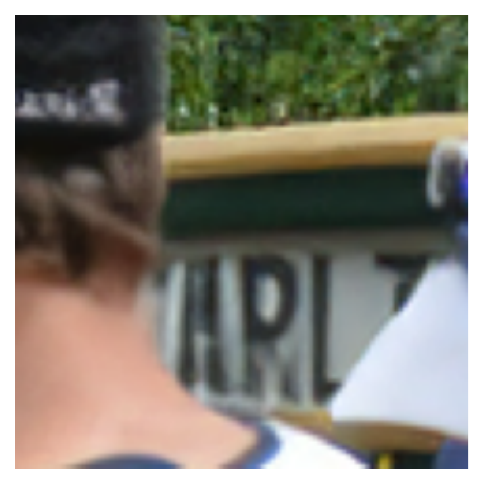} \\ \small ESRGAN-FS \cite{freq_sep} \\ (26.38 / 0.129)
    \end{subfigure}
    \begin{subfigure}{\textwidth}
        \includegraphics[width=\textwidth]{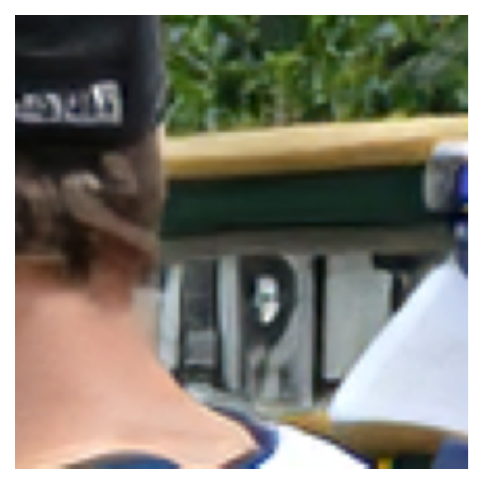} \\ \small ESRGAN+ \cite{esrganplus} \\ (24.51 / 0.173)
    \end{subfigure}
\end{subfigure}
\begin{subfigure}{0.16\textwidth}
    \begin{subfigure}{\textwidth}
        \includegraphics[width=\textwidth]{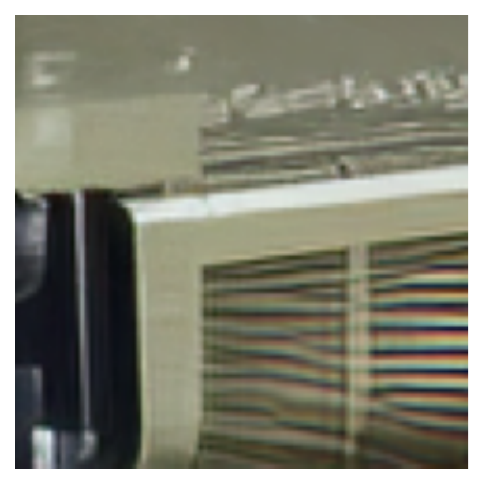} \\ \small SPSR \cite{ma_SPSR} \\ (22.28 / 0.175)
    \end{subfigure}
    \begin{subfigure}{\textwidth}
        \includegraphics[width=\textwidth]{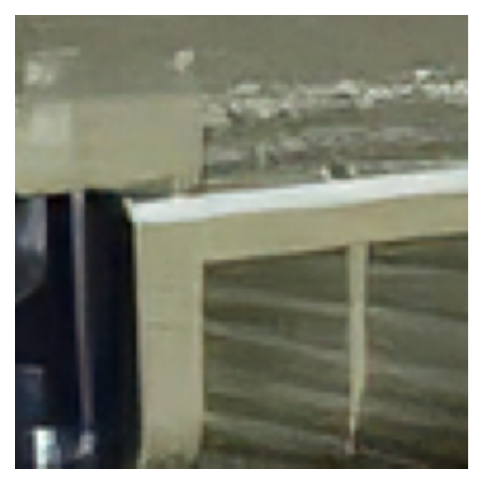} \\ \small RankSRGAN \cite{zhang2021ranksrgan} \\ (24.66 / 0.175)
    \end{subfigure}
    \begin{subfigure}{\textwidth}
        \includegraphics[width=\textwidth]{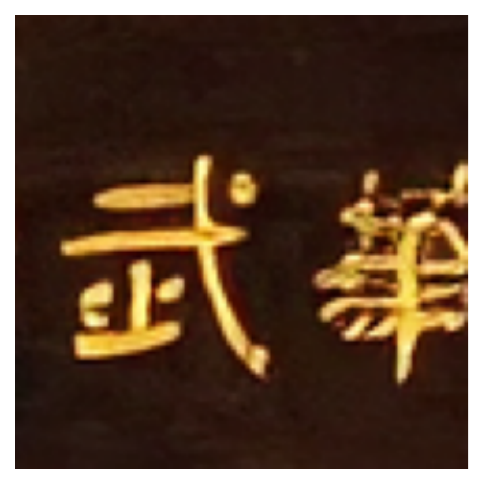} \\ \small SPSR \cite{ma_SPSR} \\ (20.86 / 0.145)
    \end{subfigure}
    \begin{subfigure}{\textwidth}
        \includegraphics[width=\textwidth]{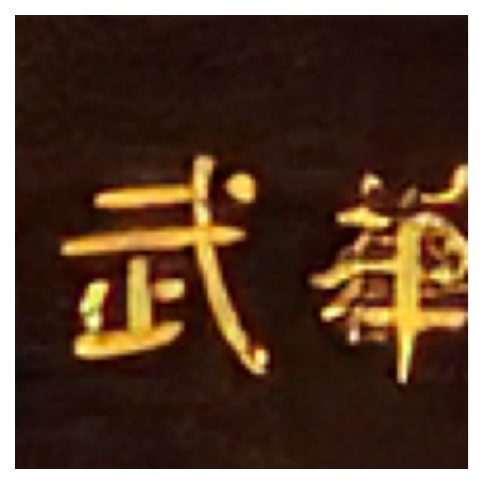} \\ \small RankSRGAN \cite{zhang2021ranksrgan} \\ (20.29 / 0.148)
    \end{subfigure}
    \begin{subfigure}{\textwidth}
        \includegraphics[width=\textwidth]{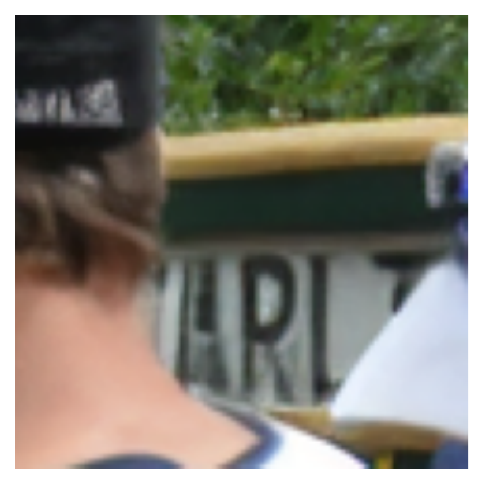} \\ \small SPSR \cite{ma_SPSR} \\ (27.25 / 0.123)
    \end{subfigure}
    \begin{subfigure}{\textwidth}
        \includegraphics[width=\textwidth]{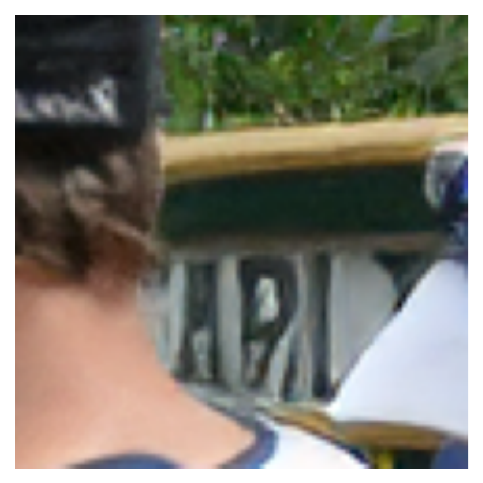} \\ \small RankSRGAN \cite{zhang2021ranksrgan} \\ (25.07 / 0.170)
    \end{subfigure}
\end{subfigure}
\begin{subfigure}{0.16\textwidth}
    \begin{subfigure}{\textwidth}
        \includegraphics[width=\textwidth]{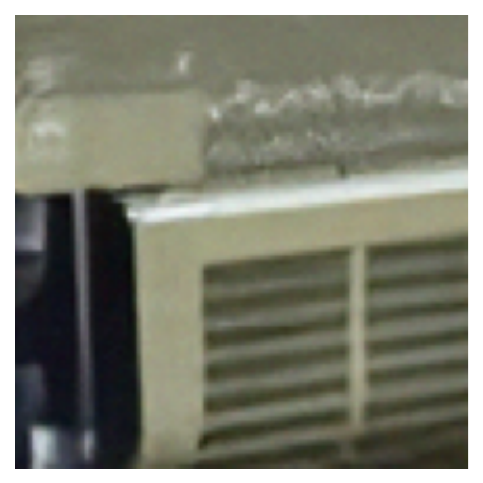} \\\small  SRFlow-DA \cite{jo2021srflowda} \\ (27.88 / 0.126)
    \end{subfigure}
    \begin{subfigure}{\textwidth}
        \includegraphics[width=\textwidth]{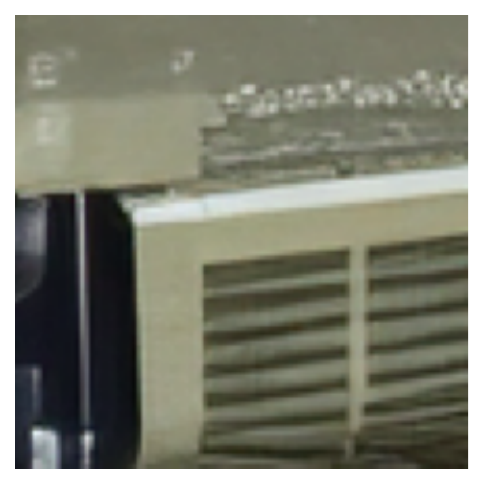} \\ \small LDL \cite{details_or_artifacts} \\ (24.91 / 0.133)
    \end{subfigure}
    \begin{subfigure}{\textwidth}
        \includegraphics[width=\textwidth]{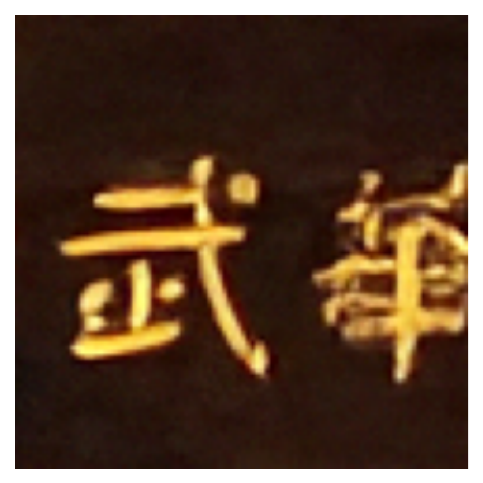} \\\small  SRFlow-DA \cite{jo2021srflowda} \\ (21.34 / 0.140)
    \end{subfigure}
    \begin{subfigure}{\textwidth}
        \includegraphics[width=\textwidth]{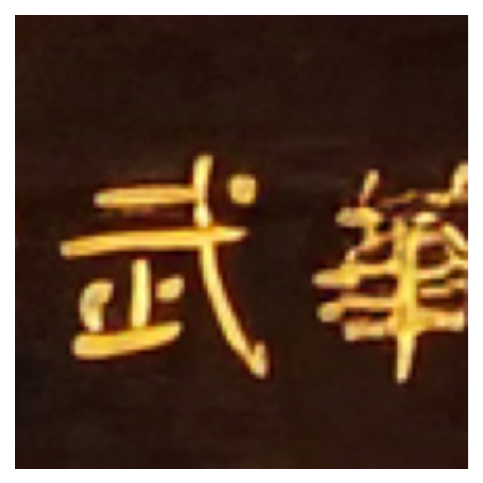} \\ \small LDL \cite{details_or_artifacts} \\ (21.66 / 0.136)
    \end{subfigure}
    \begin{subfigure}{\textwidth}
        \includegraphics[width=\textwidth]{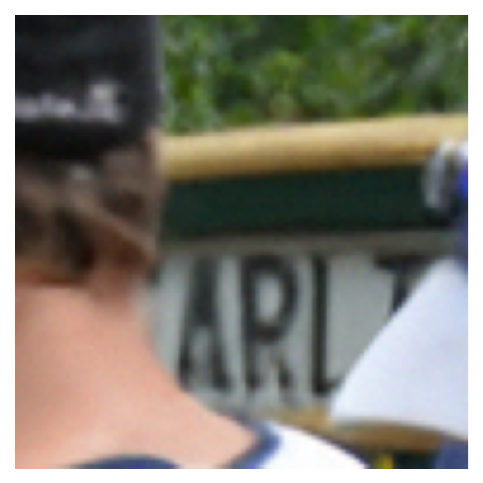} \\\small  SRFlow-DA \cite{jo2021srflowda} \\ (28.32 / 0.136)
    \end{subfigure}
    \begin{subfigure}{\textwidth}
        \includegraphics[width=\textwidth]{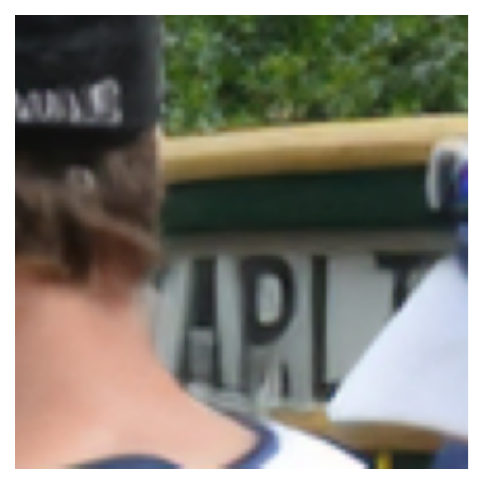} \\ \small LDL \cite{details_or_artifacts} \\ (27.81 / 0.124)
    \end{subfigure}
\end{subfigure}
\begin{subfigure}{0.16\textwidth}
    \begin{subfigure}{\textwidth}
        \includegraphics[width=\textwidth]{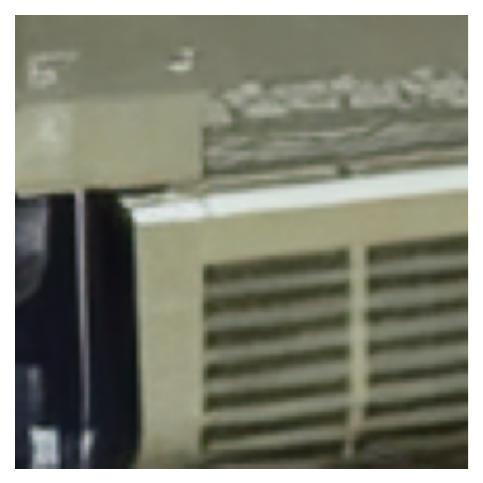} \\ \small FxSR \cite{fxsr} \\ (26.28 / 0.140)
    \end{subfigure}
            \begin{subfigure}{\textwidth}
        \includegraphics[width=\textwidth]{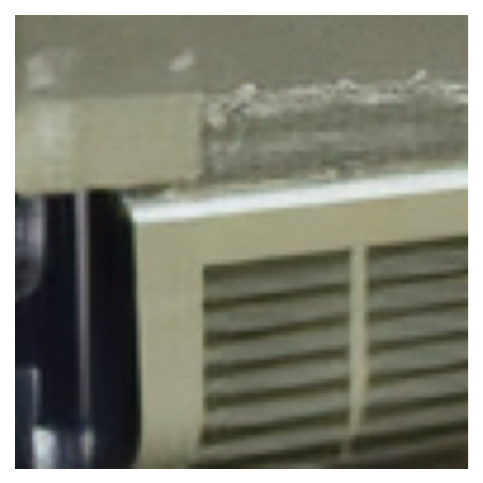} \\ \small PDASR \cite{PDASR} \\ (27.77 / 0.120)
    \end{subfigure}
    \begin{subfigure}{\textwidth}
        \includegraphics[width=\textwidth]{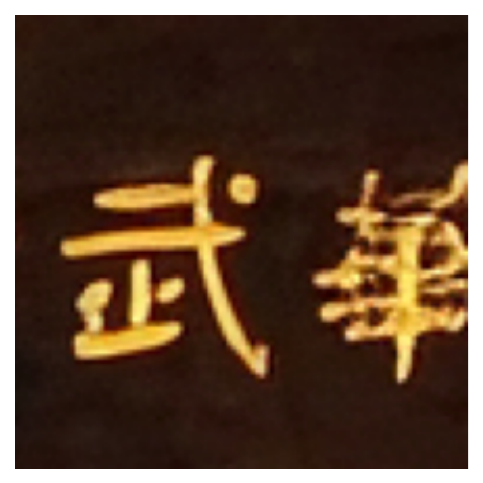} \\ \small FxSR \cite{fxsr} \\ (21.67 / 0.138)
    \end{subfigure}
            \begin{subfigure}{\textwidth}
        \includegraphics[width=\textwidth]{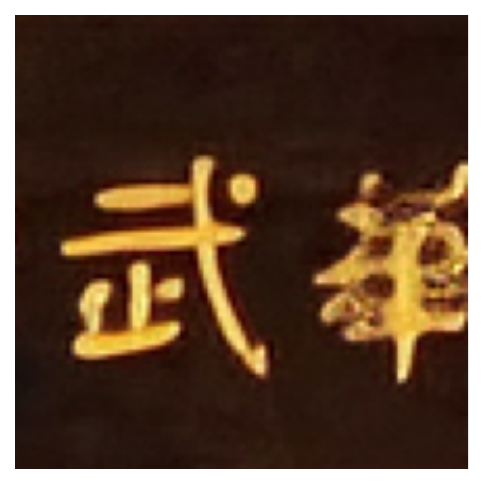} \\ \small PDASR \cite{PDASR} \\ (22.66 / 0.154)
    \end{subfigure}
    \begin{subfigure}{\textwidth}
        \includegraphics[width=\textwidth]{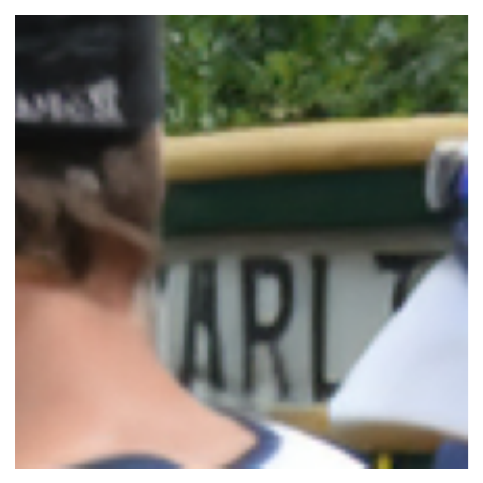} \\ \small FxSR \cite{fxsr} \\ (28.70 / 0.134)
    \end{subfigure}
            \begin{subfigure}{\textwidth}
        \includegraphics[width=\textwidth]{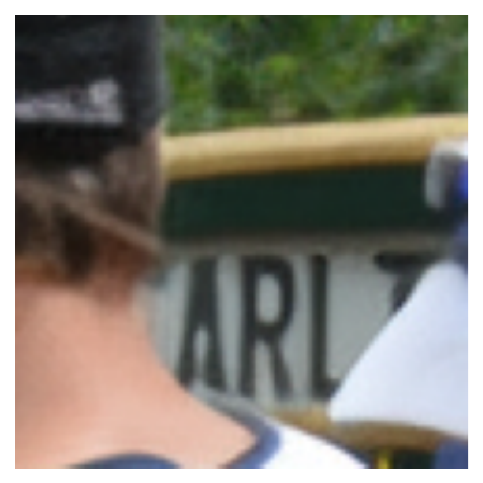} \\ \small PDASR \cite{PDASR} \\ (29.99 / 0.136)
    \end{subfigure}
\end{subfigure}
\begin{subfigure}{0.16\textwidth}
    \begin{subfigure}{\textwidth}
        \includegraphics[width=\textwidth]{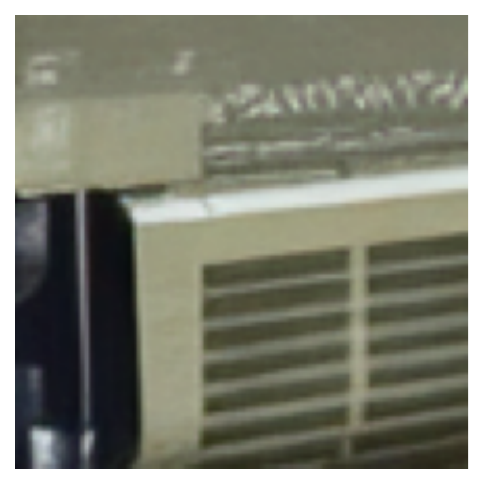} \\ \small SROOE \cite{srooe_Park_2023_CVPR} \\ (27.39 / 0.120)
    \end{subfigure}
    \begin{subfigure}{\textwidth}
        \includegraphics[width=\textwidth]{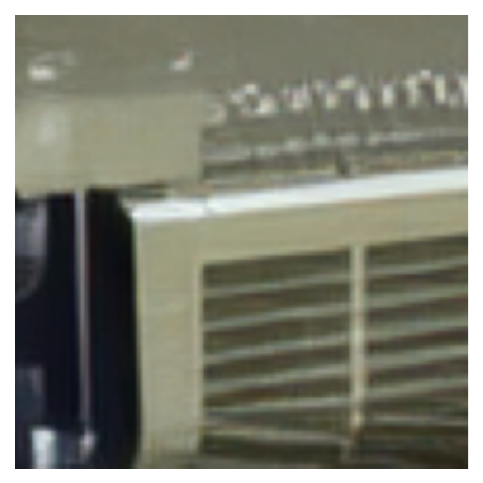} \\ \small  DualFormer \cite{dualformer_luo2023effectiveness} \\ (26.08 / 0.118)
    \end{subfigure}
    \begin{subfigure}{\textwidth}
        \includegraphics[width=\textwidth]{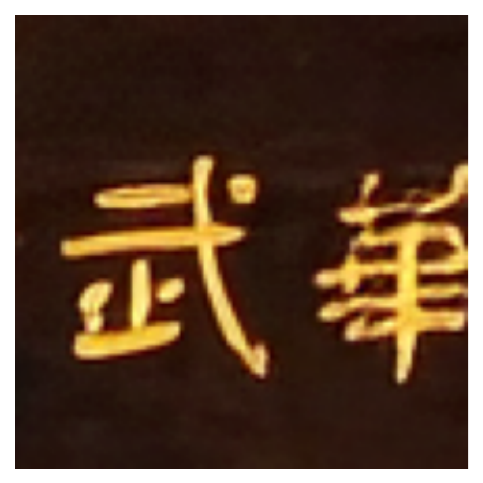} \\ \small SROOE \cite{srooe_Park_2023_CVPR} \\ (23.26 / 0.126)
    \end{subfigure}
    \begin{subfigure}{\textwidth}
        \includegraphics[width=\textwidth]{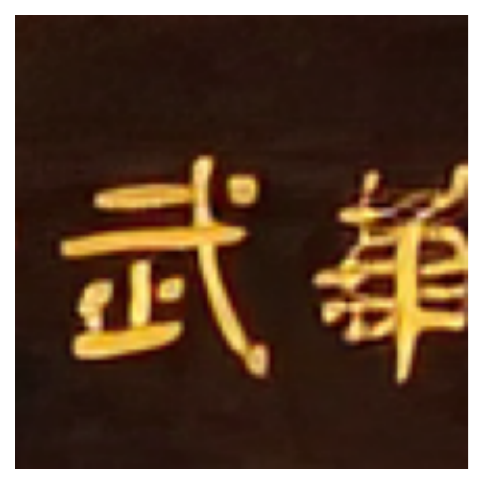} \\ \small  DualFormer \cite{dualformer_luo2023effectiveness} \\ (23.24 / 0.117)
    \end{subfigure}
    \begin{subfigure}{\textwidth}
        \includegraphics[width=\textwidth]{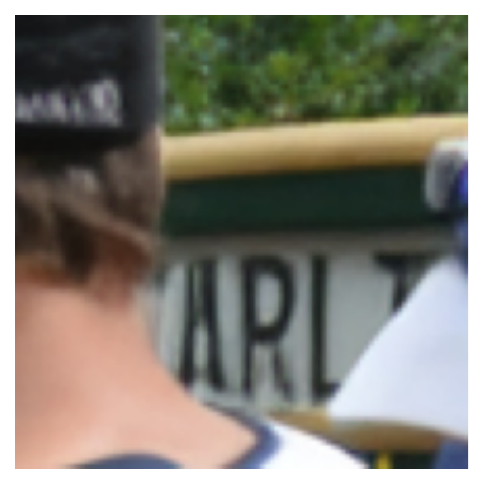} \\ \small SROOE \cite{srooe_Park_2023_CVPR} \\ (29.13 / 0.127)
    \end{subfigure}
    \begin{subfigure}{\textwidth}
        \includegraphics[width=\textwidth]{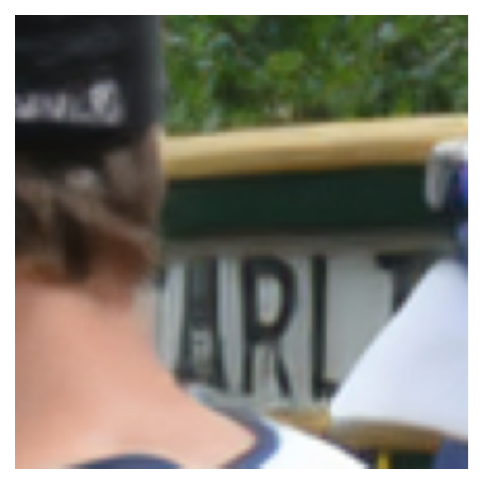} \\ \small  DualFormer \cite{dualformer_luo2023effectiveness} \\ (28.77 / 0.122)
    \end{subfigure}
\end{subfigure}
\begin{subfigure}{0.16\textwidth}
    \begin{subfigure}{\textwidth}
        \includegraphics[width=\textwidth]{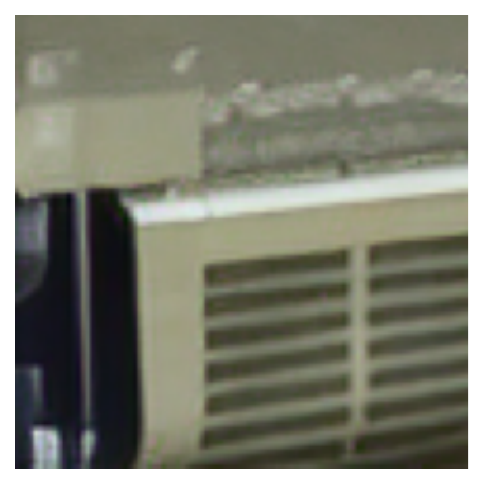} \\ \small WGSR (Ours) \\(27.99 / 0.115)
    \end{subfigure}
        \begin{subfigure}{\textwidth}
        \includegraphics[width=\textwidth]{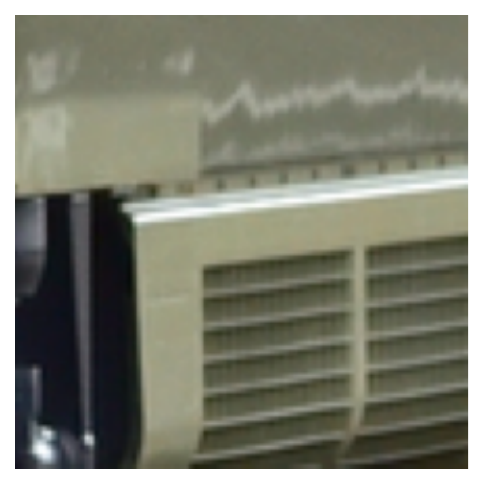} \\ \small HR (img-820)\\ (PSNR$\uparrow$ / DISTS$\downarrow$\cite{dists})
    \end{subfigure}
    \begin{subfigure}{\textwidth}
        \includegraphics[width=\textwidth]{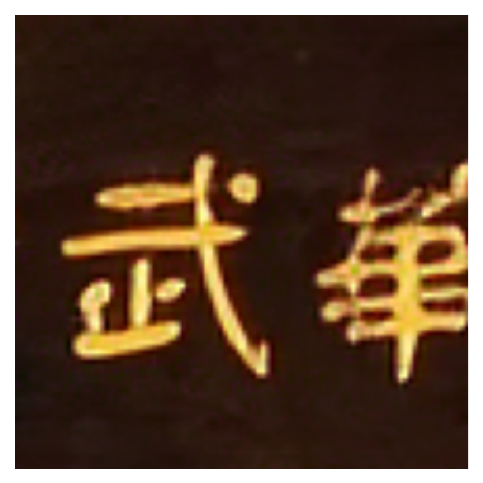} \\ \small WGSR (Ours) \\(24.19 / 0.121)
    \end{subfigure}
        \begin{subfigure}{\textwidth}
        \includegraphics[width=\textwidth]{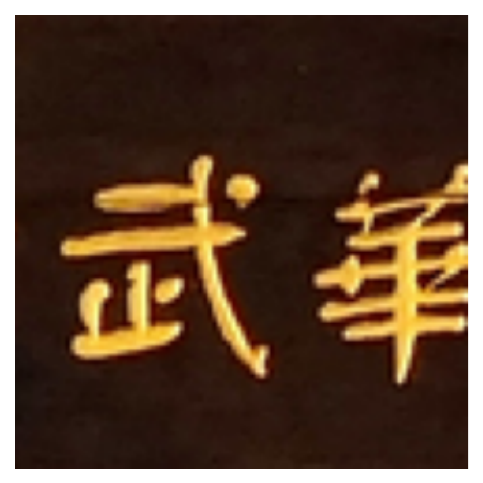} \\ \small HR (img-826)\\ (PSNR$\uparrow$ / DISTS$\downarrow$\cite{dists})
    \end{subfigure}
    \begin{subfigure}{\textwidth}
        \includegraphics[width=\textwidth]{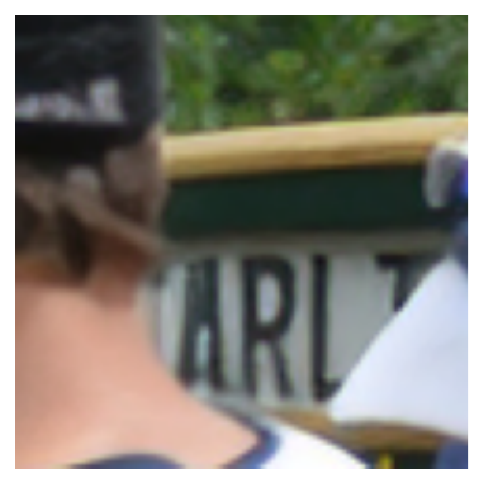} \\ \small WGSR (Ours) \\(29.70 / 0.120)
    \end{subfigure}
        \begin{subfigure}{\textwidth}
        \includegraphics[width=\textwidth]{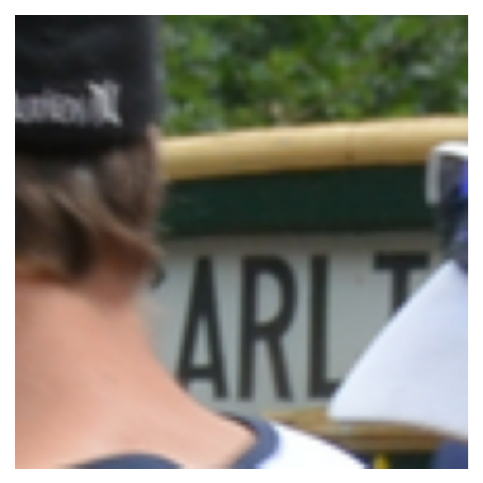} \\ \small HR (img-832)\\ (PSNR$\uparrow$ / DISTS$\downarrow$\cite{dists})
    \end{subfigure}
\end{subfigure} 
\caption{Visual comparison of the proposed wavelet-guided perceptual optimization method with the state-of-the-art for $\times$4 SR on natural images from DIV2K validation set \cite{Agustsson_2017_CVPR_Workshops}.}
\label{fig:supp_div2k2} 
\end{figure*}

\begin{figure*}
\centering
\begin{subfigure}{0.16\textwidth}
     \begin{subfigure}{\textwidth}
        \includegraphics[width=\textwidth]{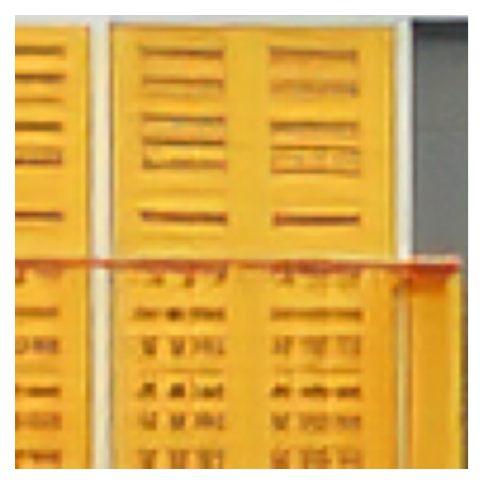} \\ \small ESRGAN-FS \cite{freq_sep} \\ (22.35 / 0.148)
    \end{subfigure}
    \begin{subfigure}{\textwidth}
        \includegraphics[width=\textwidth]{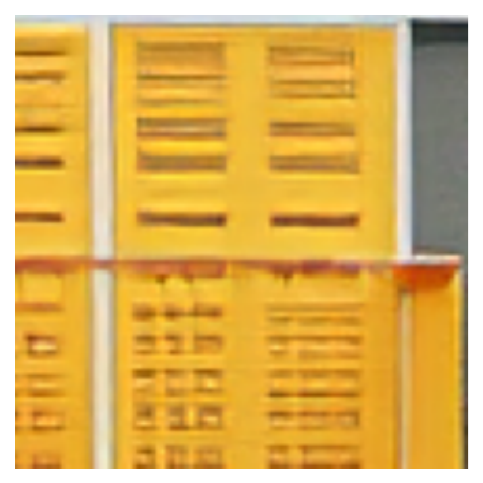} \\ \small ESRGAN+ \cite{esrganplus} \\ (21.05 / 0.144)
    \end{subfigure}
     \begin{subfigure}{\textwidth}
        \includegraphics[width=\textwidth]{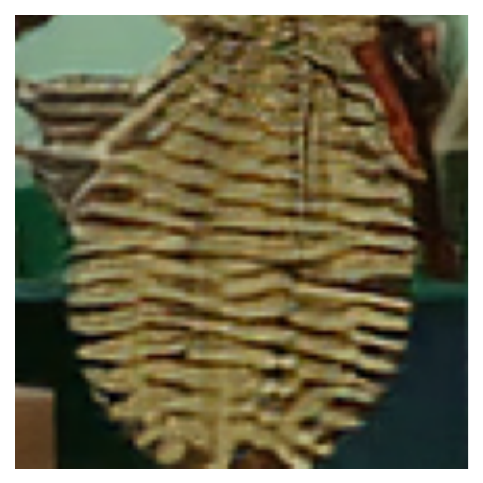} \\ \small ESRGAN-FS \cite{freq_sep} \\ (18.91 / 0.211)
    \end{subfigure}
    \begin{subfigure}{\textwidth}
        \includegraphics[width=\textwidth]{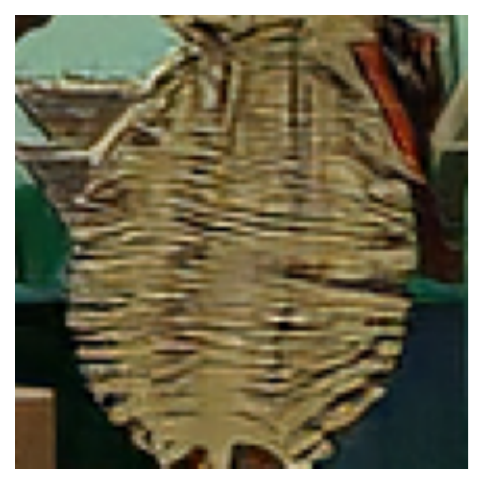} \\ \small ESRGAN+ \cite{esrganplus} \\ (17.83 / 0.246)
    \end{subfigure}
     \begin{subfigure}{\textwidth}
        \includegraphics[width=\textwidth]{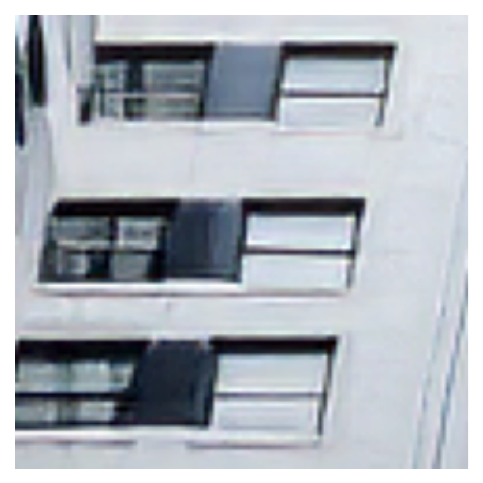} \\ \small ESRGAN-FS \cite{freq_sep} \\ (20.52 / 0.166)
    \end{subfigure}
    \begin{subfigure}{\textwidth}
        \includegraphics[width=\textwidth]{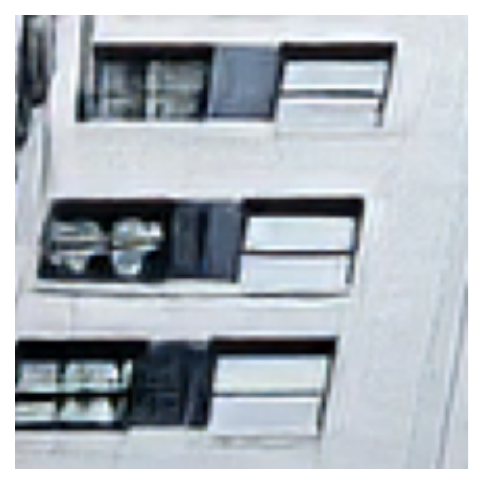} \\ \small ESRGAN+ \cite{esrganplus} \\ (18.81 / 0.190)
    \end{subfigure}
\end{subfigure}
\begin{subfigure}{0.16\textwidth}
    \begin{subfigure}{\textwidth}
        \includegraphics[width=\textwidth]{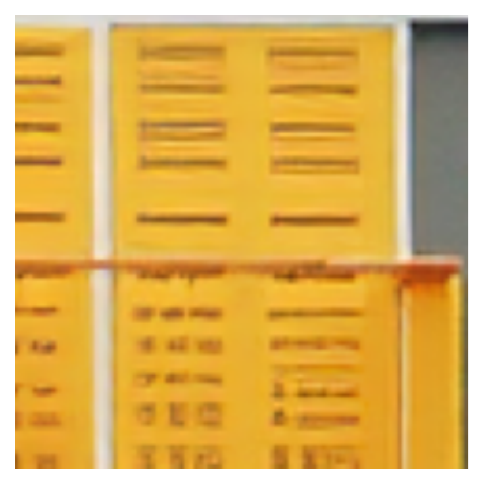} \\ \small SPSR \cite{ma_SPSR} \\ (23.24 / 0.129)
    \end{subfigure}
    \begin{subfigure}{\textwidth}
        \includegraphics[width=\textwidth]{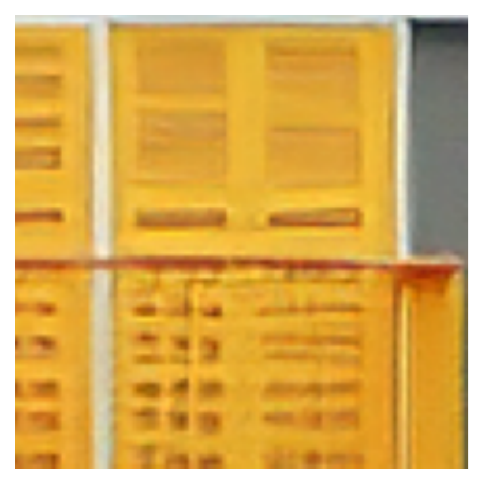} \\ \small RankSRGAN \cite{zhang2021ranksrgan} \\ (21.24 / 0.190)
    \end{subfigure}
    \begin{subfigure}{\textwidth}
        \includegraphics[width=\textwidth]{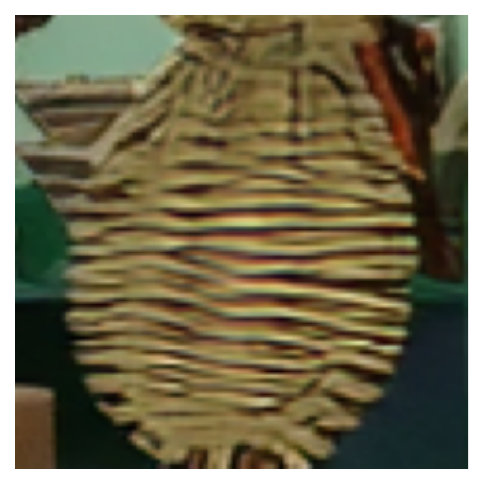} \\ \small SPSR \cite{ma_SPSR} \\ (18.65 / 0.233)
    \end{subfigure}
    \begin{subfigure}{\textwidth}
        \includegraphics[width=\textwidth]{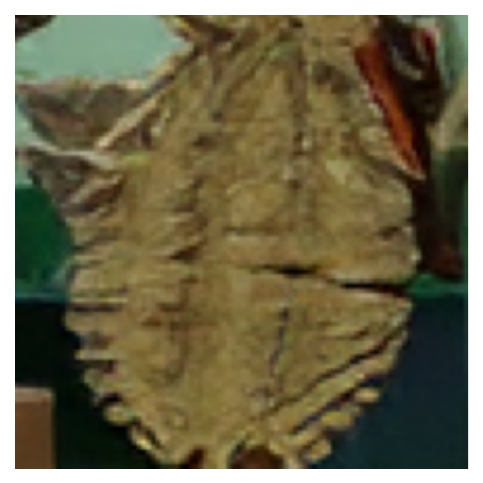} \\ \small RankSRGAN \cite{zhang2021ranksrgan} \\ (20.00 / 0.294)
    \end{subfigure}
    \begin{subfigure}{\textwidth}
        \includegraphics[width=\textwidth]{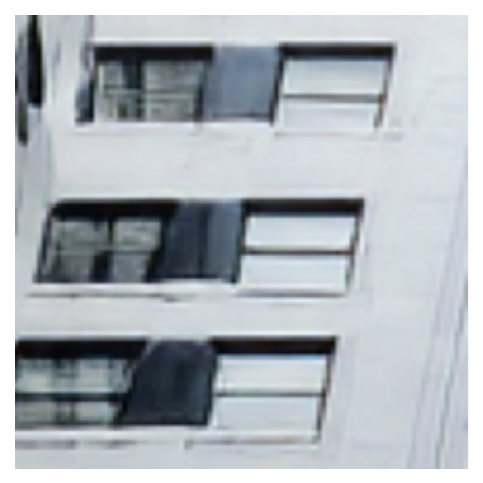} \\ \small SPSR \cite{ma_SPSR} \\ (21.14 / 0.166)
    \end{subfigure}
    \begin{subfigure}{\textwidth}
        \includegraphics[width=\textwidth]{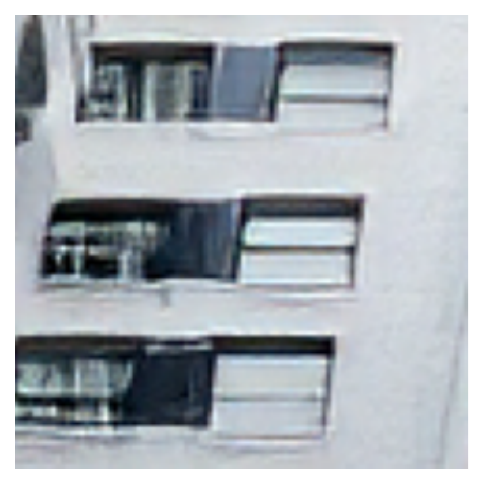} \\ \small RankSRGAN \cite{zhang2021ranksrgan} \\ (18.28 / 0.196)
    \end{subfigure}
\end{subfigure}
\begin{subfigure}{0.16\textwidth}
    \begin{subfigure}{\textwidth}
        \includegraphics[width=\textwidth]{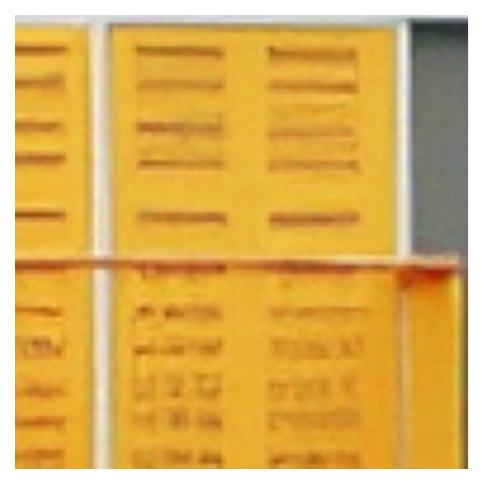} \\\small  SRFlow-DA \cite{jo2021srflowda} \\ (23.66 / 0.155)
    \end{subfigure}
    \begin{subfigure}{\textwidth}
        \includegraphics[width=\textwidth]{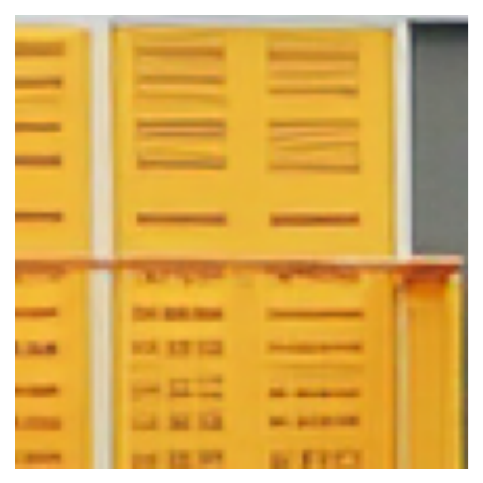} \\ \small LDL \cite{details_or_artifacts} \\ (23.46 / 0.115)
    \end{subfigure}
    \begin{subfigure}{\textwidth}
        \includegraphics[width=\textwidth]{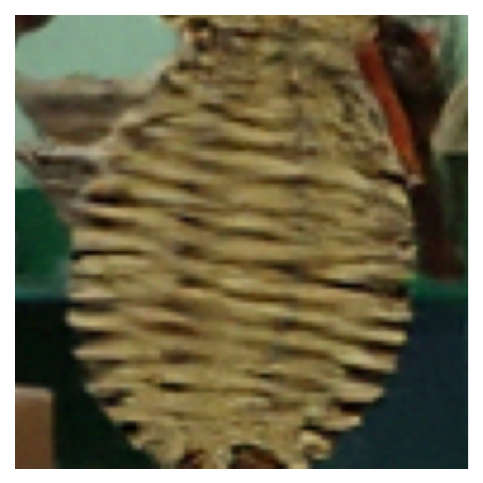} \\\small  SRFlow-DA \cite{jo2021srflowda} \\ (20.54 / 0.186)
    \end{subfigure}
    \begin{subfigure}{\textwidth}
        \includegraphics[width=\textwidth]{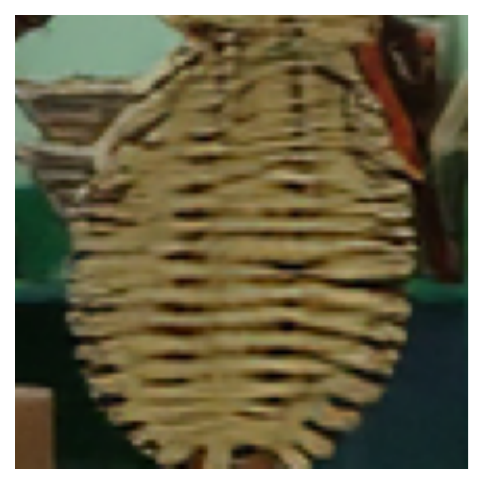} \\ \small LDL \cite{details_or_artifacts} \\ (20.16 / 0.202)
    \end{subfigure}
    \begin{subfigure}{\textwidth}
        \includegraphics[width=\textwidth]{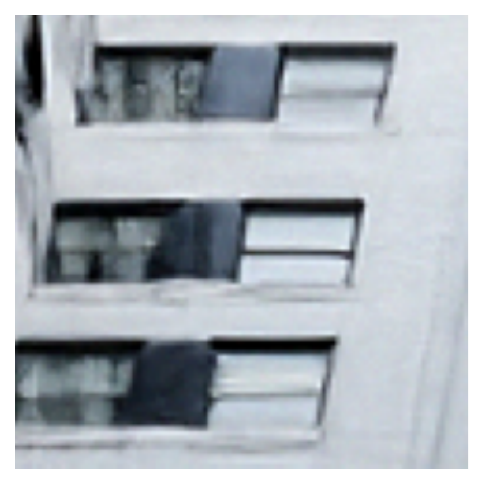} \\\small  SRFlow-DA \cite{jo2021srflowda} \\ (21.38 / 0.181)
    \end{subfigure}
    \begin{subfigure}{\textwidth}
        \includegraphics[width=\textwidth]{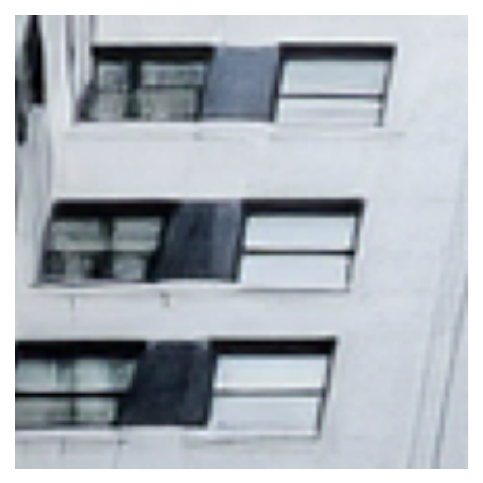} \\ \small LDL \cite{details_or_artifacts} \\ (21.86 / 0.133)
    \end{subfigure}
\end{subfigure}
\begin{subfigure}{0.16\textwidth}
    \begin{subfigure}{\textwidth}
        \includegraphics[width=\textwidth]{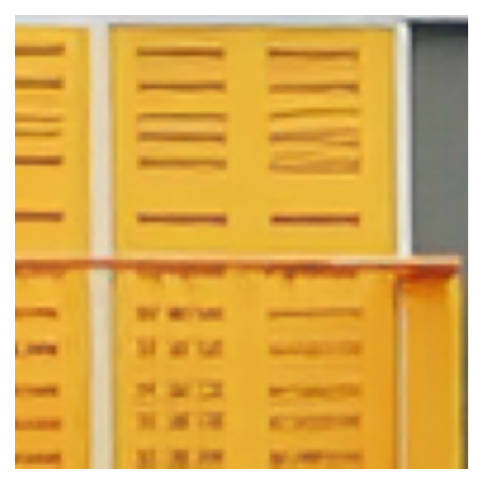} \\ \small FxSR \cite{fxsr} \\ (23.80 / 0.116)
    \end{subfigure}
            \begin{subfigure}{\textwidth}
        \includegraphics[width=\textwidth]{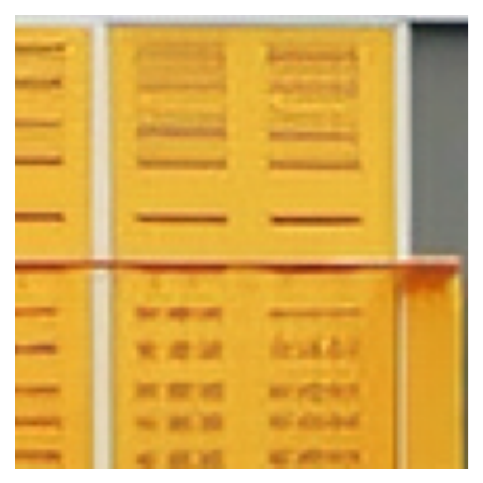} \\ \small PDASR \cite{PDASR} \\ (23.70 / 0.134)
    \end{subfigure}
    \begin{subfigure}{\textwidth}
        \includegraphics[width=\textwidth]{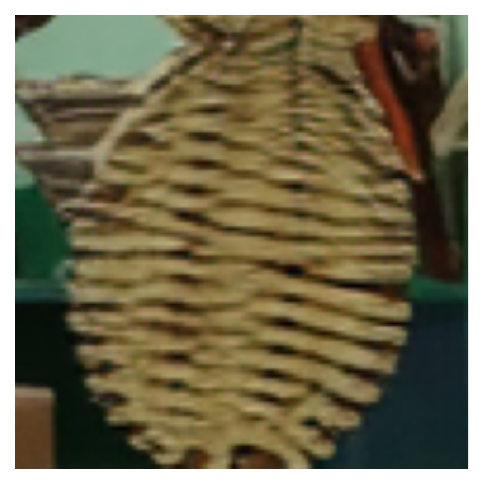} \\ \small FxSR \cite{fxsr} \\ (20.96 / 0.178)
    \end{subfigure}
            \begin{subfigure}{\textwidth}
        \includegraphics[width=\textwidth]{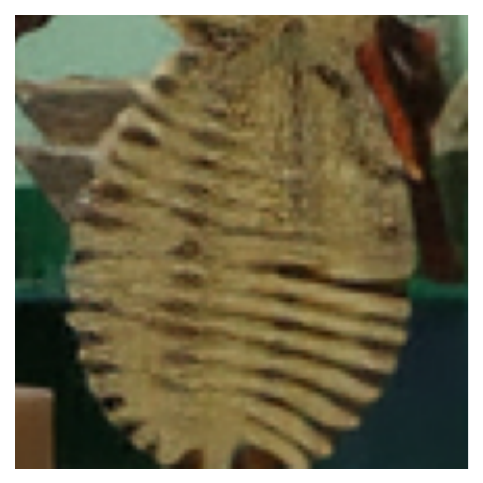} \\ \small PDASR \cite{PDASR} \\ (21.99 / 0.215)
    \end{subfigure}
    \begin{subfigure}{\textwidth}
        \includegraphics[width=\textwidth]{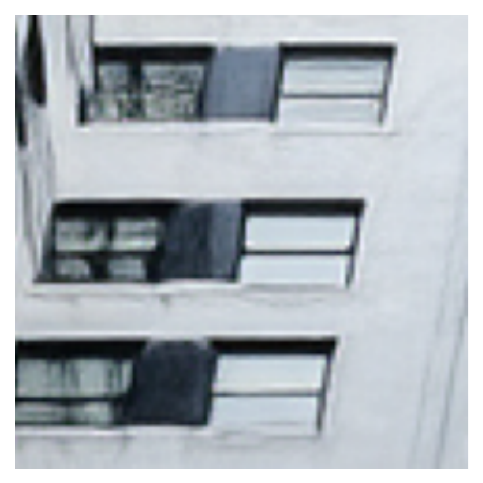} \\ \small FxSR \cite{fxsr} \\ (21.29 / 0.154)
    \end{subfigure}
            \begin{subfigure}{\textwidth}
        \includegraphics[width=\textwidth]{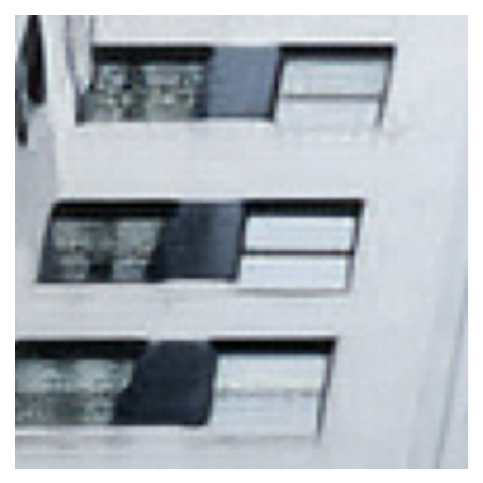} \\ \small PDASR \cite{PDASR} \\ (21.72 / 0.175)
    \end{subfigure}
\end{subfigure}
\begin{subfigure}{0.16\textwidth}
    \begin{subfigure}{\textwidth}
        \includegraphics[width=\textwidth]{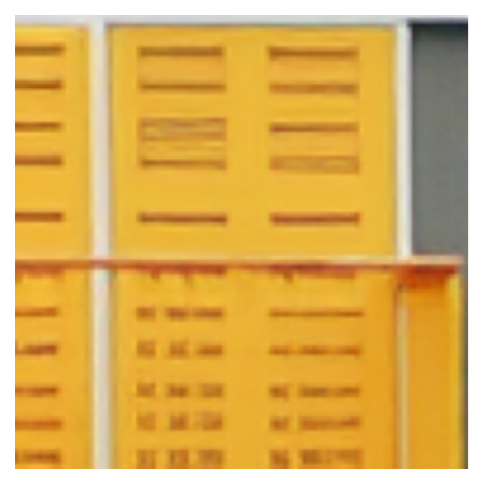} \\ \small SROOE \cite{srooe_Park_2023_CVPR} \\ (24.72 / 0.110)
    \end{subfigure}
    \begin{subfigure}{\textwidth}
        \includegraphics[width=\textwidth]{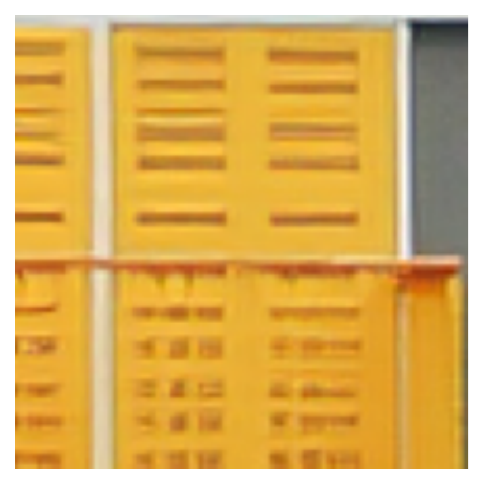} \\ \small  DualFormer \cite{dualformer_luo2023effectiveness} \\ (23.45 / 0.127)
    \end{subfigure}
    \begin{subfigure}{\textwidth}
        \includegraphics[width=\textwidth]{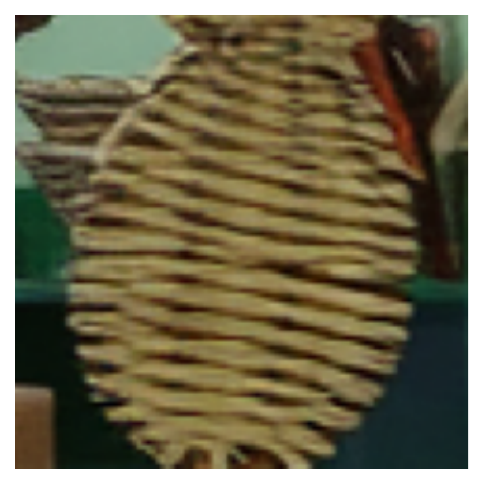} \\ \small SROOE \cite{srooe_Park_2023_CVPR} \\ (20.47 / 0.201)
    \end{subfigure}
    \begin{subfigure}{\textwidth}
        \includegraphics[width=\textwidth]{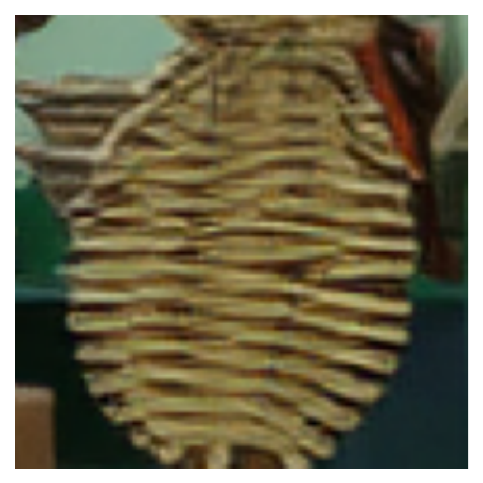} \\ \small  DualFormer \cite{dualformer_luo2023effectiveness} \\ (20.15 / 0.203)
    \end{subfigure}
    \begin{subfigure}{\textwidth}
        \includegraphics[width=\textwidth]{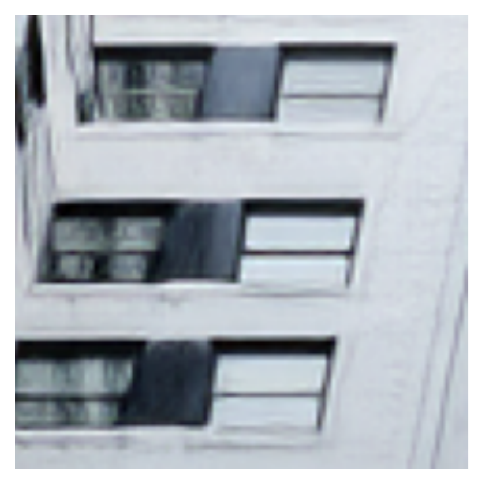} \\ \small SROOE \cite{srooe_Park_2023_CVPR} \\ (21.61 / 0.172)
    \end{subfigure}
    \begin{subfigure}{\textwidth}
        \includegraphics[width=\textwidth]{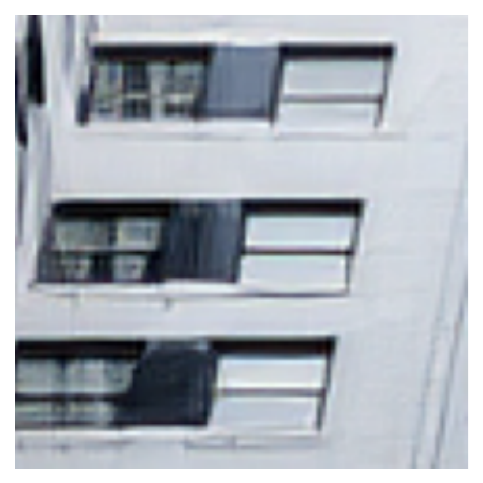} \\ \small  DualFormer \cite{dualformer_luo2023effectiveness} \\ (20.82 / 0.159)
    \end{subfigure}
\end{subfigure}
\begin{subfigure}{0.16\textwidth}
    \begin{subfigure}{\textwidth}
        \includegraphics[width=\textwidth]{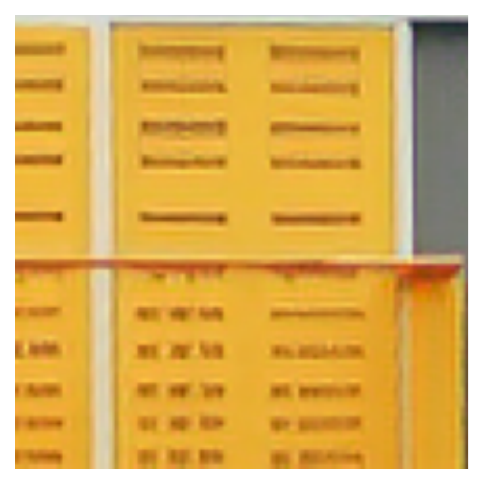} \\ \small WGSR (Ours) \\(24.57 / 0.129)
    \end{subfigure}
        \begin{subfigure}{\textwidth}
        \includegraphics[width=\textwidth]{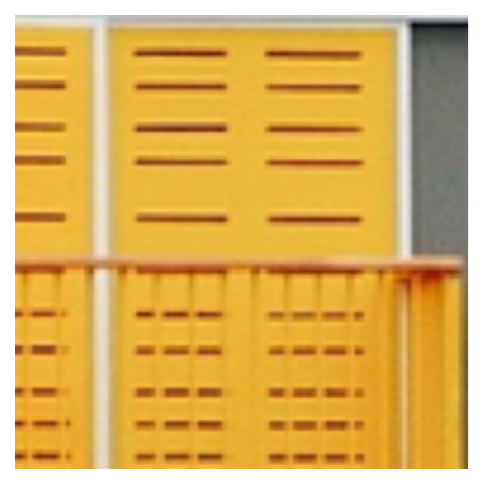} \\ \small HR (img-836)\\ (PSNR$\uparrow$ / DISTS$\downarrow$\cite{dists})
    \end{subfigure}
    \begin{subfigure}{\textwidth}
        \includegraphics[width=\textwidth]{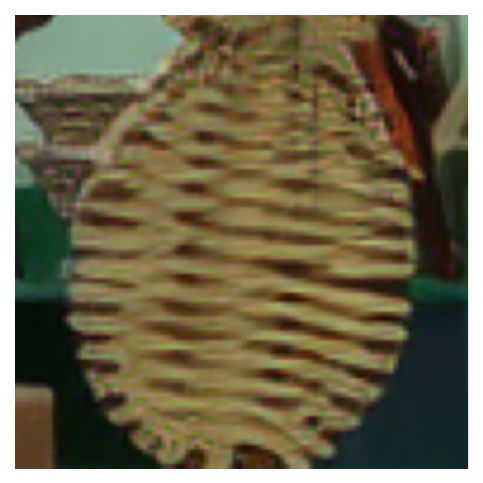} \\ \small WGSR (Ours) \\(21.60 / 0.171)
    \end{subfigure}
        \begin{subfigure}{\textwidth}
        \includegraphics[width=\textwidth]{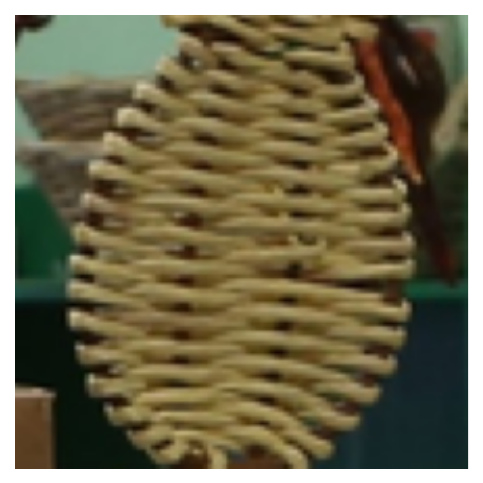} \\ \small HR (img-837)\\ (PSNR$\uparrow$ / DISTS$\downarrow$\cite{dists})
    \end{subfigure}
    \begin{subfigure}{\textwidth}
        \includegraphics[width=\textwidth]{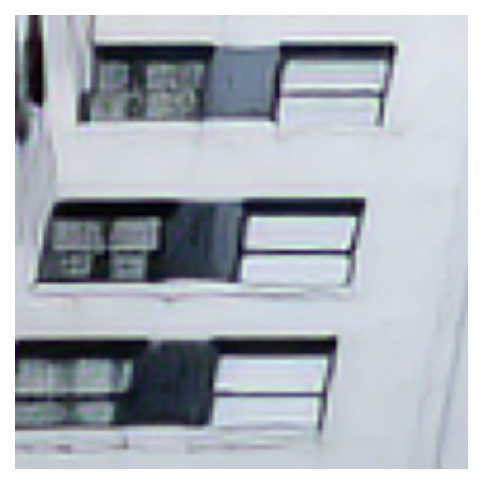} \\ \small WGSR (Ours) \\(21.75 / 0.174)
    \end{subfigure}
        \begin{subfigure}{\textwidth}
        \includegraphics[width=\textwidth]{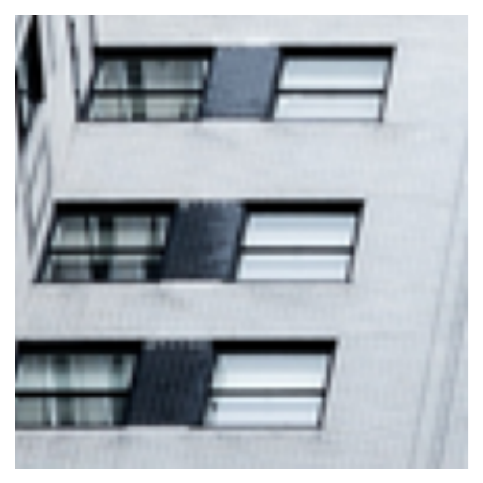} \\ \small HR (img-846)\\ (PSNR$\uparrow$ / DISTS$\downarrow$\cite{dists})
    \end{subfigure}
\end{subfigure} 
\caption{Visual comparison of the proposed wavelet-guided perceptual optimization method with the state-of-the-art for $\times$4 SR on natural images from DIV2K validation set \cite{Agustsson_2017_CVPR_Workshops}.}
\label{fig:supp_div2k3} 
\end{figure*}

\begin{figure*}
\centering
\begin{subfigure}{0.16\textwidth}
     \begin{subfigure}{\textwidth}
        \includegraphics[width=\textwidth]{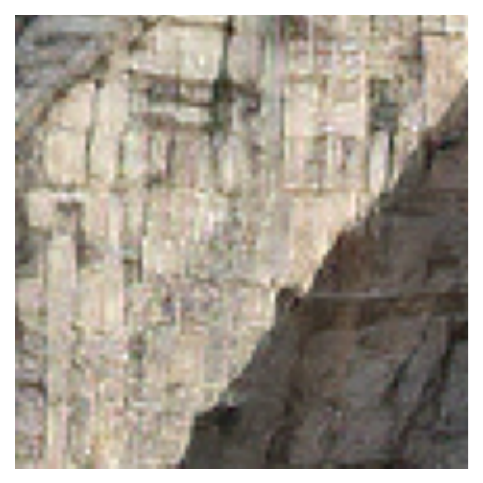} \\ \small ESRGAN-FS \cite{freq_sep} \\ (20.64 / 0.193)
    \end{subfigure}
    \begin{subfigure}{\textwidth}
        \includegraphics[width=\textwidth]{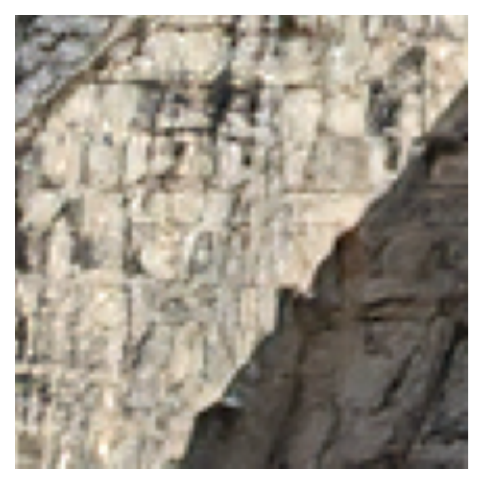} \\ \small ESRGAN+ \cite{esrganplus} \\ (19.61 / 0.225)
    \end{subfigure}
     \begin{subfigure}{\textwidth}
        \includegraphics[width=\textwidth]{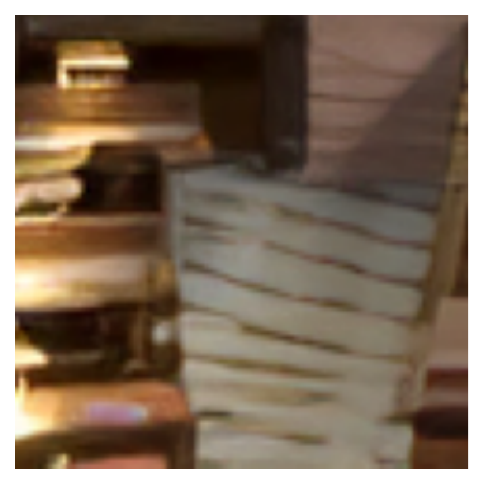} \\ \small ESRGAN-FS \cite{freq_sep} \\ (24.45 / 0.189)
    \end{subfigure}
    \begin{subfigure}{\textwidth}
        \includegraphics[width=\textwidth]{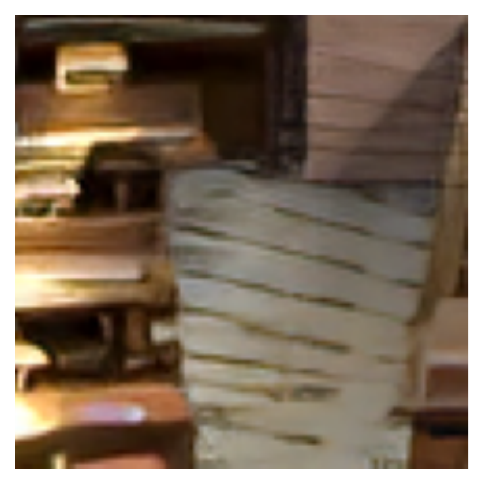} \\ \small ESRGAN+ \cite{esrganplus} \\ (22.91 / 0.178)
    \end{subfigure}
     \begin{subfigure}{\textwidth}
        \includegraphics[width=\textwidth]{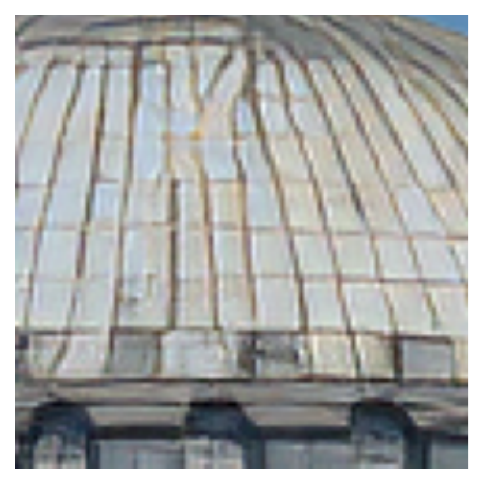} \\ \small ESRGAN-FS \cite{freq_sep} \\ (20.85 / 0.255)
    \end{subfigure}
    \begin{subfigure}{\textwidth}
        \includegraphics[width=\textwidth]{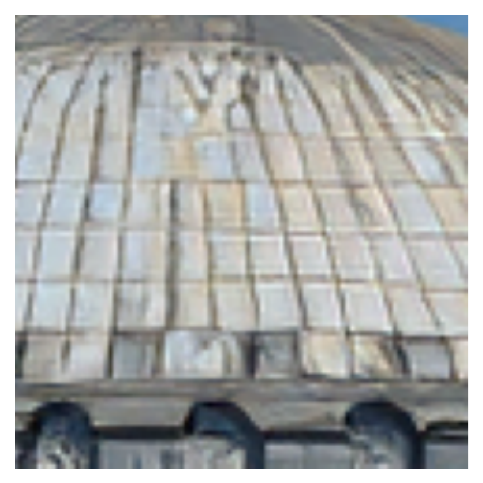} \\ \small ESRGAN+ \cite{esrganplus} \\ (21.07 / 0.212)
    \end{subfigure}
\end{subfigure}
\begin{subfigure}{0.16\textwidth}
    \begin{subfigure}{\textwidth}
        \includegraphics[width=\textwidth]{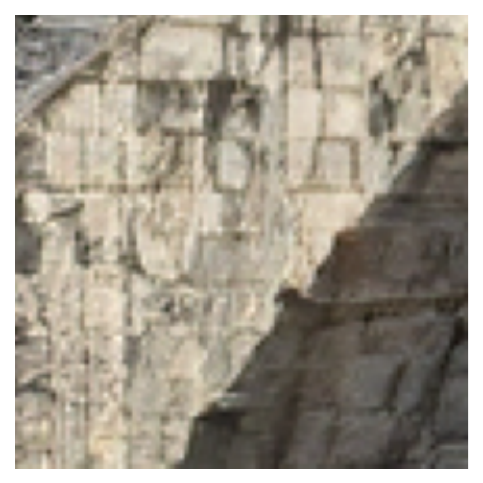} \\ \small SPSR \cite{ma_SPSR} \\ (20.74 / 0.171)
    \end{subfigure}
    \begin{subfigure}{\textwidth}
        \includegraphics[width=\textwidth]{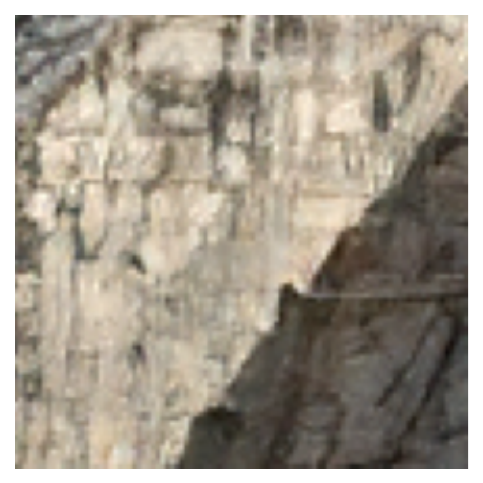} \\ \small RankSRGAN \cite{zhang2021ranksrgan} \\ (21.08 / 0.203)
    \end{subfigure}
    \begin{subfigure}{\textwidth}
        \includegraphics[width=\textwidth]{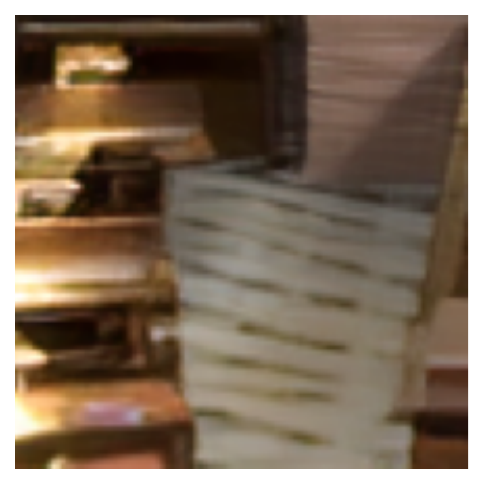} \\ \small SPSR \cite{ma_SPSR} \\ (23.88 / 0.194)
    \end{subfigure}
    \begin{subfigure}{\textwidth}
        \includegraphics[width=\textwidth]{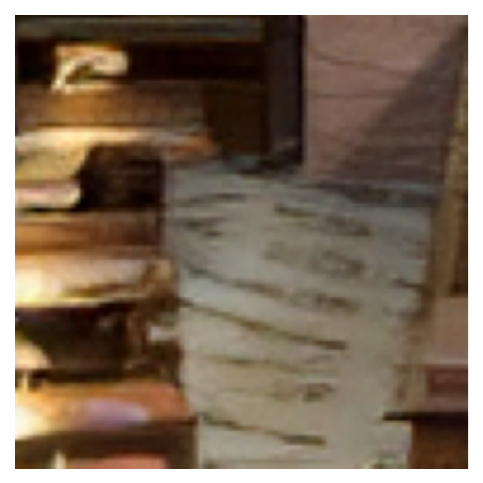} \\ \small RankSRGAN \cite{zhang2021ranksrgan} \\ (23.38 / 0.203)
    \end{subfigure}
    \begin{subfigure}{\textwidth}
        \includegraphics[width=\textwidth]{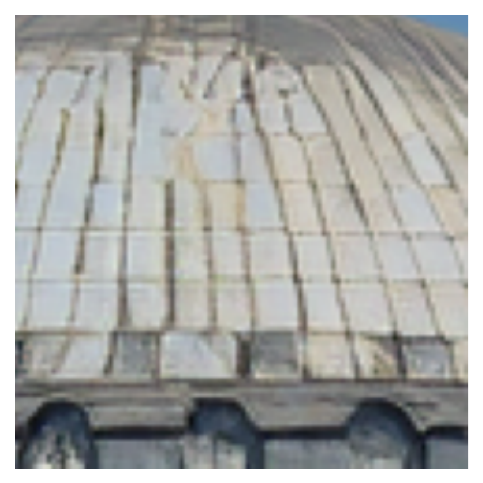} \\ \small SPSR \cite{ma_SPSR} \\ (22.11 / 0.227)
    \end{subfigure}
    \begin{subfigure}{\textwidth}
        \includegraphics[width=\textwidth]{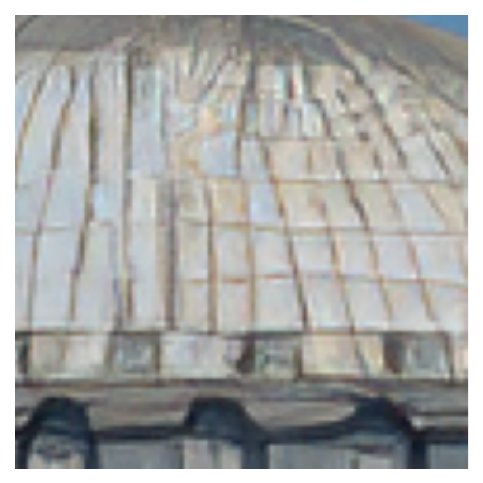} \\ \small RankSRGAN \cite{zhang2021ranksrgan} \\ (21.58 / 0.234)
    \end{subfigure}
\end{subfigure}
\begin{subfigure}{0.16\textwidth}
    \begin{subfigure}{\textwidth}
        \includegraphics[width=\textwidth]{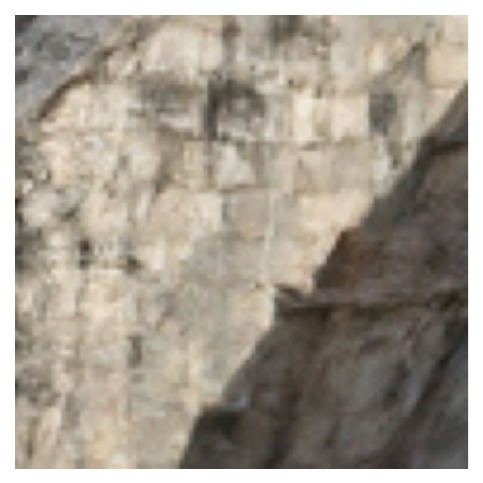} \\\small  SRFlow-DA \cite{jo2021srflowda} \\ (22.36 / 0.216)
    \end{subfigure}
    \begin{subfigure}{\textwidth}
        \includegraphics[width=\textwidth]{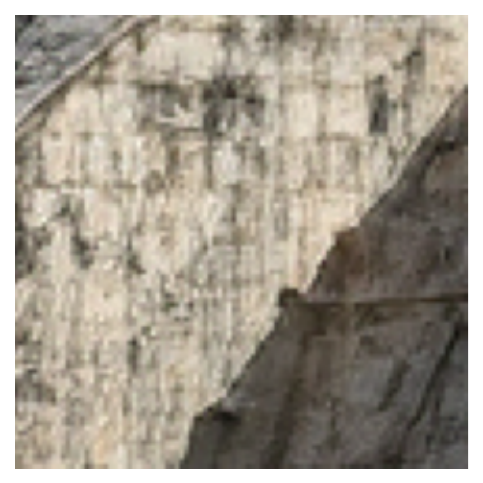} \\ \small LDL \cite{details_or_artifacts} \\ (20.67 / 0.188)
    \end{subfigure}
    \begin{subfigure}{\textwidth}
        \includegraphics[width=\textwidth]{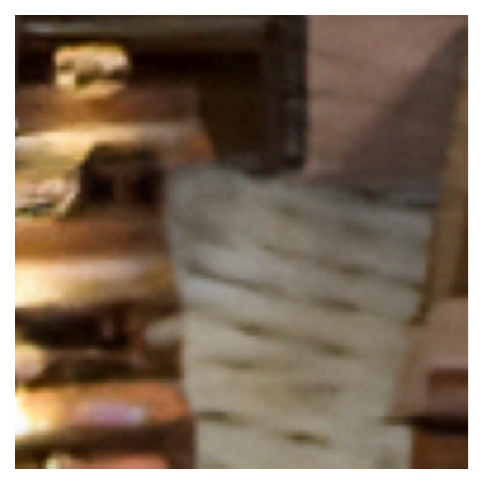} \\\small  SRFlow-DA \cite{jo2021srflowda} \\ (24.58 / 0.230)
    \end{subfigure}
    \begin{subfigure}{\textwidth}
        \includegraphics[width=\textwidth]{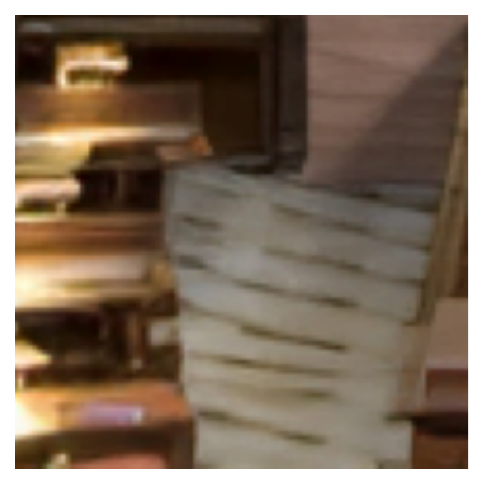} \\ \small LDL \cite{details_or_artifacts} \\ (24.98 / 0.182)
    \end{subfigure}
    \begin{subfigure}{\textwidth}
        \includegraphics[width=\textwidth]{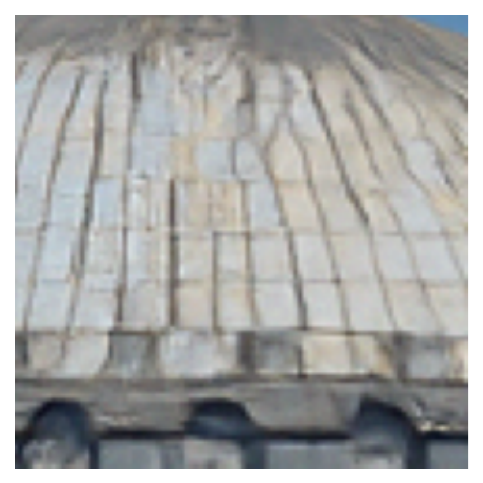} \\\small  SRFlow-DA \cite{jo2021srflowda} \\ (22.22 / 0.225)
    \end{subfigure}
    \begin{subfigure}{\textwidth}
        \includegraphics[width=\textwidth]{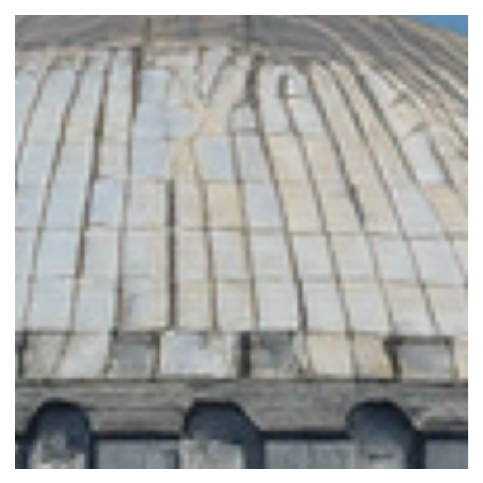} \\ \small LDL \cite{details_or_artifacts} \\ (22.58 / 0.229)
    \end{subfigure}
\end{subfigure}
\begin{subfigure}{0.16\textwidth}
    \begin{subfigure}{\textwidth}
        \includegraphics[width=\textwidth]{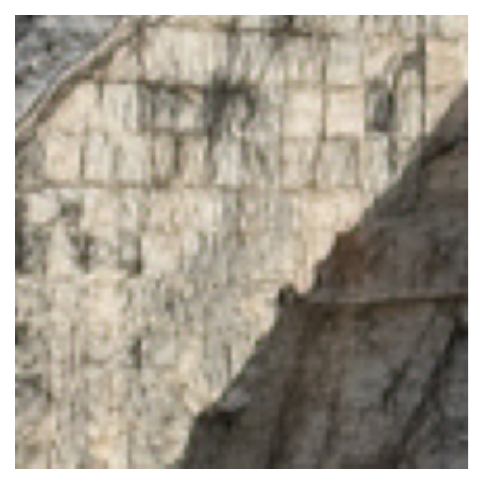} \\ \small FxSR \cite{fxsr} \\ (21.43 / 0.185)
    \end{subfigure}
            \begin{subfigure}{\textwidth}
        \includegraphics[width=\textwidth]{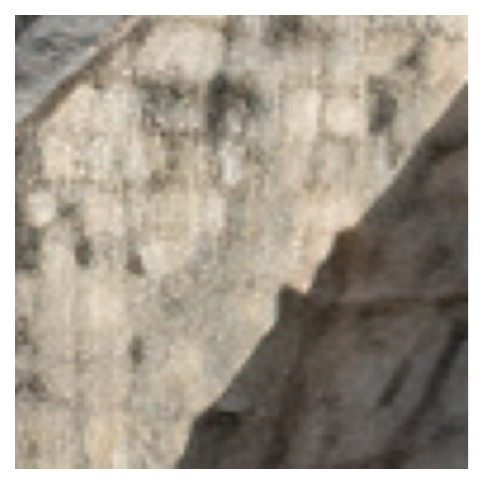} \\ \small PDASR \cite{PDASR} \\ (22.76 / 0.235)
    \end{subfigure}
    \begin{subfigure}{\textwidth}
        \includegraphics[width=\textwidth]{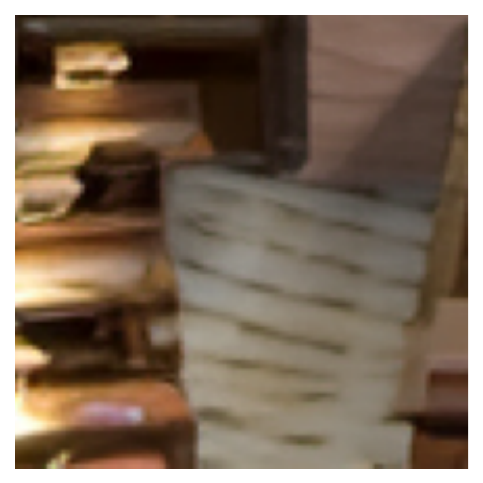} \\ \small FxSR \cite{fxsr} \\ (25.04 / 0.176)
    \end{subfigure}
            \begin{subfigure}{\textwidth}
        \includegraphics[width=\textwidth]{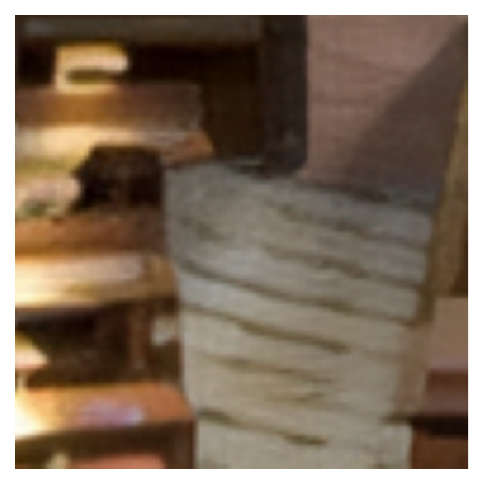} \\ \small PDASR \cite{PDASR} \\ (25.33 / 0.212)
    \end{subfigure}
    \begin{subfigure}{\textwidth}
        \includegraphics[width=\textwidth]{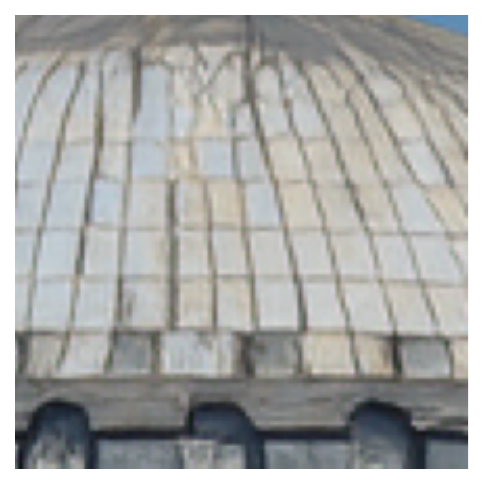} \\ \small FxSR \cite{fxsr} \\ (22.70 / 0.205)
    \end{subfigure}
            \begin{subfigure}{\textwidth}
        \includegraphics[width=\textwidth]{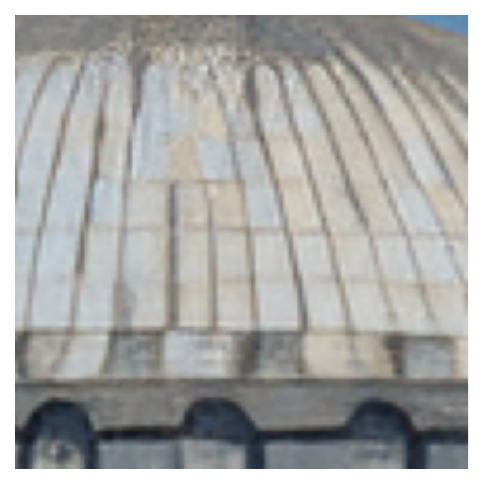} \\ \small PDASR \cite{PDASR} \\ (23.23 / 0.234)
    \end{subfigure}
\end{subfigure}
\begin{subfigure}{0.16\textwidth}
    \begin{subfigure}{\textwidth}
        \includegraphics[width=\textwidth]{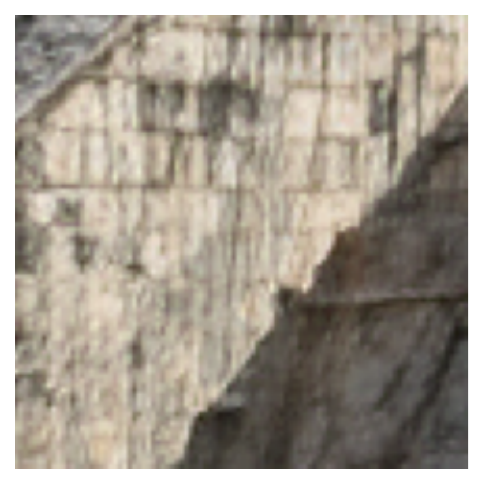} \\ \small SROOE \cite{srooe_Park_2023_CVPR} \\ (21.48 / 0.176)
    \end{subfigure}
    \begin{subfigure}{\textwidth}
        \includegraphics[width=\textwidth]{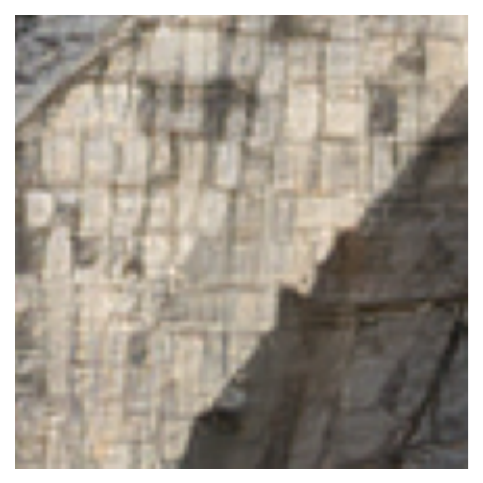} \\ \small  DualFormer \cite{dualformer_luo2023effectiveness} \\ (22.11 / 0.178)
    \end{subfigure}
    \begin{subfigure}{\textwidth}
        \includegraphics[width=\textwidth]{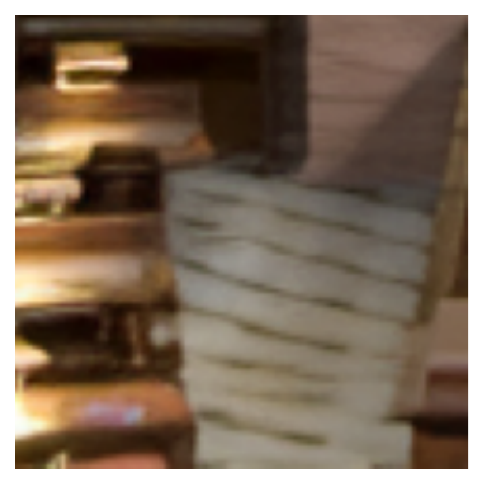} \\ \small SROOE \cite{srooe_Park_2023_CVPR} \\ (25.03 / 0.190)
    \end{subfigure}
    \begin{subfigure}{\textwidth}
        \includegraphics[width=\textwidth]{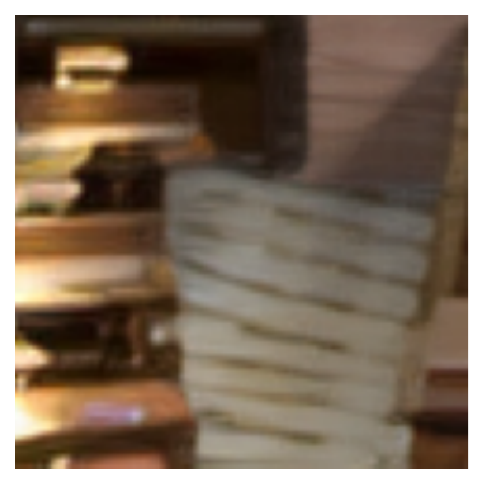} \\ \small  DualFormer \cite{dualformer_luo2023effectiveness} \\ (24.95 / 0.206)
    \end{subfigure}
    \begin{subfigure}{\textwidth}
        \includegraphics[width=\textwidth]{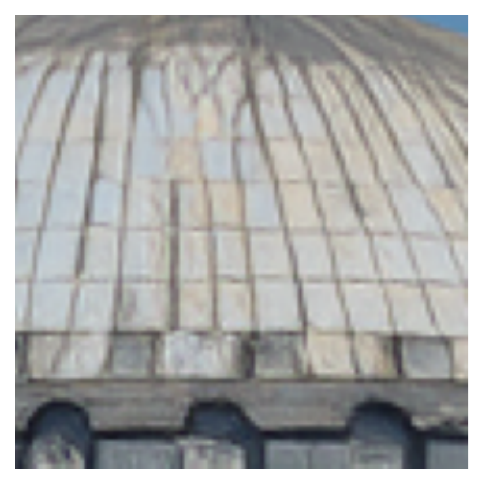} \\ \small SROOE \cite{srooe_Park_2023_CVPR} \\ (22.72 / 0.198)
    \end{subfigure}
    \begin{subfigure}{\textwidth}
        \includegraphics[width=\textwidth]{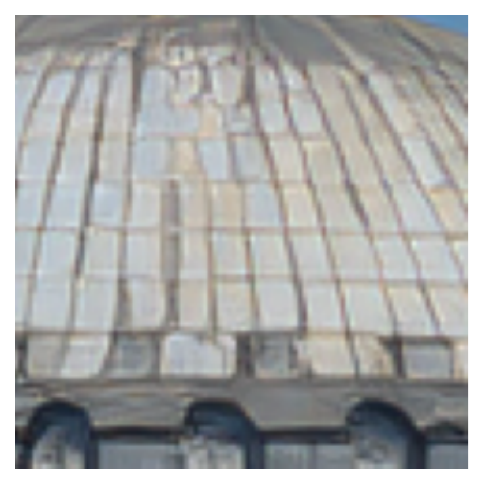} \\ \small  DualFormer \cite{dualformer_luo2023effectiveness} \\ (22.70 / 0.210)
    \end{subfigure}
\end{subfigure}
\begin{subfigure}{0.16\textwidth}
    \begin{subfigure}{\textwidth}
        \includegraphics[width=\textwidth]{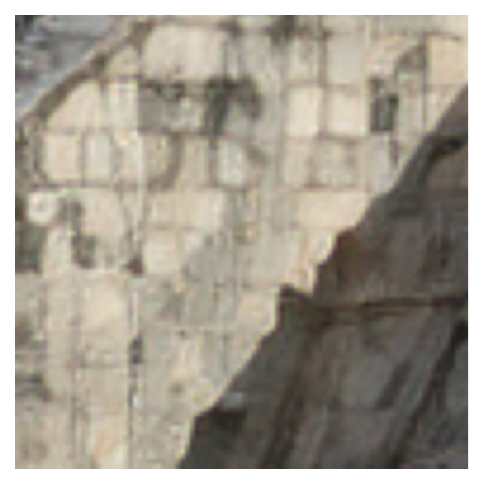} \\ \small WGSR (Ours) \\(22.78 / 0.145)
    \end{subfigure}
        \begin{subfigure}{\textwidth}
        \includegraphics[width=\textwidth]{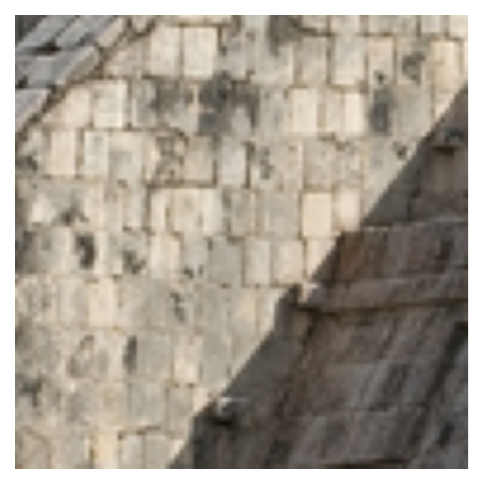} \\ \small HR (img-881)\\ (PSNR$\uparrow$ / DISTS$\downarrow$\cite{dists})
    \end{subfigure}
    \begin{subfigure}{\textwidth}
        \includegraphics[width=\textwidth]{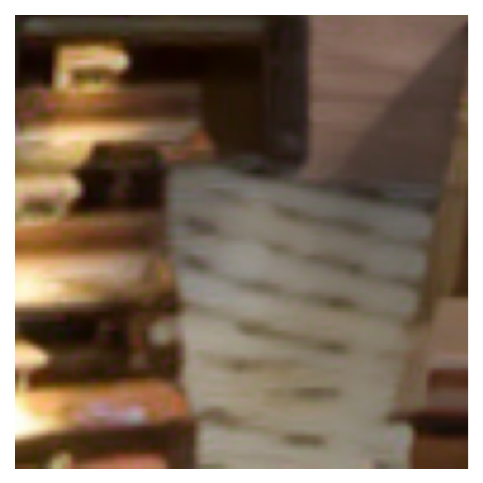} \\ \small WGSR (Ours) \\(25.91 / 0.212)
    \end{subfigure}
        \begin{subfigure}{\textwidth}
        \includegraphics[width=\textwidth]{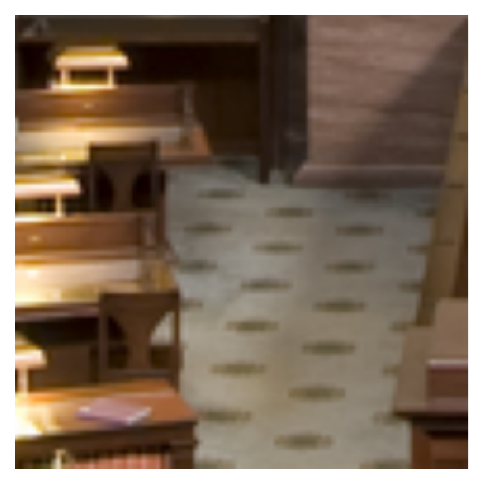} \\ \small HR (img-884)\\ (PSNR$\uparrow$ / DISTS$\downarrow$\cite{dists})
    \end{subfigure}
    \begin{subfigure}{\textwidth}
        \includegraphics[width=\textwidth]{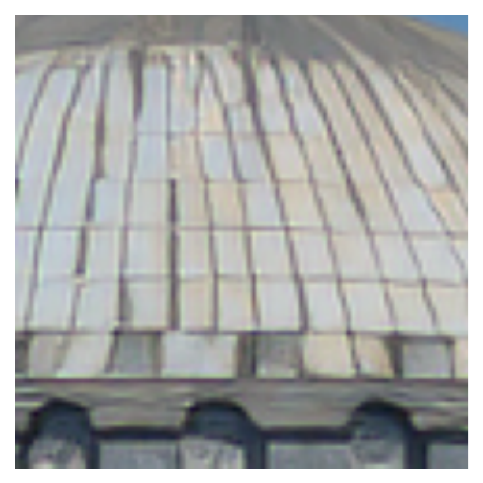} \\ \small WGSR (Ours) \\ (22.98 / 0.222)
    \end{subfigure}
        \begin{subfigure}{\textwidth}
        \includegraphics[width=\textwidth]{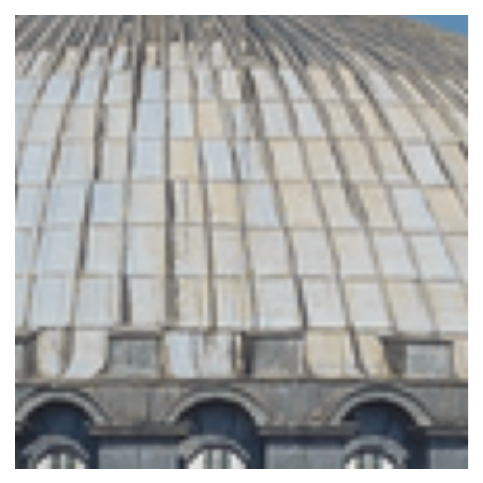} \\ \small HR (img-890)\\ (PSNR$\uparrow$ / DISTS$\downarrow$\cite{dists})
    \end{subfigure}
\end{subfigure} 
\caption{Visual comparison of the proposed wavelet-guided perceptual optimization method with the state-of-the-art for $\times$4 SR on natural images from DIV2K validation set \cite{Agustsson_2017_CVPR_Workshops}.}
\label{fig:supp_div2k4} 
\end{figure*}

\begin{figure*}
\centering
\begin{subfigure}{0.16\textwidth}
     \begin{subfigure}{\textwidth}
        \includegraphics[width=\textwidth]{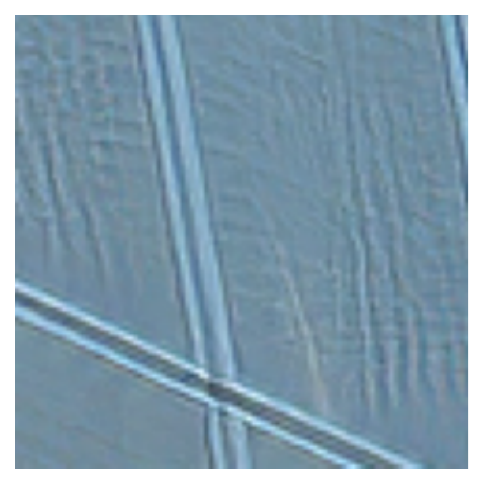} \\ \small ESRGAN-FS \cite{freq_sep} \\ (25.67 / 0.257)
    \end{subfigure}
    \begin{subfigure}{\textwidth}
        \includegraphics[width=\textwidth]{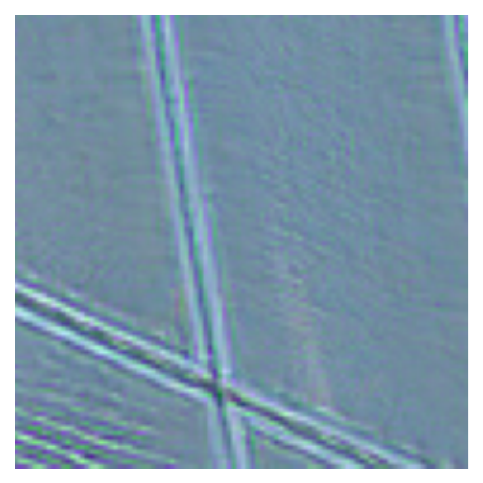} \\ \small ESRGAN+ \cite{esrganplus} \\ (26.19 / 0.227)
    \end{subfigure}
     \begin{subfigure}{\textwidth}
        \includegraphics[width=\textwidth]{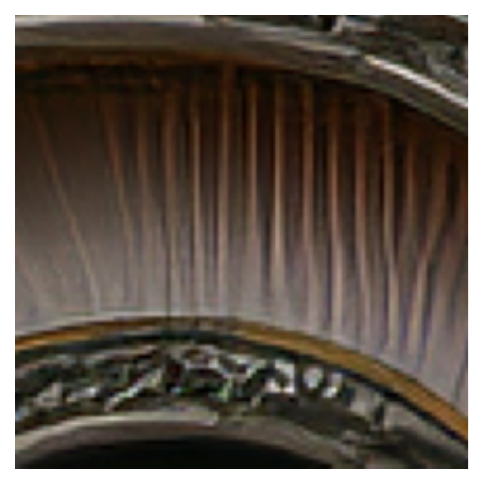} \\ \small ESRGAN-FS \cite{freq_sep} \\ (22.46 / 0.221)
    \end{subfigure}
    \begin{subfigure}{\textwidth}
        \includegraphics[width=\textwidth]{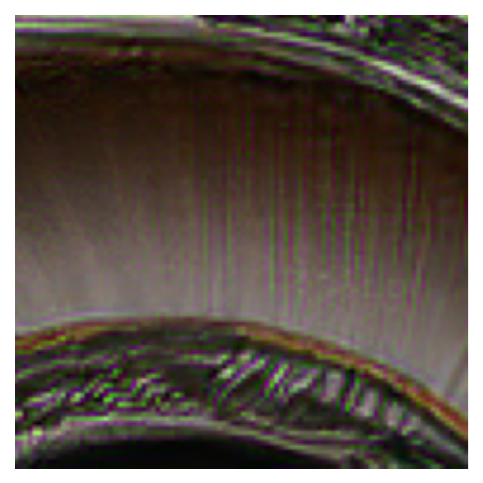} \\ \small ESRGAN+ \cite{esrganplus} \\ (23.09 / 0.237)
    \end{subfigure}
     \begin{subfigure}{\textwidth}
        \includegraphics[width=\textwidth]{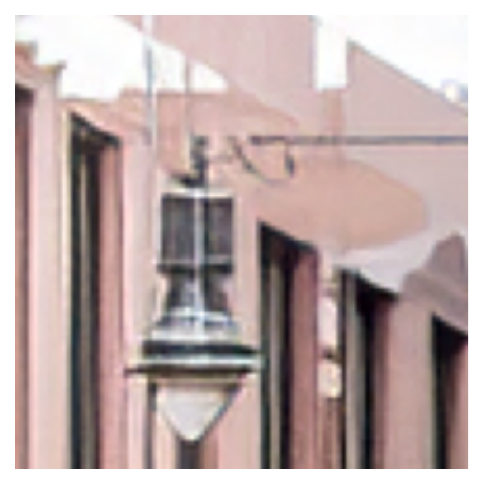} \\ \small ESRGAN-FS \cite{freq_sep} \\ (20.72 / 0.149)
    \end{subfigure}
    \begin{subfigure}{\textwidth}
        \includegraphics[width=\textwidth]{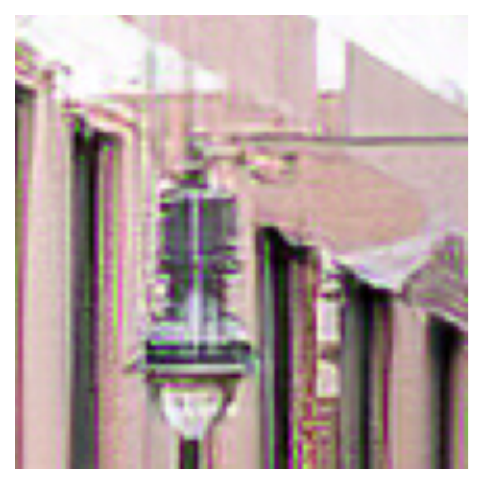} \\ \small ESRGAN+ \cite{esrganplus} \\ (20.25 / 0.191)
    \end{subfigure}
\end{subfigure}
\begin{subfigure}{0.16\textwidth}
    \begin{subfigure}{\textwidth}
        \includegraphics[width=\textwidth]{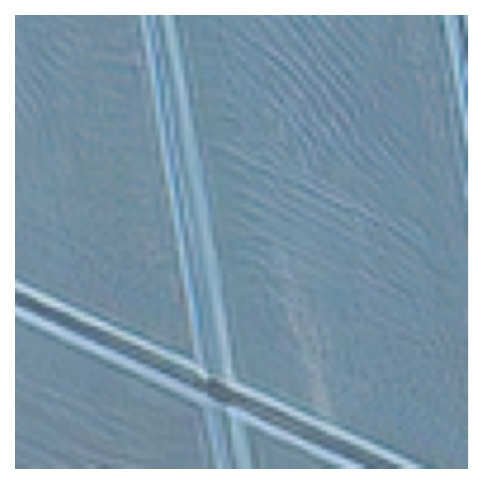} \\ \small SPSR \cite{ma_SPSR} \\ (25.60 / 0.209)
    \end{subfigure}
    \begin{subfigure}{\textwidth}
        \includegraphics[width=\textwidth]{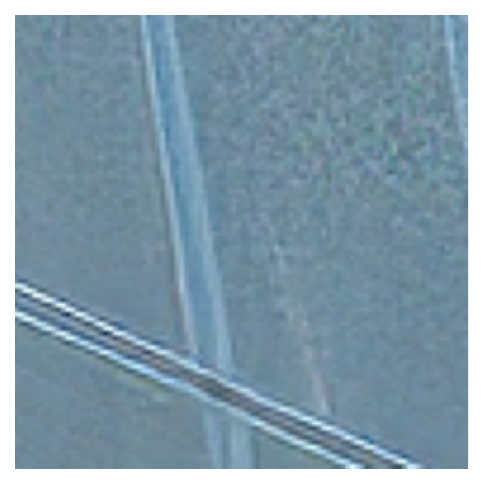} \\ \small RankSRGAN \cite{zhang2021ranksrgan} \\ (23.60 / 0.231)
    \end{subfigure}
    \begin{subfigure}{\textwidth}
        \includegraphics[width=\textwidth]{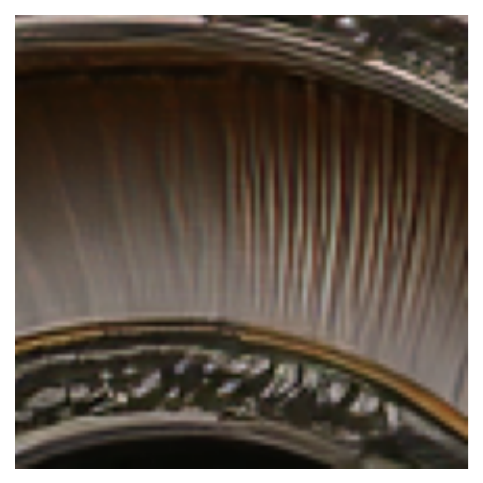} \\ \small SPSR \cite{ma_SPSR} \\ (22.93 / 0.228)
    \end{subfigure}
    \begin{subfigure}{\textwidth}
        \includegraphics[width=\textwidth]{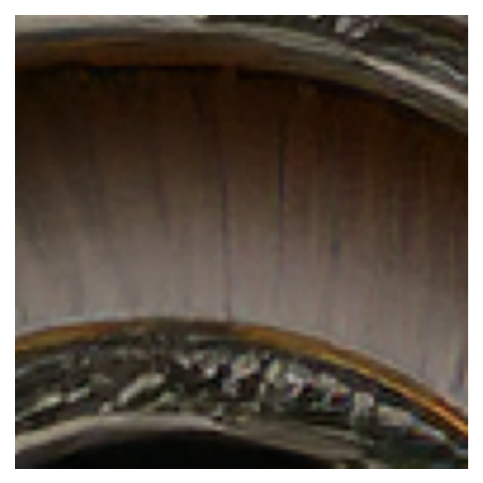} \\ \small RankSRGAN \cite{zhang2021ranksrgan} \\ (24.12 / 0.163)
    \end{subfigure}
    \begin{subfigure}{\textwidth}
        \includegraphics[width=\textwidth]{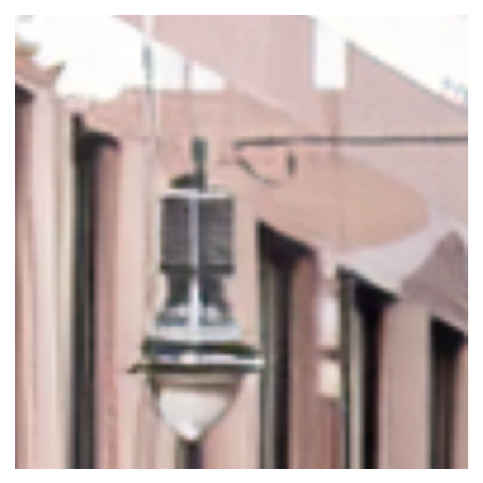} \\ \small SPSR \cite{ma_SPSR} \\ (22.17 / 0.149)
    \end{subfigure}
    \begin{subfigure}{\textwidth}
        \includegraphics[width=\textwidth]{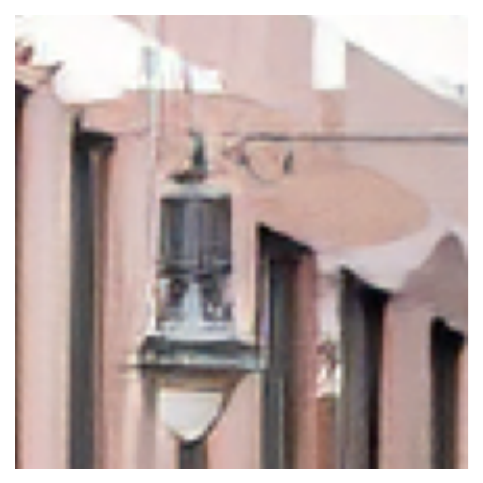} \\ \small RankSRGAN \cite{zhang2021ranksrgan} \\ (21.49 / 0.159)
    \end{subfigure}
\end{subfigure}
\begin{subfigure}{0.16\textwidth}
    \begin{subfigure}{\textwidth}
        \includegraphics[width=\textwidth]{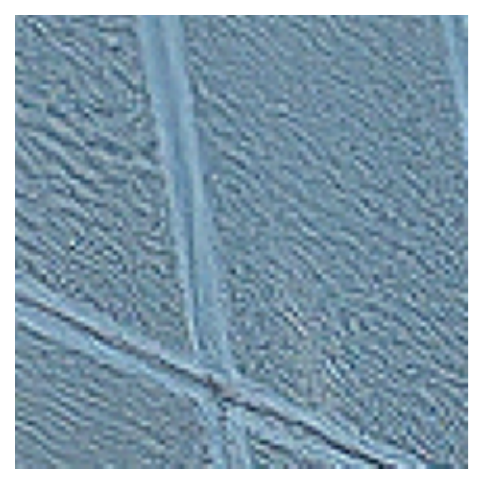} \\\small  SRFlow-DA \cite{jo2021srflowda} \\ (20.26 / 0.325)
    \end{subfigure}
    \begin{subfigure}{\textwidth}
        \includegraphics[width=\textwidth]{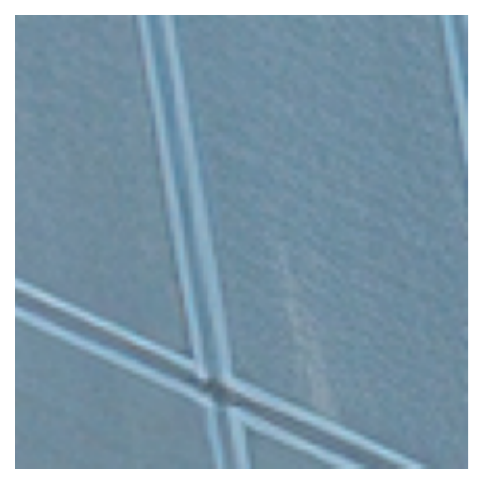} \\ \small LDL \cite{details_or_artifacts} \\ (27.65 / 0.160)
    \end{subfigure}
    \begin{subfigure}{\textwidth}
        \includegraphics[width=\textwidth]{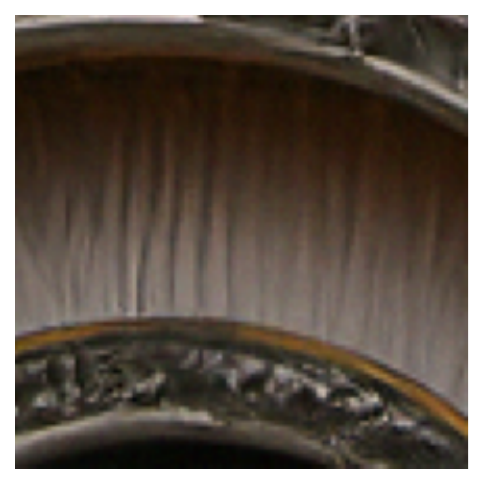} \\\small  SRFlow-DA \cite{jo2021srflowda} \\ (25.15 / 0.196)
    \end{subfigure}
    \begin{subfigure}{\textwidth}
        \includegraphics[width=\textwidth]{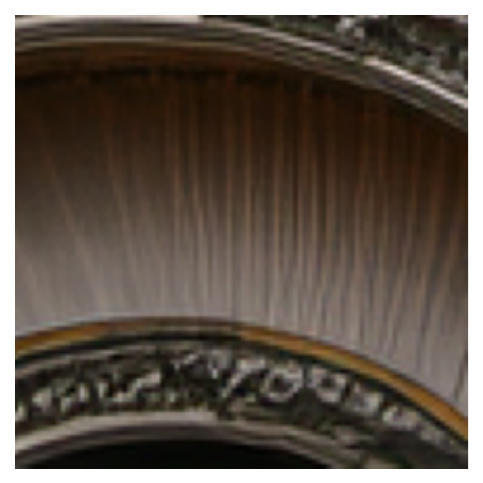} \\ \small LDL \cite{details_or_artifacts} \\ (24.50 / 0.211)
    \end{subfigure}
    \begin{subfigure}{\textwidth}
        \includegraphics[width=\textwidth]{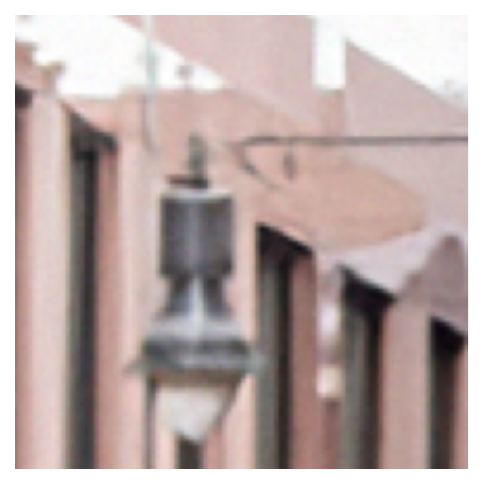} \\\small  SRFlow-DA \cite{jo2021srflowda} \\ (24.77 / 0.175)
    \end{subfigure}
    \begin{subfigure}{\textwidth}
        \includegraphics[width=\textwidth]{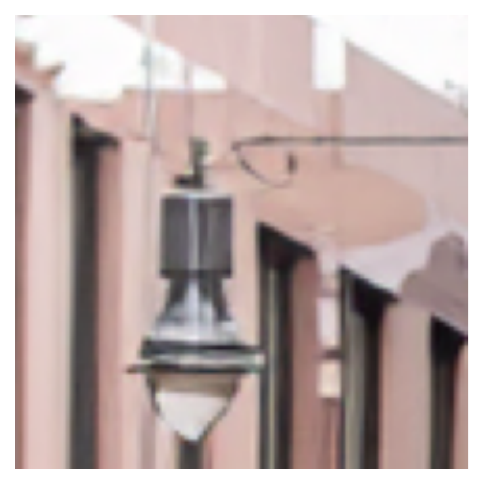} \\ \small LDL \cite{details_or_artifacts} \\ (23.19 / 0.154)
    \end{subfigure}
\end{subfigure}
\begin{subfigure}{0.16\textwidth}
    \begin{subfigure}{\textwidth}
        \includegraphics[width=\textwidth]{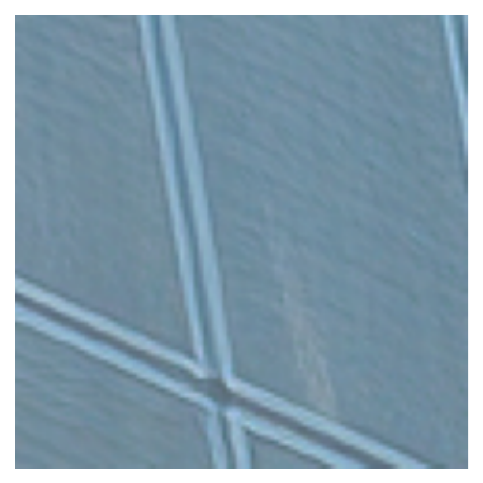} \\ \small FxSR \cite{fxsr} \\ (28.91 / 0.228)
    \end{subfigure}
            \begin{subfigure}{\textwidth}
        \includegraphics[width=\textwidth]{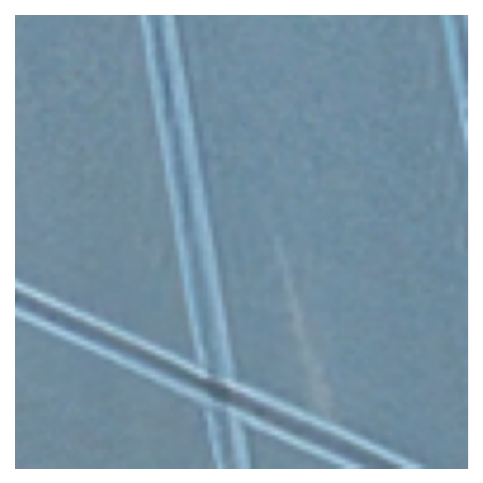} \\ \small PDASR \cite{PDASR} \\ (28.22 / 0.190)
    \end{subfigure}
    \begin{subfigure}{\textwidth}
        \includegraphics[width=\textwidth]{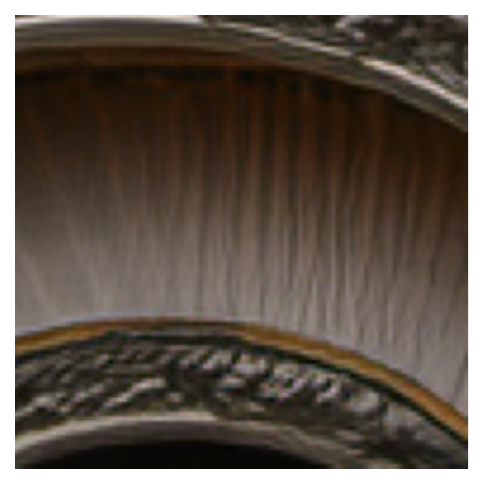} \\ \small FxSR \cite{fxsr} \\ (25.19 / 0.192)
    \end{subfigure}
            \begin{subfigure}{\textwidth}
        \includegraphics[width=\textwidth]{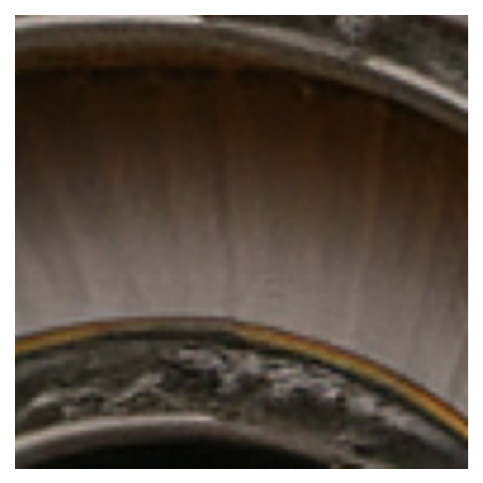} \\ \small PDASR \cite{PDASR} \\ (26.72 / 0.180)
    \end{subfigure}
    \begin{subfigure}{\textwidth}
        \includegraphics[width=\textwidth]{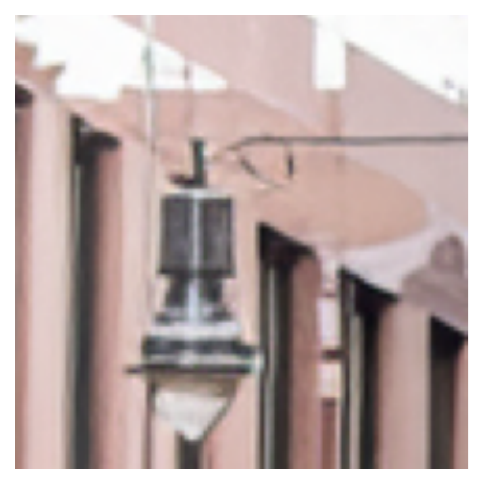} \\ \small FxSR \cite{fxsr} \\ (23.46 / 0.152)
    \end{subfigure}
            \begin{subfigure}{\textwidth}
        \includegraphics[width=\textwidth]{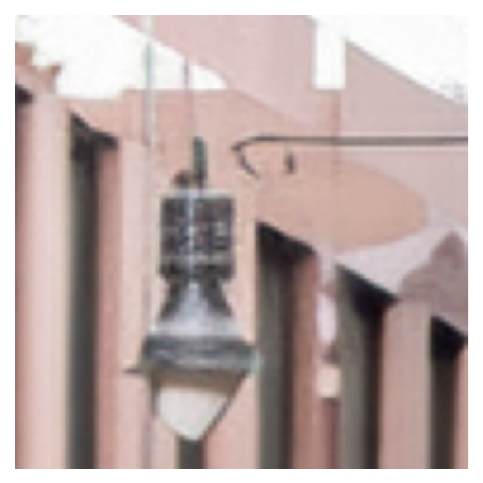} \\ \small PDASR \cite{PDASR} \\ (24.38 / 0.163)
    \end{subfigure}
\end{subfigure}
\begin{subfigure}{0.16\textwidth}
    \begin{subfigure}{\textwidth}
        \includegraphics[width=\textwidth]{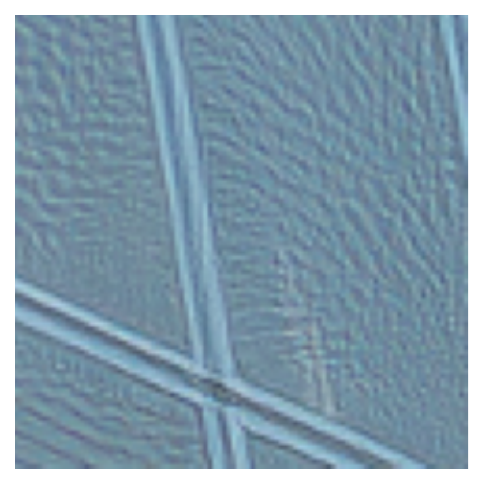} \\ \small SROOE \cite{srooe_Park_2023_CVPR} \\ (25.51 / 0.257)
    \end{subfigure}
    \begin{subfigure}{\textwidth}
        \includegraphics[width=\textwidth]{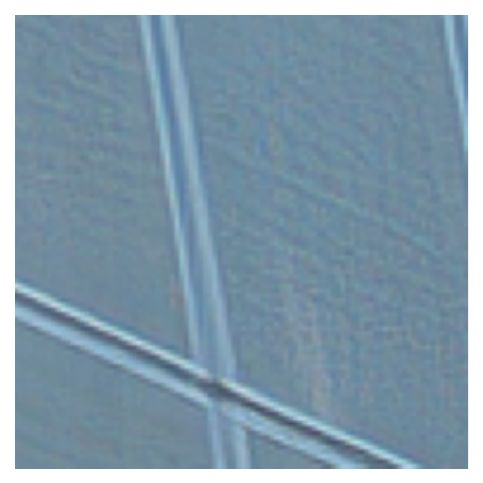} \\ \small  DualFormer \cite{dualformer_luo2023effectiveness} \\ (27.82 / 0.185)
    \end{subfigure}
    \begin{subfigure}{\textwidth}
        \includegraphics[width=\textwidth]{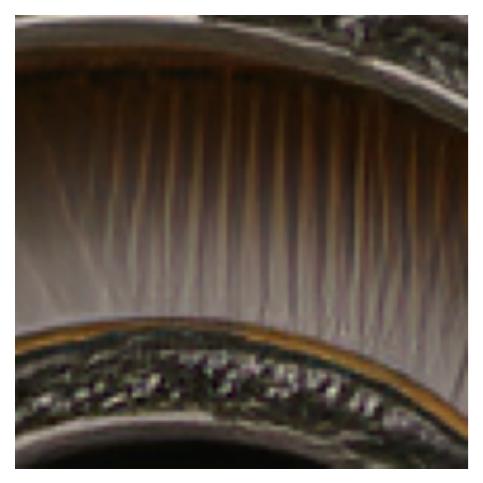} \\ \small SROOE \cite{srooe_Park_2023_CVPR} \\ (25.06 / 0.233)
    \end{subfigure}
    \begin{subfigure}{\textwidth}
        \includegraphics[width=\textwidth]{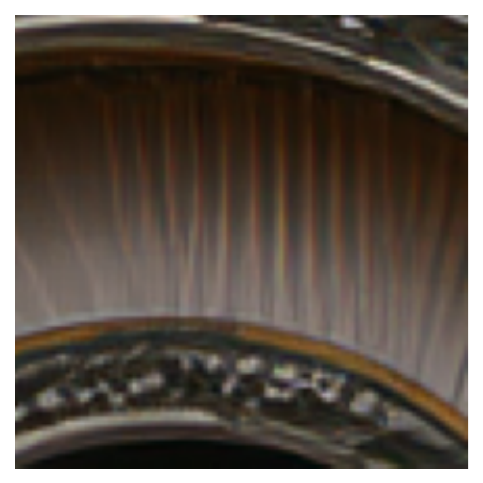} \\ \small  DualFormer \cite{dualformer_luo2023effectiveness} \\ (25.86 / 0.188)
    \end{subfigure}
    \begin{subfigure}{\textwidth}
        \includegraphics[width=\textwidth]{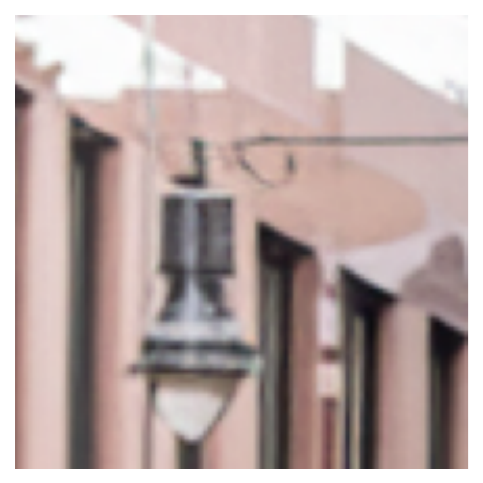} \\ \small SROOE \cite{srooe_Park_2023_CVPR} \\ (24.62 / 0.170)
    \end{subfigure}
    \begin{subfigure}{\textwidth}
        \includegraphics[width=\textwidth]{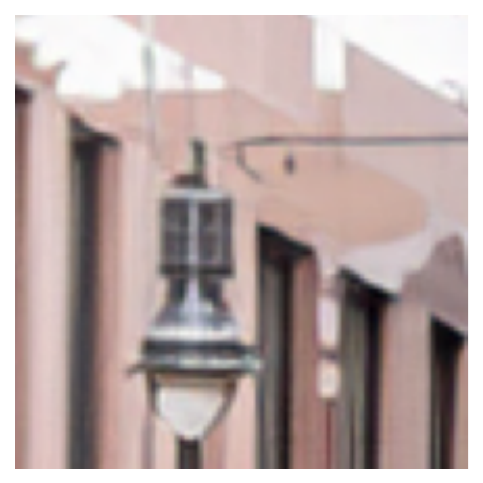} \\ \small  DualFormer \cite{dualformer_luo2023effectiveness} \\ (24.08 / 0.149)
    \end{subfigure}
\end{subfigure}
\begin{subfigure}{0.16\textwidth}
    \begin{subfigure}{\textwidth}
        \includegraphics[width=\textwidth]{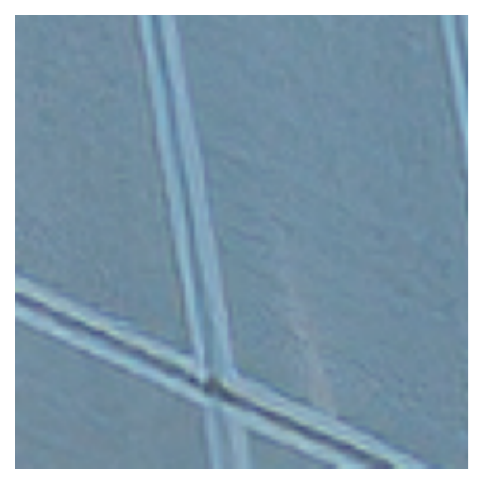} \\ \small WGSR (Ours) \\ (28.91 / 0.173)
    \end{subfigure}
        \begin{subfigure}{\textwidth}
        \includegraphics[width=\textwidth]{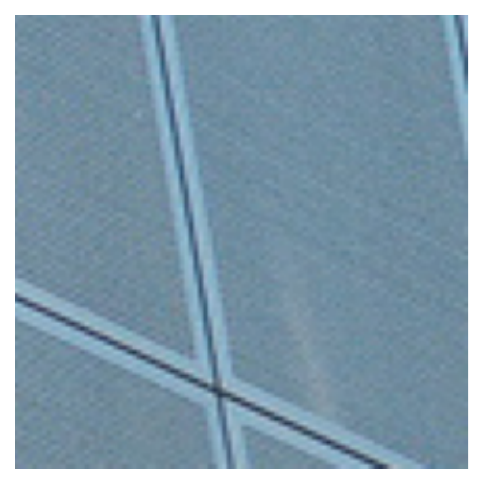} \\ \small HR (img-26)\\ (PSNR$\uparrow$ / DISTS$\downarrow$\cite{dists})
    \end{subfigure}
    \begin{subfigure}{\textwidth}
        \includegraphics[width=\textwidth]{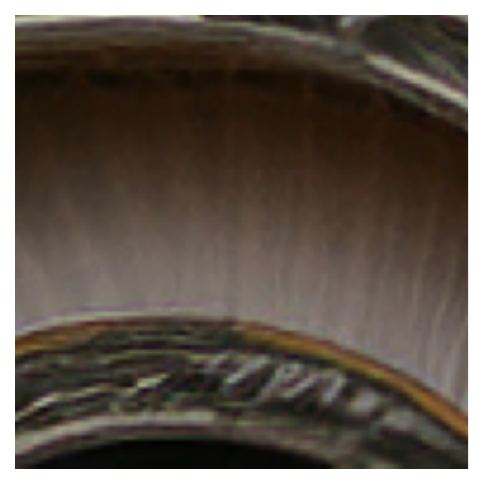} \\ \small WGSR (Ours) \\(25.65 / 0.214)
    \end{subfigure}
        \begin{subfigure}{\textwidth}
        \includegraphics[width=\textwidth]{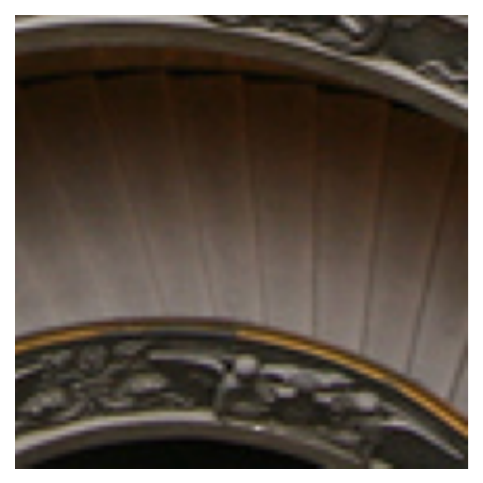} \\ \small HR (img-51)\\ (PSNR$\uparrow$ / DISTS$\downarrow$\cite{dists})
    \end{subfigure}
    \begin{subfigure}{\textwidth}
        \includegraphics[width=\textwidth]{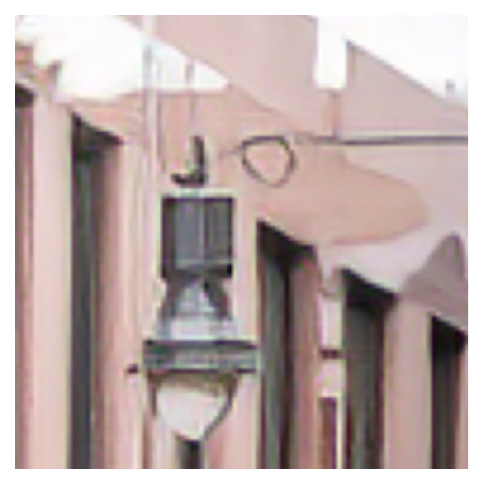} \\ \small WGSR (Ours) \\ (22.67 / 0.147)
    \end{subfigure}
        \begin{subfigure}{\textwidth}
        \includegraphics[width=\textwidth]{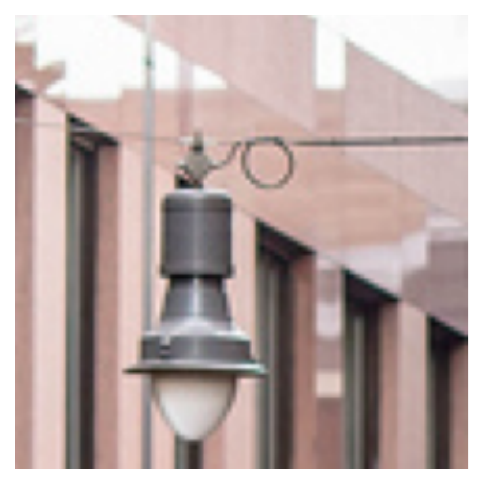} \\ \small HR (img-64)\\ (PSNR$\uparrow$ / DISTS$\downarrow$\cite{dists})
    \end{subfigure}
\end{subfigure} 
\caption{Visual comparison of the proposed wavelet-guided perceptual optimization method with the state-of-the-art for $\times$4 SR on natural images from Urban100 validation set \cite{urban100_cite}.}
\label{fig:supp_urban1} 
\end{figure*}

\begin{figure*}
\centering
\begin{subfigure}{0.16\textwidth}
     \begin{subfigure}{\textwidth}
        \includegraphics[width=\textwidth]{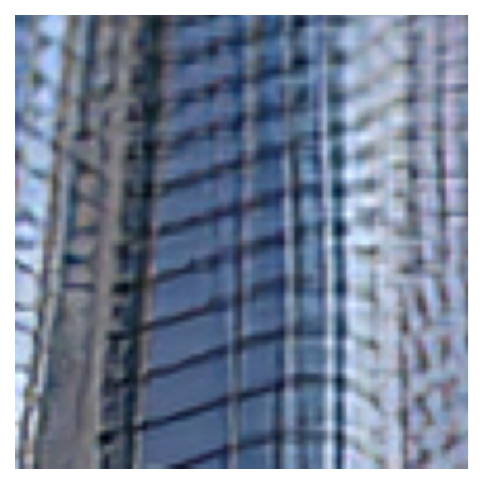} \\ \small ESRGAN-FS \cite{freq_sep} \\ (18.36 / 0.283)
    \end{subfigure}
    \begin{subfigure}{\textwidth}
        \includegraphics[width=\textwidth]{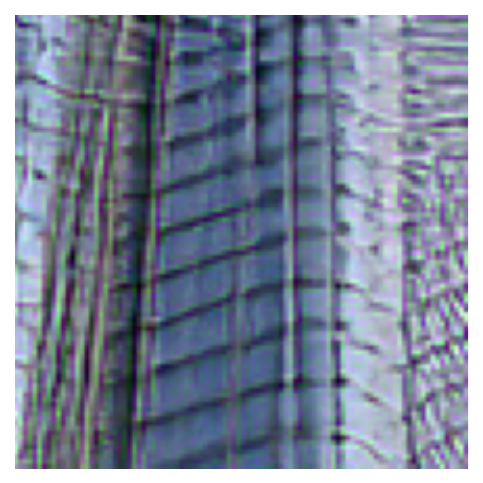} \\ \small ESRGAN+ \cite{esrganplus} \\ (17.85 / 0.258)
    \end{subfigure}
     \begin{subfigure}{\textwidth}
        \includegraphics[width=\textwidth]{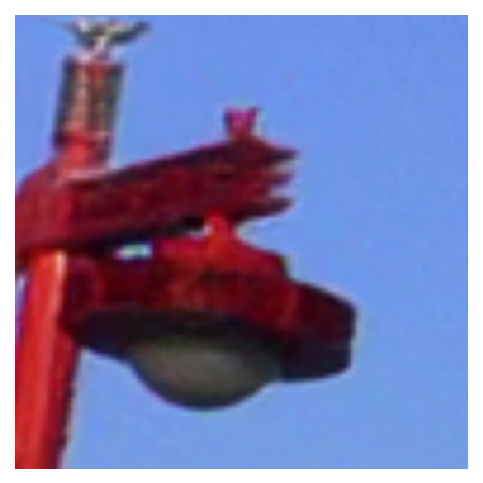} \\ \small ESRGAN-FS \cite{freq_sep} \\ (30.22 / 0.144)
    \end{subfigure}
    \begin{subfigure}{\textwidth}
        \includegraphics[width=\textwidth]{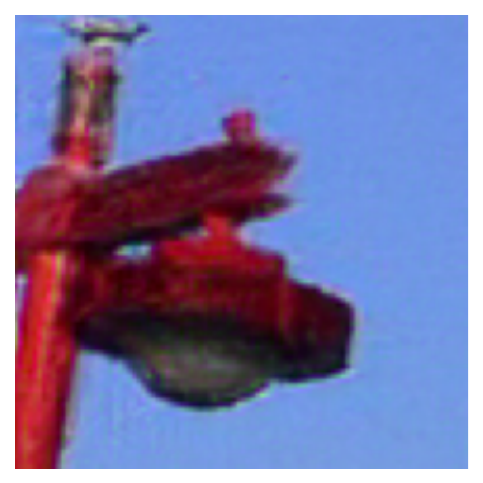} \\ \small ESRGAN+ \cite{esrganplus} \\ (28.22 / 0.170)
    \end{subfigure}
     \begin{subfigure}{\textwidth}
        \includegraphics[width=\textwidth]{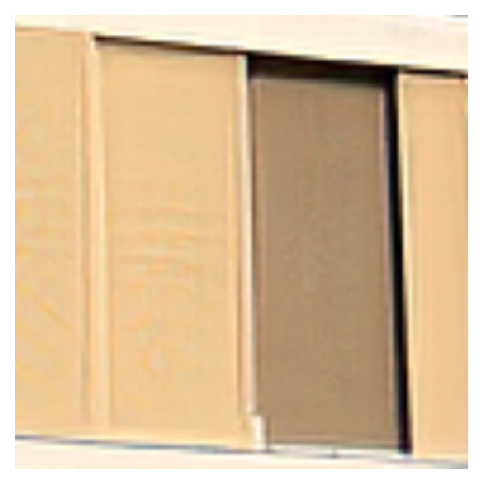} \\ \small ESRGAN-FS \cite{freq_sep} \\ (29.72 / 0.111)
    \end{subfigure}
    \begin{subfigure}{\textwidth}
        \includegraphics[width=\textwidth]{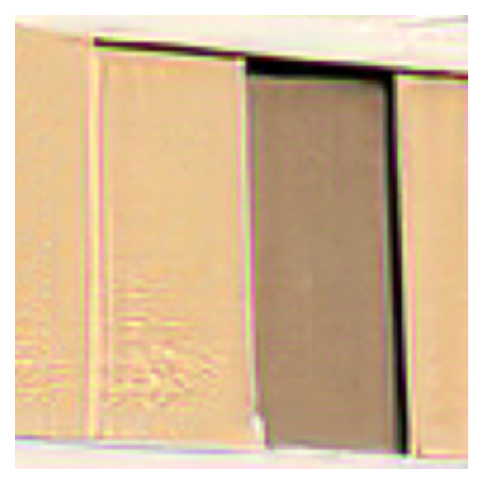} \\ \small ESRGAN+ \cite{esrganplus} \\ (26.59 / 0.161)
    \end{subfigure}
\end{subfigure}
\begin{subfigure}{0.16\textwidth}
    \begin{subfigure}{\textwidth}
        \includegraphics[width=\textwidth]{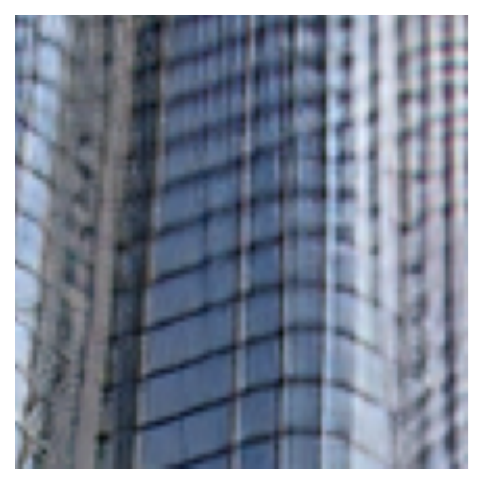} \\ \small SPSR \cite{ma_SPSR} \\(19.31 / 0.278)
    \end{subfigure}
    \begin{subfigure}{\textwidth}
        \includegraphics[width=\textwidth]{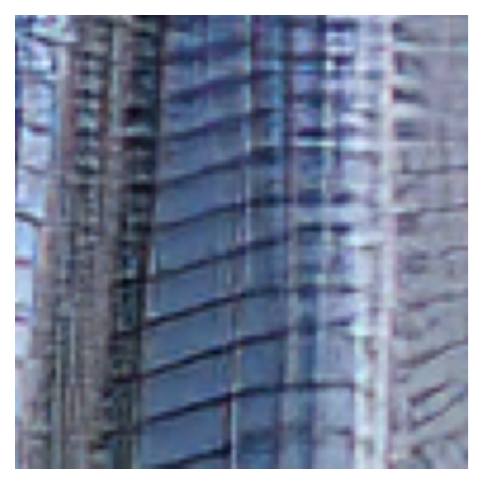} \\ \small RankSRGAN \cite{zhang2021ranksrgan} \\ (18.81 / 0.294)
    \end{subfigure}
    \begin{subfigure}{\textwidth}
        \includegraphics[width=\textwidth]{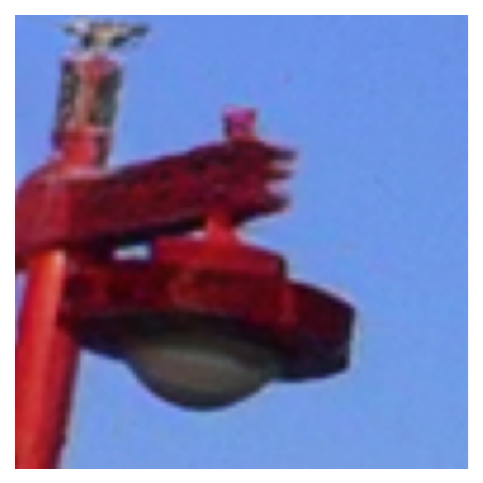} \\ \small SPSR \cite{ma_SPSR} \\ (29.98 / 0.145)
    \end{subfigure}
    \begin{subfigure}{\textwidth}
        \includegraphics[width=\textwidth]{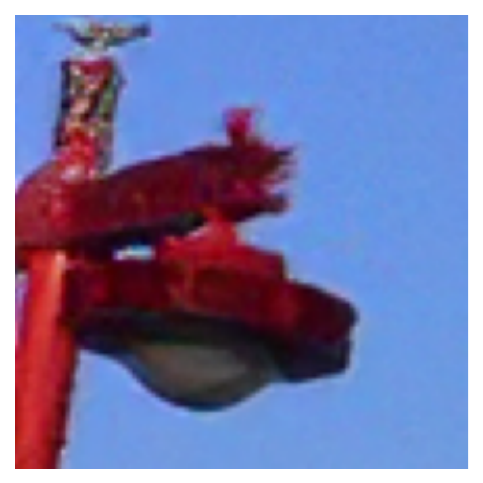} \\ \small RankSRGAN \cite{zhang2021ranksrgan} \\ (28.16 / 0.170)
    \end{subfigure}
    \begin{subfigure}{\textwidth}
        \includegraphics[width=\textwidth]{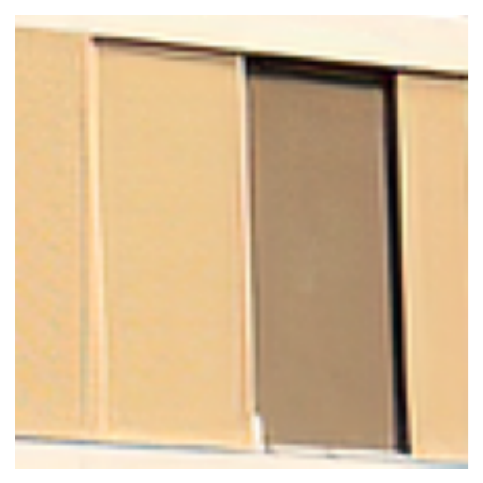} \\ \small SPSR \cite{ma_SPSR} \\ (29.66 / 0.109)
    \end{subfigure}
    \begin{subfigure}{\textwidth}
        \includegraphics[width=\textwidth]{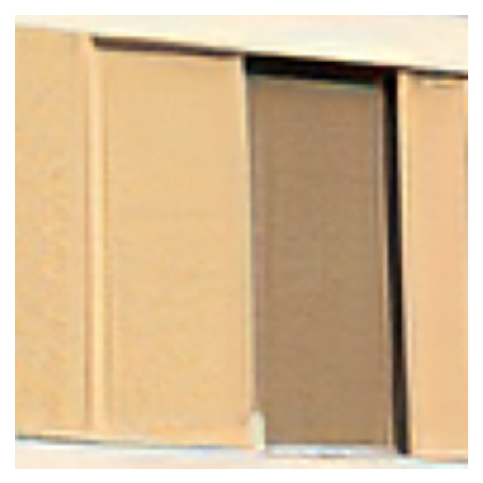} \\ \small RankSRGAN \cite{zhang2021ranksrgan} \\ (27.75 / 0.127)
    \end{subfigure}
\end{subfigure}
\begin{subfigure}{0.16\textwidth}
    \begin{subfigure}{\textwidth}
        \includegraphics[width=\textwidth]{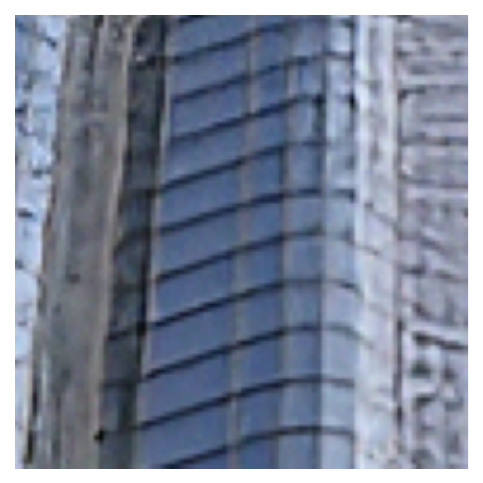} \\\small  SRFlow-DA \cite{jo2021srflowda} \\ (19.92 / 0.258)
    \end{subfigure}
    \begin{subfigure}{\textwidth}
        \includegraphics[width=\textwidth]{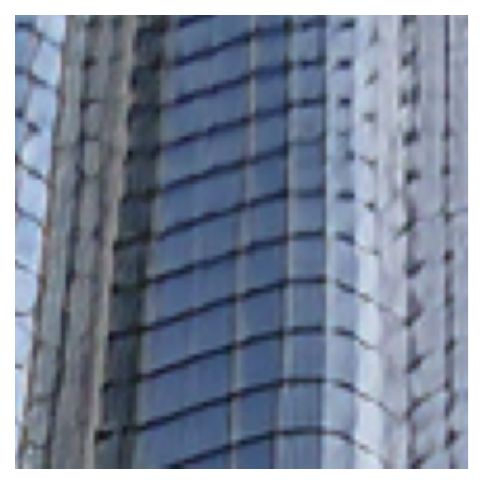} \\ \small LDL \cite{details_or_artifacts} \\ (20.06 / 0.245)
    \end{subfigure}
    \begin{subfigure}{\textwidth}
        \includegraphics[width=\textwidth]{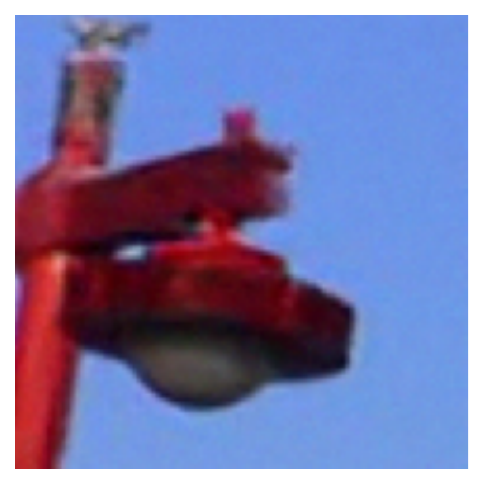} \\\small  SRFlow-DA \cite{jo2021srflowda} \\ (29.57 / 0.171)
    \end{subfigure}
    \begin{subfigure}{\textwidth}
        \includegraphics[width=\textwidth]{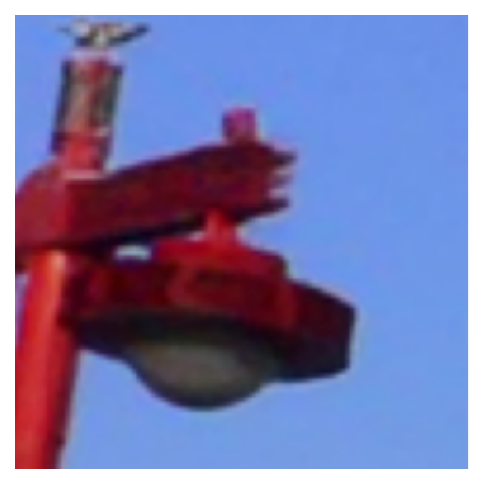} \\ \small LDL \cite{details_or_artifacts} \\ (30.70 / 0.147)
    \end{subfigure}
    \begin{subfigure}{\textwidth}
        \includegraphics[width=\textwidth]{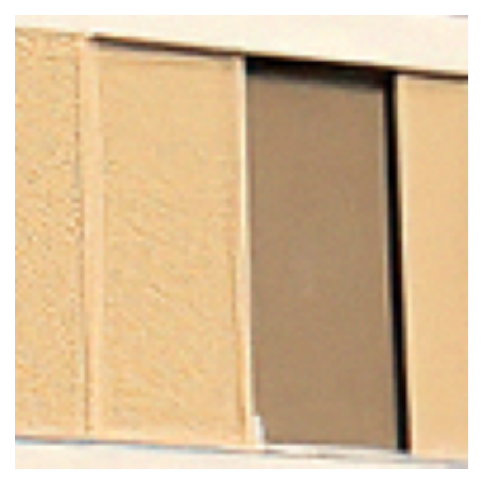} \\\small  SRFlow-DA \cite{jo2021srflowda} \\ (30.38 / 0.146)
    \end{subfigure}
    \begin{subfigure}{\textwidth}
        \includegraphics[width=\textwidth]{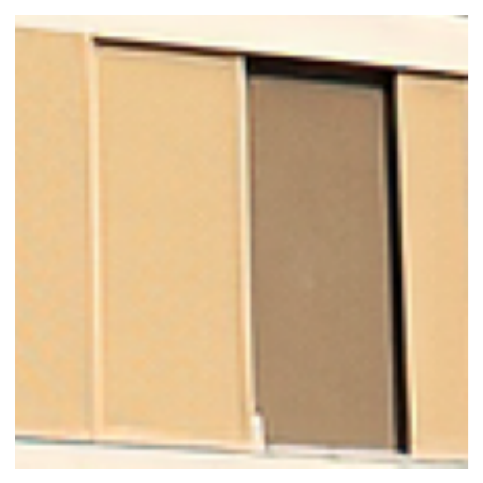} \\ \small LDL \cite{details_or_artifacts} \\ (30.61 / 0.109)
    \end{subfigure}
\end{subfigure}
\begin{subfigure}{0.16\textwidth}
    \begin{subfigure}{\textwidth}
        \includegraphics[width=\textwidth]{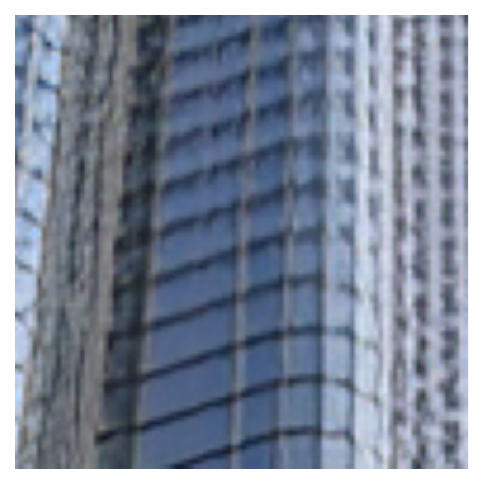} \\ \small FxSR \cite{fxsr} \\ (19.44 / 0.251)
    \end{subfigure}
            \begin{subfigure}{\textwidth}
        \includegraphics[width=\textwidth]{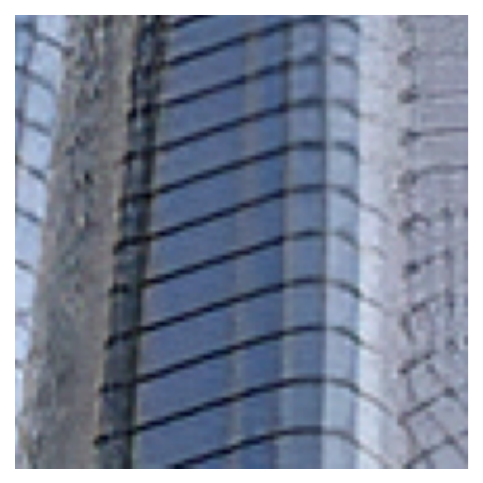} \\ \small PDASR \cite{PDASR} \\ (21.08 / 0.219)
    \end{subfigure}
    \begin{subfigure}{\textwidth}
        \includegraphics[width=\textwidth]{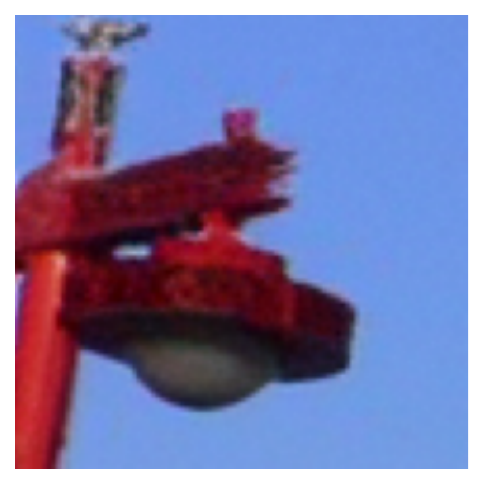} \\ \small FxSR \cite{fxsr} \\ (29.99 / 0.155)
    \end{subfigure}
            \begin{subfigure}{\textwidth}
        \includegraphics[width=\textwidth]{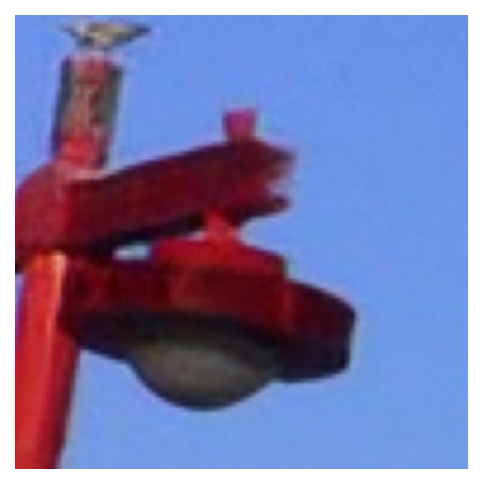} \\ \small PDASR \cite{PDASR} \\ (30.28 / 0.142)
    \end{subfigure}
    \begin{subfigure}{\textwidth}
        \includegraphics[width=\textwidth]{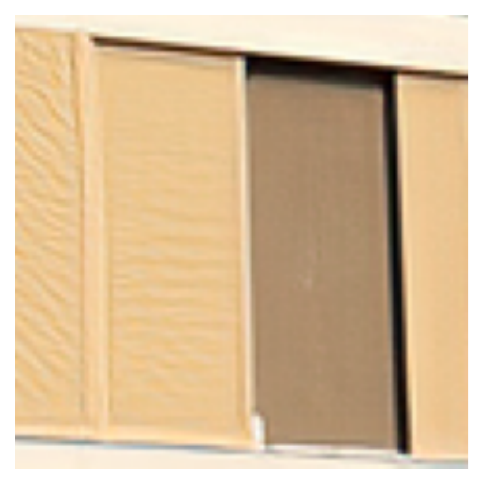} \\ \small FxSR \cite{fxsr} \\ (31.52 / 0.106)
    \end{subfigure}
            \begin{subfigure}{\textwidth}
        \includegraphics[width=\textwidth]{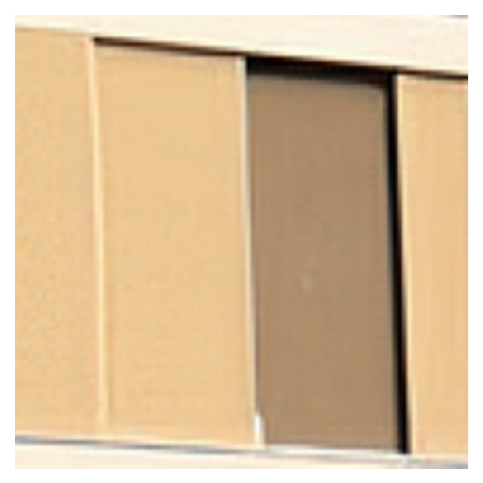} \\ \small PDASR \cite{PDASR} \\ (31.10 / 0.094)
    \end{subfigure}
\end{subfigure}
\begin{subfigure}{0.16\textwidth}
    \begin{subfigure}{\textwidth}
        \includegraphics[width=\textwidth]{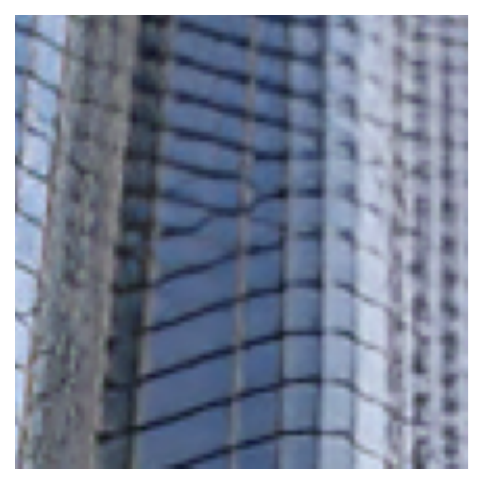} \\ \small SROOE \cite{srooe_Park_2023_CVPR} \\ (19.94 / 0.256)
    \end{subfigure}
    \begin{subfigure}{\textwidth}
        \includegraphics[width=\textwidth]{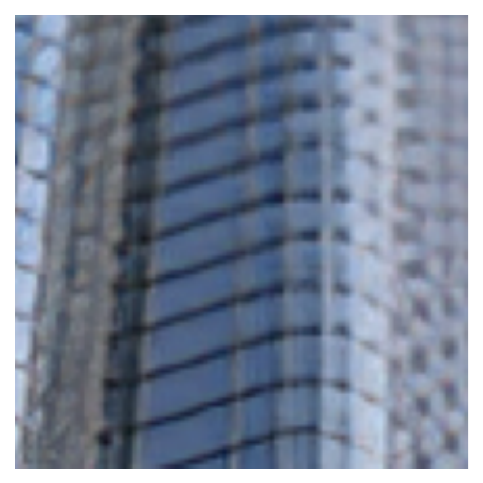} \\ \small  DualFormer \cite{dualformer_luo2023effectiveness} \\ (20.66 / 0.251)
    \end{subfigure}
    \begin{subfigure}{\textwidth}
        \includegraphics[width=\textwidth]{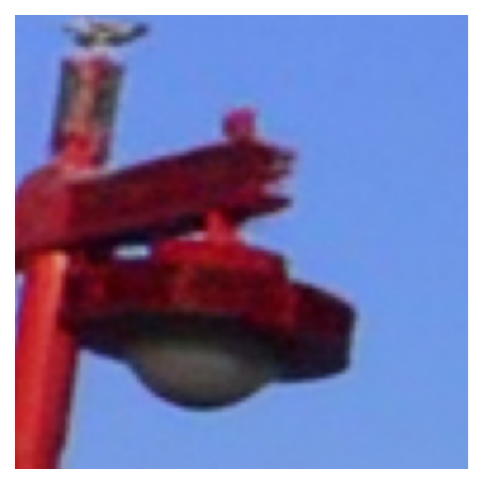} \\ \small SROOE \cite{srooe_Park_2023_CVPR} \\ (30.43 / 0.145)
    \end{subfigure}
    \begin{subfigure}{\textwidth}
        \includegraphics[width=\textwidth]{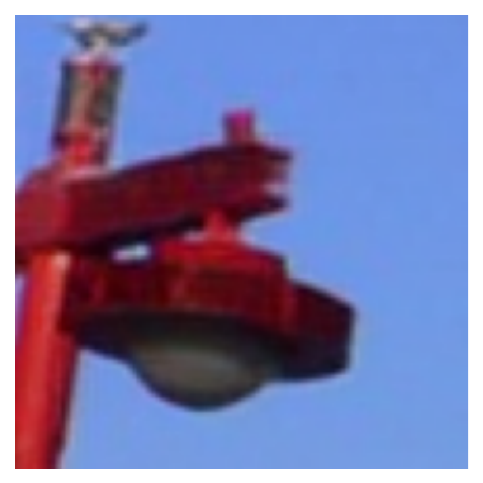} \\ \small  DualFormer \cite{dualformer_luo2023effectiveness} \\ (30.58 / 0.142)
    \end{subfigure}
    \begin{subfigure}{\textwidth}
        \includegraphics[width=\textwidth]{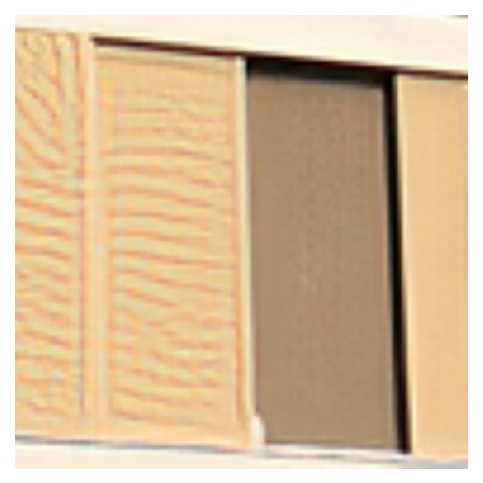} \\ \small SROOE \cite{srooe_Park_2023_CVPR} \\ (29.96 / 0.141)
    \end{subfigure}
    \begin{subfigure}{\textwidth}
        \includegraphics[width=\textwidth]{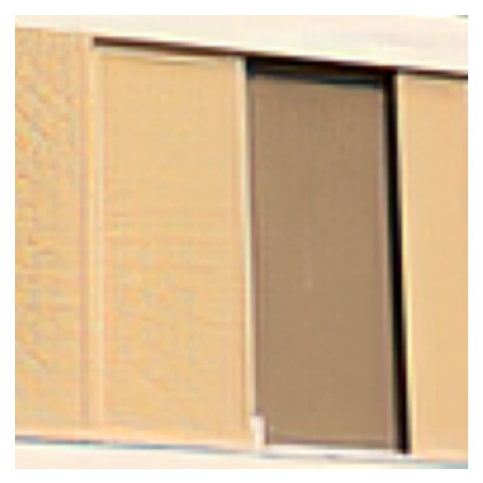} \\ \small  DualFormer \cite{dualformer_luo2023effectiveness} \\ (30.26 / 0.122)
    \end{subfigure}
\end{subfigure}
\begin{subfigure}{0.16\textwidth}
    \begin{subfigure}{\textwidth}
        \includegraphics[width=\textwidth]{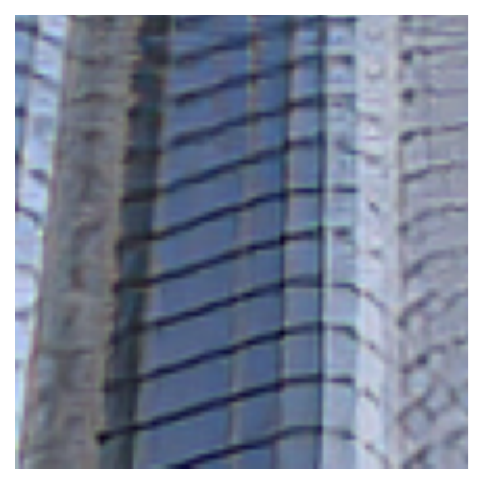} \\ \small WGSR (Ours) \\ (20.98 / 0.252)
    \end{subfigure}
        \begin{subfigure}{\textwidth}
        \includegraphics[width=\textwidth]{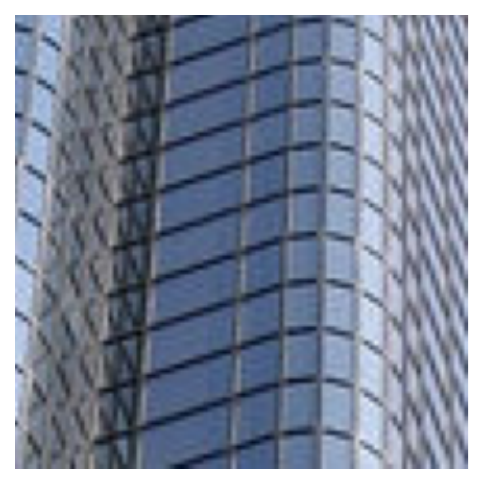} \\ \small HR (img-74)\\ (PSNR$\uparrow$ / DISTS$\downarrow$\cite{dists})
    \end{subfigure}
    \begin{subfigure}{\textwidth}
        \includegraphics[width=\textwidth]{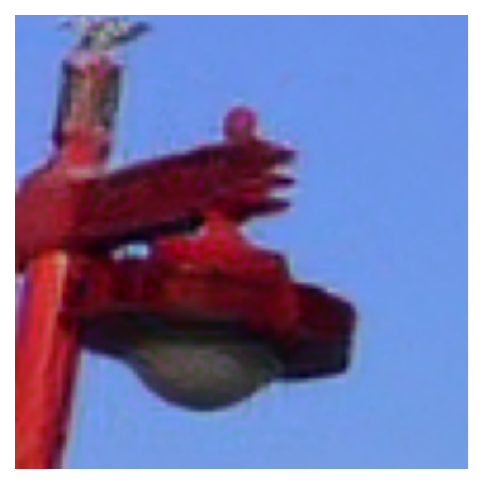} \\ \small WGSR (Ours) \\(30.04 / 0.162)
    \end{subfigure}
        \begin{subfigure}{\textwidth}
        \includegraphics[width=\textwidth]{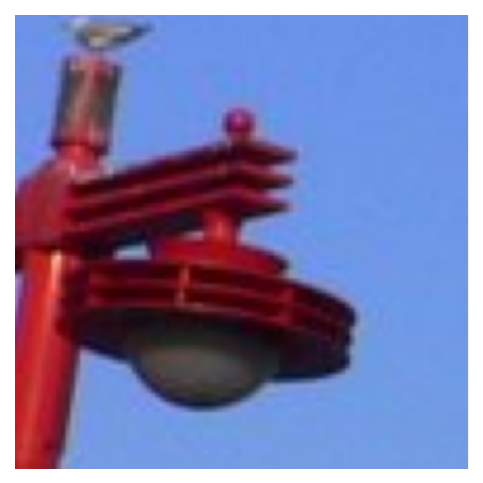} \\ \small HR (img-86)\\ (PSNR$\uparrow$ / DISTS$\downarrow$\cite{dists})
    \end{subfigure}
    \begin{subfigure}{\textwidth}
        \includegraphics[width=\textwidth]{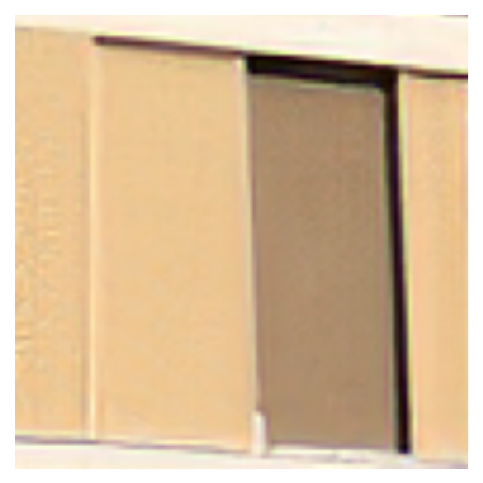} \\ \small WGSR (Ours) \\ (30.83 / 0.124)
    \end{subfigure}
        \begin{subfigure}{\textwidth}
        \includegraphics[width=\textwidth]{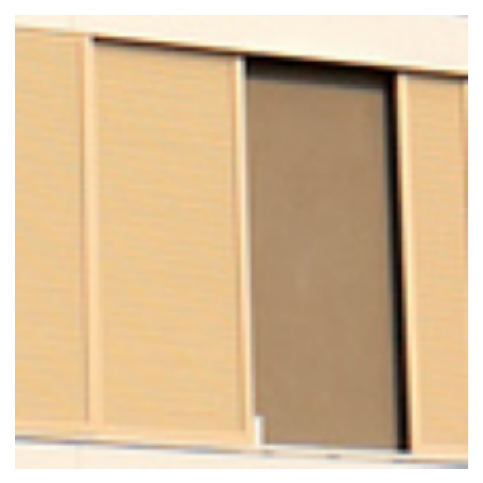} \\ \small HR (img-87)\\ (PSNR$\uparrow$ / DISTS$\downarrow$\cite{dists})
    \end{subfigure}
\end{subfigure} 
\caption{Visual comparison of the proposed wavelet-guided perceptual optimization method with the state-of-the-art for $\times$4 SR on natural images from Urban100 validation set \cite{urban100_cite}.}
\label{fig:supp_urban2} 
\end{figure*}

% \section{Rationale}
% \label{sec:rationale}
% % 
% Having the supplementary compiled together with the main paper means that:
% % 
% \begin{itemize}
% \item The supplementary can back-reference sections of the main paper, for example, we can refer to \cref{sec:intro};
% \item The main paper can forward reference sub-sections within the supplementary explicitly (e.g. referring to a particular experiment); 
% \item When submitted to arXiv, the supplementary will already included at the end of the paper.
% \end{itemize}
% % 
% To split the supplementary pages from the main paper, you can use \href{https://support.apple.com/en-ca/guide/preview/prvw11793/mac#:~:text=Delete%20a%20page%20from%20a,or%20choose%20Edit%20%3E%20Delete).}{Preview (on macOS)}, \href{https://www.adobe.com/acrobat/how-to/delete-pages-from-pdf.html#:~:text=Choose%20%E2%80%9CTools%E2%80%9D%20%3E%20%E2%80%9COrganize,or%20pages%20from%20the%20file.}{Adobe Acrobat} (on all OSs), as well as \href{https://superuser.com/questions/517986/is-it-possible-to-delete-some-pages-of-a-pdf-document}{command line tools}.

\begin{figure*}
\centering
\begin{subfigure}{0.24\textwidth}
     \begin{subfigure}{\textwidth}
        \includegraphics[width=\textwidth]{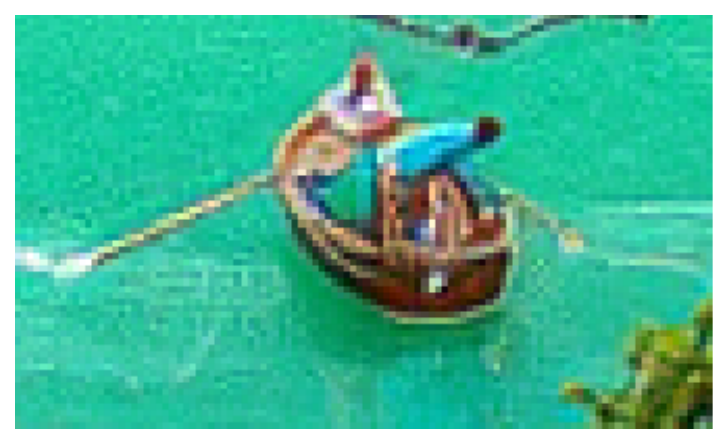} \\ \small bior2.6 \\ (21.22 / 0.180)
    \end{subfigure}
    \begin{subfigure}{\textwidth}
        \includegraphics[width=\textwidth]{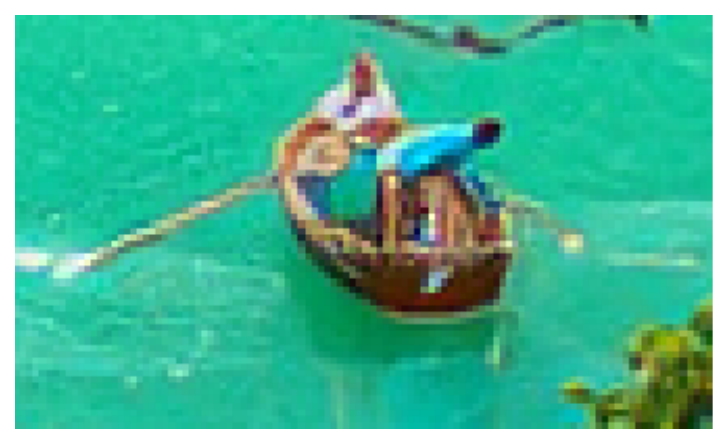} \\ \small bior4.4 \\ (21.68 / 0.168)
    \end{subfigure}
     \begin{subfigure}{\textwidth}
        \includegraphics[width=\textwidth]{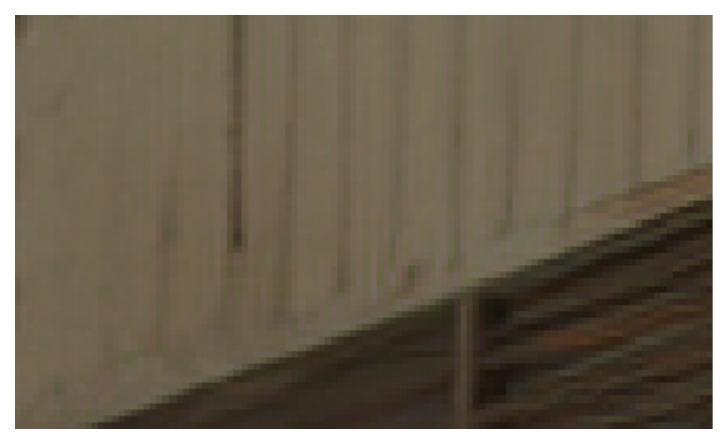} \\ \small bior2.6 \\ (34.38 / 0.124)
    \end{subfigure}
    \begin{subfigure}{\textwidth}
        \includegraphics[width=\textwidth]{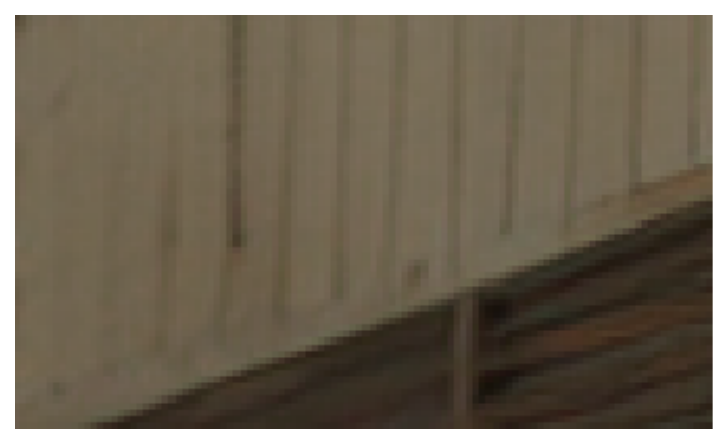} \\ \small bior4.4 \\ (33.97 / 0.130)
    \end{subfigure}
     \begin{subfigure}{\textwidth}
        \includegraphics[width=\textwidth]{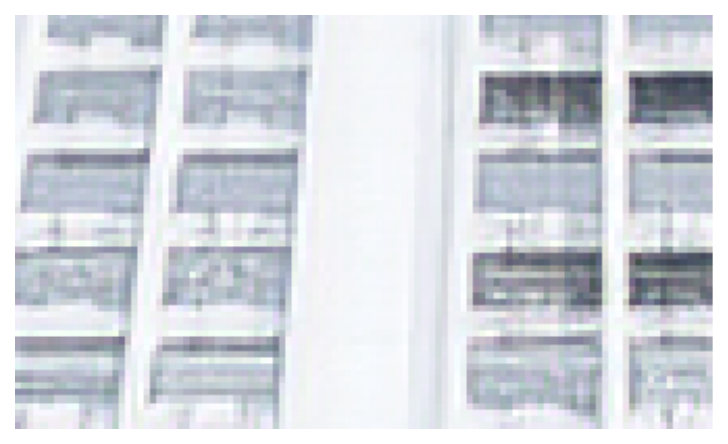} \\ \small bior2.6 \\ (18.49 / 0.191)
    \end{subfigure}
    \begin{subfigure}{\textwidth}
        \includegraphics[width=\textwidth]{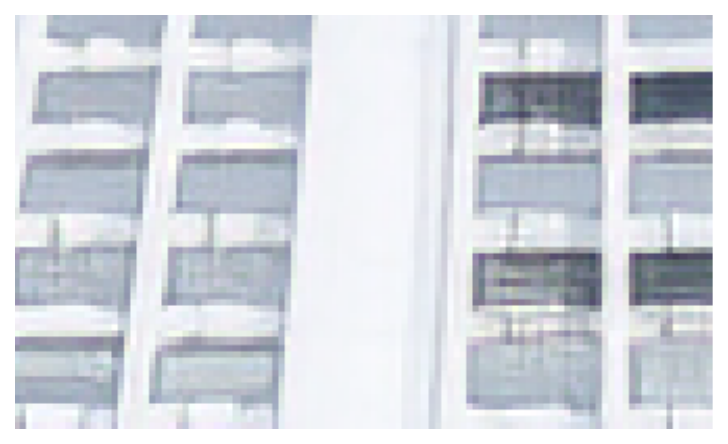} \\ \small bior4.4 \\ (18.49 / 0.193)
    \end{subfigure}
\end{subfigure}
\vspace{14pt}
\begin{subfigure}{0.24\textwidth}
    \begin{subfigure}{\textwidth}
        \includegraphics[width=\textwidth]{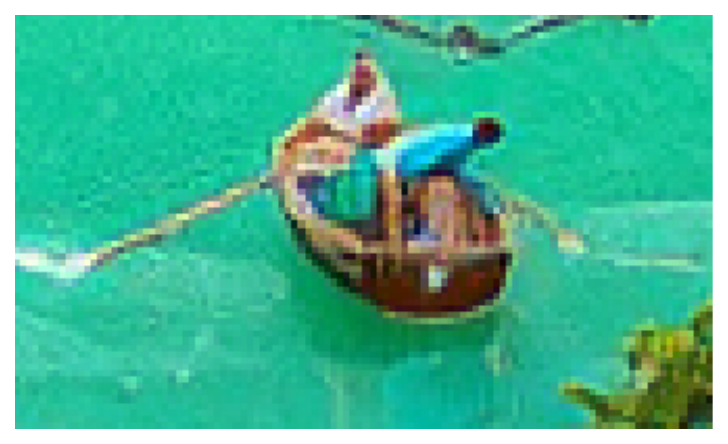} \\ \small db7 \\(21.46 / 0.168)
    \end{subfigure}
    \begin{subfigure}{\textwidth}
        \includegraphics[width=\textwidth]{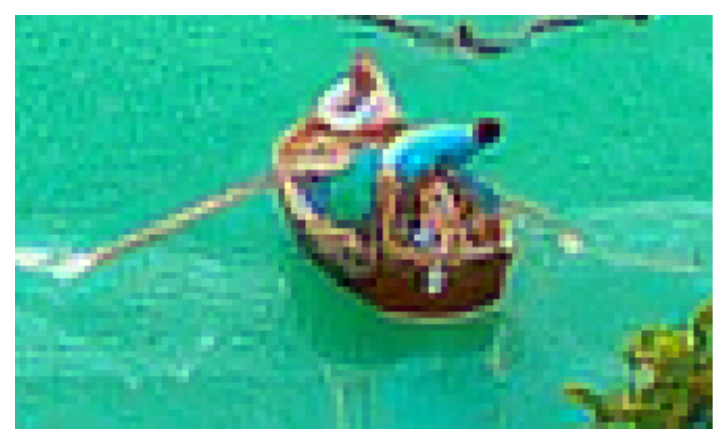} \\ \small db19  \\ (21.21 / 0.177)
    \end{subfigure}
    \begin{subfigure}{\textwidth}
        \includegraphics[width=\textwidth]{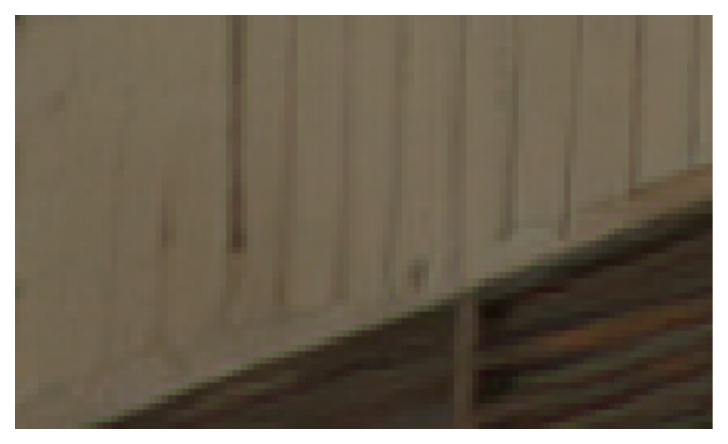} \\ \small db7  \\ (33.36 / 0.122)
    \end{subfigure}
    \begin{subfigure}{\textwidth}
        \includegraphics[width=\textwidth]{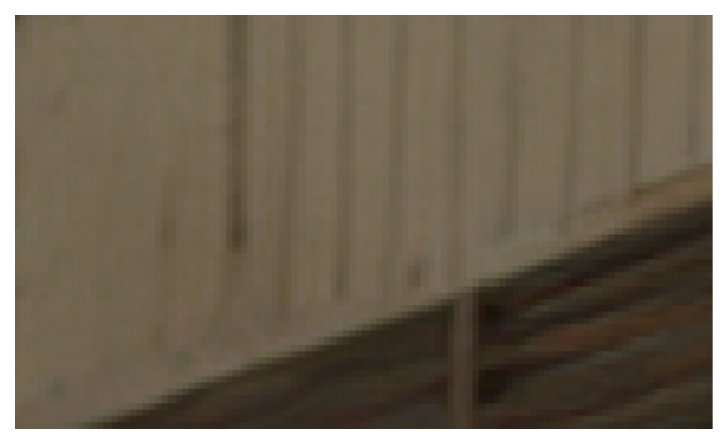} \\ \small db19  \\ (34.27 / 0.146)
    \end{subfigure}
    \begin{subfigure}{\textwidth}
        \includegraphics[width=\textwidth]{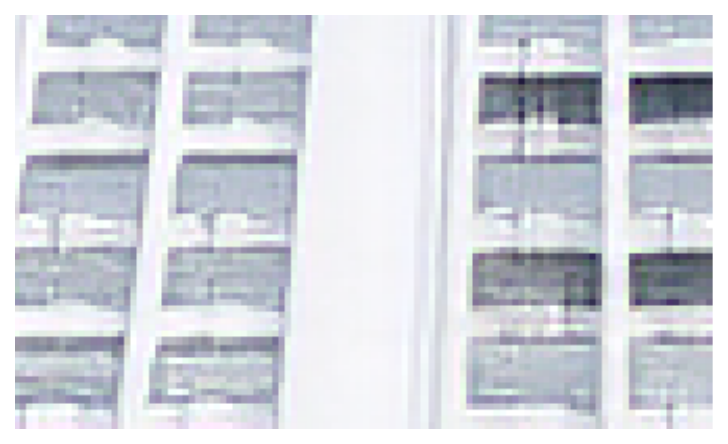} \\ \small db7  \\ (18.34 / 0.183)
    \end{subfigure}
    \begin{subfigure}{\textwidth}
        \includegraphics[width=\textwidth]{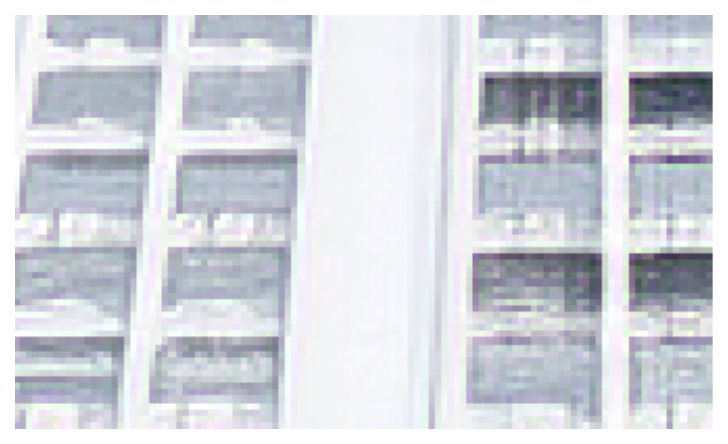} \\ \small db19  \\ (18.53 / 0.201)
    \end{subfigure}
\end{subfigure}
\begin{subfigure}{0.24\textwidth}
    \begin{subfigure}{\textwidth}
        \includegraphics[width=\textwidth]{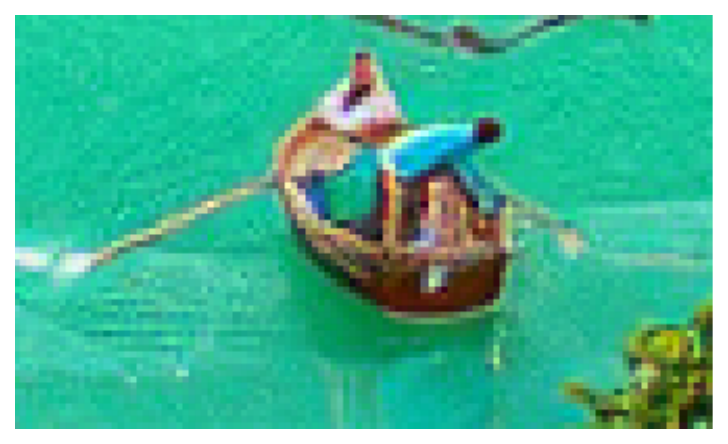} \\\small  haar \\ (21.23 / 0.164)
    \end{subfigure}
    \begin{subfigure}{\textwidth}
        \includegraphics[width=\textwidth]{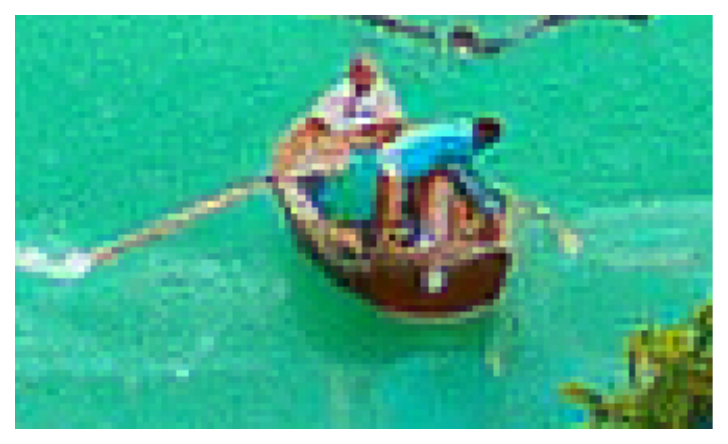} \\ \small sym19 \\ (21.05 / 0.171)
    \end{subfigure}
    \begin{subfigure}{\textwidth}
        \includegraphics[width=\textwidth]{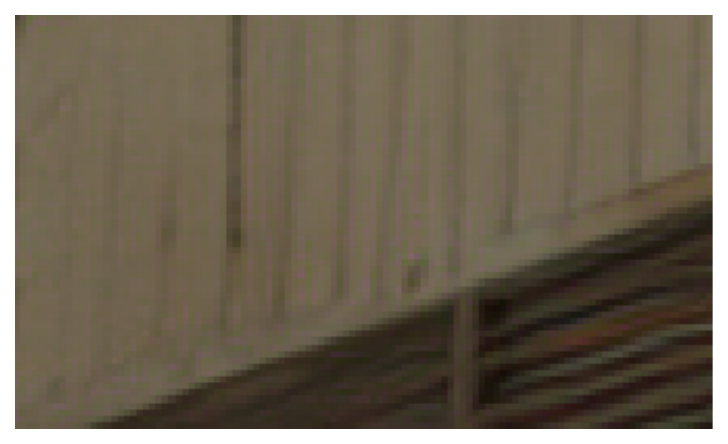} \\\small  haar \\ (34.58 / 0.111)
    \end{subfigure}
    \begin{subfigure}{\textwidth}
        \includegraphics[width=\textwidth]{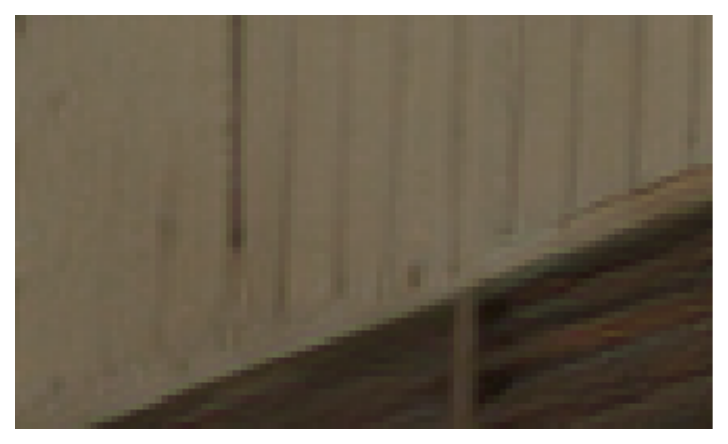} \\ \small sym19 \\ (34.11 / 0.129)
    \end{subfigure}
    \begin{subfigure}{\textwidth}
        \includegraphics[width=\textwidth]{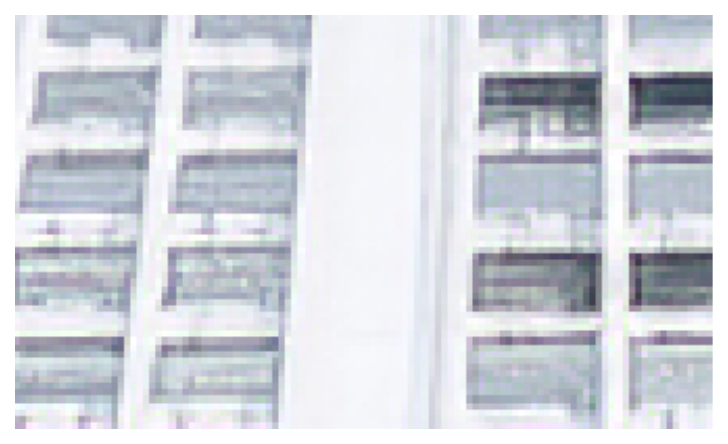} \\\small  haar \\ (18.36 / 0.186)
    \end{subfigure}
    \begin{subfigure}{\textwidth}
        \includegraphics[width=\textwidth]{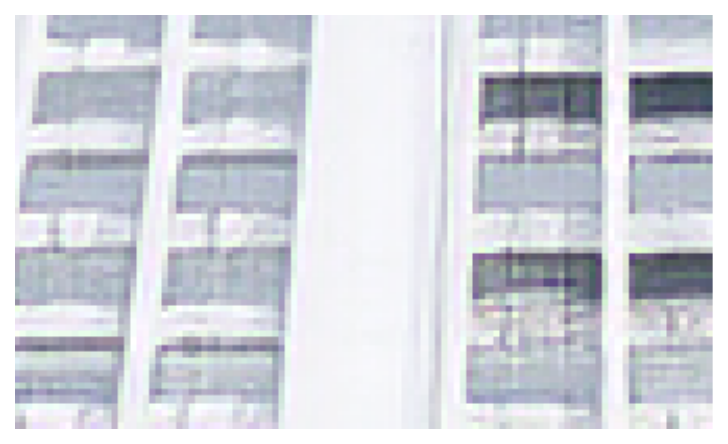} \\ \small sym19 \\ (18.34 / 0.200)
    \end{subfigure}
\end{subfigure}
\begin{subfigure}{0.24\textwidth}
    \begin{subfigure}{\textwidth}
        \includegraphics[width=\textwidth]{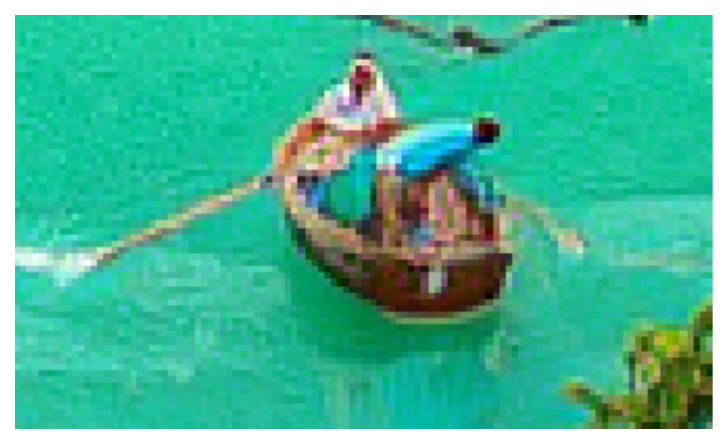} \\ \small sym7 (WGSR) \\ (21.62 / 0.155)
    \end{subfigure}
            \begin{subfigure}{\textwidth}
        \includegraphics[width=\textwidth]{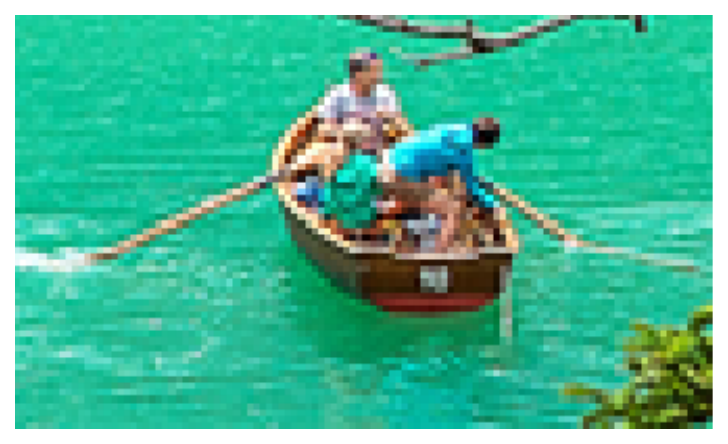} \\ \small HR (img-807) \\ (PSNR$\uparrow$ / DISTS$\downarrow$ \cite{dists})
    \end{subfigure}
    \begin{subfigure}{\textwidth}
        \includegraphics[width=\textwidth]{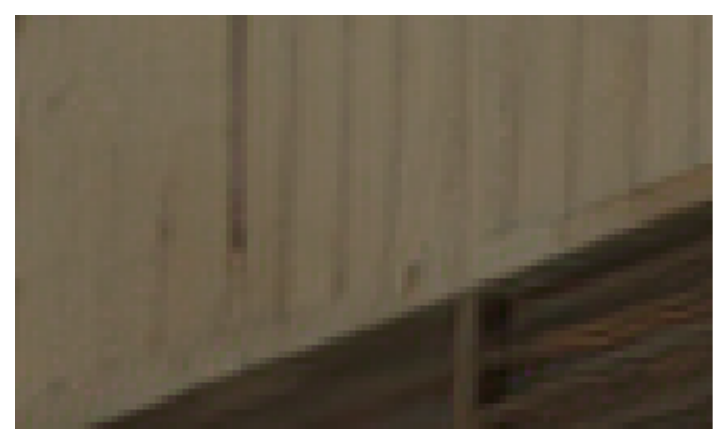} \\ \small sym7 (WGSR) \\ (34.37 / 0.119)
    \end{subfigure}
            \begin{subfigure}{\textwidth}
        \includegraphics[width=\textwidth]{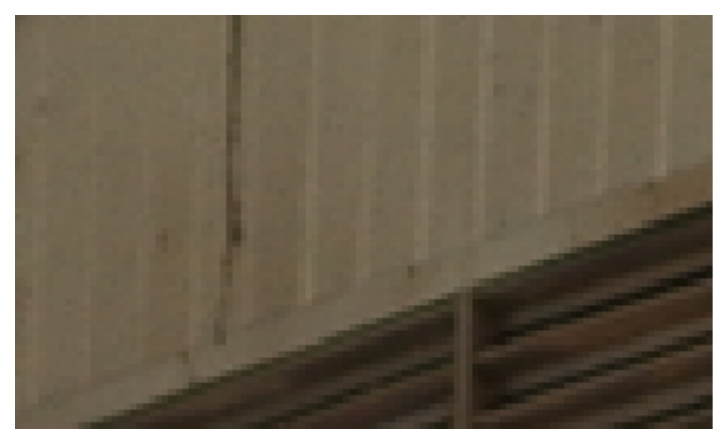} \\ \small HR (img-831) \\ (PSNR$\uparrow$ / DISTS$\downarrow$ \cite{dists})
    \end{subfigure}
    \begin{subfigure}{\textwidth}
        \includegraphics[width=\textwidth]{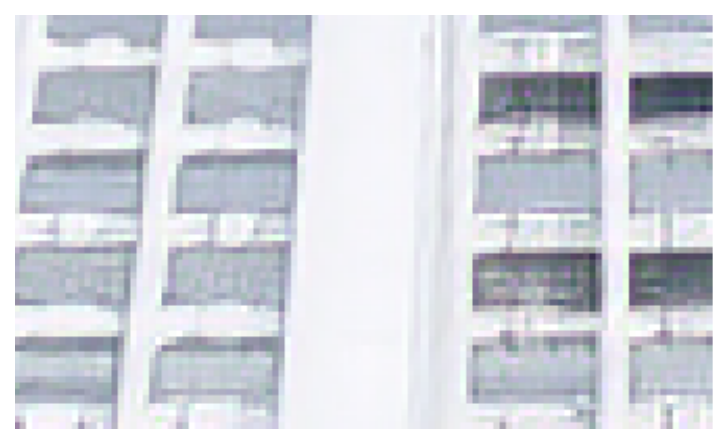} \\ \small sym7 (WGSR) \\ (18.44 / 0.212)
    \end{subfigure}
            \begin{subfigure}{\textwidth}
        \includegraphics[width=\textwidth]{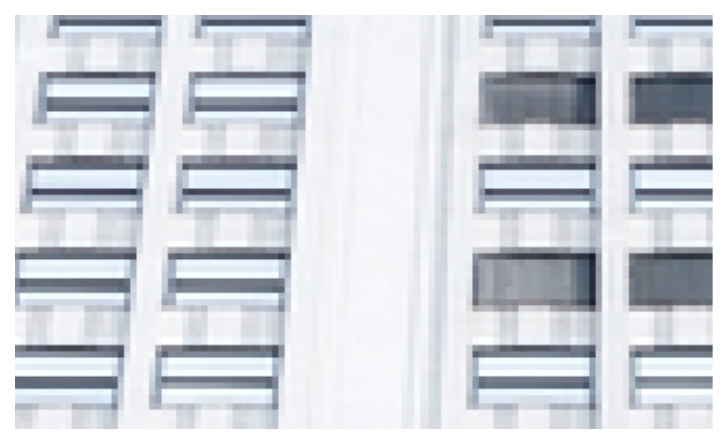} \\ \small HR (img-846) \\ (PSNR$\uparrow$ / DISTS$\downarrow$ \cite{dists})
    \end{subfigure}
\end{subfigure} 
\caption{Visual comparison of WGSR method with different wavelet families for 4$\times$ SR on DIV2K \cite{Agustsson_2017_CVPR_Workshops}.}
\label{fig:supp_wavelet_fam_visual} 
\end{figure*}
